# Supplementary material for: How rotational invariance of common kernels prevents generalization in high dimensions
Source: arXiv:2104.04244 source file (2021-04-09)
Supplement: Supplementary file 1 [file Appendix_Corollaries.tex]

\section{Proofs of Corollaries}
\mw{\begin{itemize}
    \item what is the corollary in the section E.1.
    \item what is p? should it be q? Maybe define a macro?
\end{itemize}}
\makepurple{
\begin{cor}
\label{cr:EVlowerbound}
Assume that for any $j$, $g_j$ is a positive definite function. In addition, assume that there exist $j \geq p+1$ such that $g_j(1,1) > 0$. Then, there exists some positive non zero constant $c_{\lambda_{min}}$ such that
\begin{equation}
\label{eq:lambdamin}
    \lambda_{min}(K) \geq c_{\lambda_{min}} >0 ~~~a.s.
\end{equation}
\end{cor}
}

\subsection{Proof of Corollary \ref{cr:poly}}
\begin{proof}
The corollary follows straight forwardly form the proof of Theorem \ref{th:main_text} when replacing $\fstarz(\Z)$ with $y$ in Equation \ref{eq:thmainpoly}. Note that this is only possible if $y$ has bounded entries. Hence, we can conclude the proof. 
\end{proof}

\subsection{Proof of Corollary \ref{cr:EVlowerbound}}
\begin{proof}
We make use of the same notation as in the proof of Proposition \ref{prop:elkarouiextension}. Let $\tilde{M}$ be the matrix with entries
\begin{align}
    \tilde{M}_{i,j} :=  
    \sum_{m =0}^{p}(\z_i^T\z_j)^{m} \sum_{ \makepurple{l_1+l_2  \geq p+1-m}} \frac{ g_{m}^{(l_1,l_2)}(\eta^{m,i,j}_{l_1,l_2})}{l_1
    ! l_2!} (\z_i^T\z_i -1 )^{l_1} (\z_j^T\z_j -1 )^{l_2}   ~~ a.s.
\end{align}
where $\eta^{m,i,j}_{l_1,l_2}\in \mathbb{R}$ are chosen such that 
\begin{align*}
    K_{i,j} &= \tilde{M}_{i,j} + \sum_{m =0}^p (\z_i^T\z_j)^{m} \sum_{ l_1+l_2 \leq p-m} \frac{ g_{m}^{(l_1,l_2)}(1,1)}{l_1
    ! l_2!} (\z_i^T\z_i -1 )^{l_1} (\z_j^T\z_j -1 )^{l_2}   \\ 
    &+ (\z_i^T\z_j)^{p+1} \sum_{m =p+1}^{\infty}  (\z_i^T\z_j)^{m-(p+1)} g_{m}(\lvert\lvert \z_i\rvert\rvert_2^2,\lvert\lvert \z_j\rvert\rvert_2^2)  ~~ a.s.
\end{align*}
In a first step, the goal is to show that $\lvert\lvert \tilde{M}\rvert\rvert_2^2 \to 0$. We already know form the proof of Proposition \ref{prop:elkarouiextension} that this is true for the off diagonal matrix of $\tilde{M}$. Hence, we only need to show that $\lvert\lvert D_{\tilde{M}}\rvert\rvert_2^2 \to 0$, where $D_{\tilde{M}}$ is the diagonal matrix of $\tilde{M}$. However, again using the same argumentation as in the proof of Proposition \ref{prop:elkarouiextension} and by the fact that $ l_1+l_2 \geq 1$, we can see that
\begin{equation}
    \sum_{m =0}^{p} \sum_{ \makepurple{l_1+l_2  \geq p+1-m}} \left|  \frac{ g_{m}^{(l_1,l_2)}(\eta^{m,i,j}_{l_1,l_2})}{l_1
    ! l_2!} (\z_i^T\z_i -1 )^{l_1+l_2} (\z_i^T\z_i)^{m} \right| \to 0
\end{equation}
from which the claim follows. Therefore, we have that 
\begin{equation}
    \lvert\lvert  K - (M + \tilde{M})\rvert\rvert_2^2 \to 0
\end{equation}
Next, note that we have
\begin{equation}
    M + \tilde{M} =  \textbf{I}_n\left(k(e_1,e_1)  - \sum_{i =0}^p g_i(1,1) \right) +  \sum_{i=0}^p (\textbf{X}^T\textbf{X})^{\circ i} \circ K_{g_i}
\end{equation}
with $K_{g_m}$ the matrix with entries $K_{g_m, i,j} = g_m(\lvert\lvert \z_i\rvert\rvert_2^2, \lvert\lvert \z_j\rvert\rvert_2^2)$, which is positive semi definite since $g_m$ is a positive definite function by assumption. Hence, by Schur's Product Theorem, we get that $ (\textbf{X}^T\textbf{X})^{\circ i} \circ K_{g_i}$ is positive semi definite, and therefore, 
\begin{equation}
    M + \tilde{M} \succeq \textbf{I}_n\left(k(e_1,e_1)  - \sum_{i =0}^p g_i(1,1) \right). 
\end{equation}
The proof then follows from the fact that $k(e_1,e_1) = \sum_{i =0}^{\infty} g_i(1,1) >\sum_{i =0}^p g_i(1,1) $, which holds true since by assumption $g_i \geq 0$ and there exists $j \geq p+1$ such that $g_j >0$.
\end{proof}
