# Supplementary material for: How rotational invariance of common kernels prevents generalization in high dimensions
Source: arXiv:2104.04244 source file (2021-04-09)
Supplement: Supplementary file 2 [file Appendix_RBF.tex]

\section{$\alpha$-Exponential Kernels}

\item[(A.1)] \textit{Kernel has a local power expansion}:
  Define the neighborhood $\convergeset{\delta}{\delta'} \subset \R^d \times \R^d$  as
  \begin{equation*}
    \convergeset{\delta}{\delta'} := \{(\xk,\xkd) \in  \R^d \times \R^d \mid (\|\xk\|_2^2, \|\xkd\|_2^2) \in [1-\delta, 1+\delta] \times
  [1-\delta, 1+\delta]\}.
  \end{equation*}
  
  A kernel $\kernf$ has a local power expansion if $\rotkerfunc$ can be expanded as a power series
  \begin{equation}
    \label{eq:kerneldefg}
    \kerfunc{\xk}{\xkd}= \rotkerfunc(\|\xk\|_2^2, \|\xkd\|_2^2, \xk^\top \xkd) = \sum_{j=0}^{\infty} \rotkerfunccoeffj{j}(\|\xk\|_2^2,\|\xkd\|_2^2) (\xk^\top \xkd)^j 
   \end{equation}
   that converges in a neighborhood $\convergeset{\delta,\delta'}$ of the sphere for some $\delta, \delta'>0$ and where $g_i$ \fy{don't need $g_i\geq 0$ anymore?} is
  $(\floor{2/\beta}+1-i)$-times continuously differentiable in an
  neighbourhood of $(1,1)$. In addition, we assume that there exists $\jthresh > \floor{2/\beta}$ such that $\rotkerfunc_{\jthresh}(1,1) >0$.
  %%   In  particular, there exists a power series as described in Equation
  %% \ref{eq:kerneldefg}, for which we can find $\delta>0,\delta'>0$ such
  %% that for any
  %% $(x,x') \in \RR^d \times \RR^d$, with
  %% $(||\xk||_2^2, ||\xkd||_2^2) \in [1-\delta, 1+\delta] \times
  %% [1-\delta, 1+\delta]$ and $\xk^\top \xkd \in [-\delta',\delta']$, the
  %% power series converges and equals $k(\xk,\xkd)$.  In particular, we
  %% assume that the function $g$ from Equation \ref{eq:kerneldefg} is
  %% continuous and for any $i \leq \floor{2/\beta}+1$, $g_i$ is
  %% $(\floor{2/\beta}+1-i)$-times continuously differentiable in an
  %% neighbourhood of $(1,1)$.
\item[(A.2)] \textit{Positive Definiteness:} All $g_i$ from Assumption A.1 are positive semidefinite kernels. \kd{I would state this as an extra assumption since it is quite different for A.1} \fy{so this covers NTK?}
\item[(A.3)] \textit{Restricted Lipschitz
  Continuity:} The restriction of $k$ on $\{(x,x)| x \in \R^d,
  \| x \|_2^2 \in [1-\delta_L, 1+\delta_L]\}$ is
  a Lipschitz continuous function for some constant $\delta_L>0$.

\begin{proof}[Proof of Lemma \ref{lm:alphaexp}]
For simplicity, we show that the result holds true for $\tau_0 = 1$. It is then not difficult to see that it holds also true for the more general case where $\tau_0 >0$ is some constant. In a first step, we note that we already know from Lemma \ref{lm:alphaexpbound} that the Eigenvalues of the matrix $D^{\alpha}$ are all bounded away from zero by some constant $c_{\alpha} >0$ independent of $n$. The goal of this proof is to make use of this fact in order to show the desired result. The proof is separated in several steps. In a first step, we construct a kernel positive definite kernel $\tilde{k}$ such that $\exp(-||X-X'||^{\alpha}) = \exp(\tilde{k}(X,X')) \exp(-||X-X'||^{\alpha} - \tilde{k}(X,X')) $ and $\exp(-||X-X'||^{\alpha} - \tilde{k}(X,X')) $ is a positive definite function. Then, we show that the Eigenvalues of the kernel matrix of $\exp(\tilde{k}(X,X'))$ are lower bounded and finally, in a last step, we show that this implies that the Eigenvalues of the kernel matrix of $\exp(-||X-X'||^{\alpha})$ are lower bounded. \\\\
\textbf{Step 1:}
Let $d_{\alpha} = ||X-X'||^{\alpha}$. We know from Chapter~3 Theorem~2.2
\cite{Berg84} that this is a conditionally negative definite function, i.e. for every $v \in \mathbb{R}^n$ with $1^T v = 0$, $v^T D^{\alpha}v \geq 0$. As shown in Chapter~3 Lemma~2.1 \cite{Berg84}, a kernel function $\phi(X,X')$ is conditionally negative definite, if and only if for any $X_0$, $ \phi(X,X_0) + \phi(X_0,X') -\phi(X,X') - \phi(X_0,X_0)$ is a positive definite function. Hence, we know that  $ d_{\alpha}(X,0) + d_{\alpha}(X_0,X') -d_{\alpha}(X,X') - d_{\alpha}(X_0,X_0)$ is positive definite. Let $A$ be the corresponding kernel matrix evaluated at $\textbf{X}$. It is shown in the proof of Chapter~3 Lemma~2.1 \cite{Berg84} that for any $v \in \mathbb{R}^n$,
$$ - v^T A v = \begin{pmatrix}v \\ - 1^Tv\end{pmatrix} \begin{pmatrix} D^{\alpha} & d_{\alpha}(X_0, \textbf{X}) \\ d_{\alpha}(X_0, \textbf{X})^T & d_{\alpha}(X_0,X_0) \end{pmatrix}\begin{pmatrix}v \\ - 1^Tv\end{pmatrix} \leq 0
$$
where $d_{\alpha}(X_0, \textbf{X})$ is the vector with entries $d_{\alpha}(X_0, \textbf{X})_i = d_{\alpha}(X_i,X_0)$. Note that inequality $\leq 0$ follows from the fact that $d_{\alpha}$ is conditionally negative definite and $1^T \begin{pmatrix}v \\ - 1^Tv\end{pmatrix} = 0$. The issue now is that even when the matrix $\begin{pmatrix} D^{\alpha} & d_{\alpha}(X_0, \textbf{X}) \\ d_{\alpha}(X_0, \textbf{X})^T & d_{\alpha}(X_0,X_0) \end{pmatrix}$ has Eigenvalues bounded away from zero, we can not conclude that this is also the case for $A$. The reason is because the vector $v = \frac{1}{\sqrt{n}} 1$ has $||v||_2 = 1$ but $1^T v = \sqrt{n}$. Thus, this would only imply that $- v^T A v \leq \frac{-c}{n}$. \\
The goal is now to construct a kernel function $\tilde{k}$ based on the same idea which, however, satisfies $- v^T A v \leq c$ for some constant $c>0$ and $A$ again the kernel matrix of $\tilde{k}$ evaluated at $\textbf{X}$. In a first step, note that we can extend the proof of Lemma \ref{lm:innerpr} to see that there exists almost surely with respect to the draws of $\textbf{X}$ a set of $n$ vectors $\tilde{\textbf{X}}$, such that for any two vectors $X,X' \in \textbf{X} \cup \tilde{\textbf{X}}$, we have that
\begin{equation}
\label{eq:tmpconineq}
    | X^TX' - \delta_{X = X'} | \leq n^{-\beta/2} \log(n)^{1+\epsilon} 
\end{equation}
Next, note that because $\textbf{X} \cup \tilde{\textbf{X}}$ are in total $2 n$ vectors, we can use the proof of Lemma \ref{lm:alphaexpbound} to the find there exists some constant $c_{\lambda} > 0$ independent of $n$ such that for any $v \in \mathbb{R}^{2n}$ with $||v||_21$ and $1^T v = 0$, 

$$v^T  \begin{pmatrix} D^{\alpha} & D^{\alpha}(\tilde{\textbf{X}}, \textbf{X}) \\ D^{\alpha}(\tilde{\textbf{X}}, \textbf{X})^T & \tilde{D}^{\alpha} \end{pmatrix} v \leq -c_{\lambda}$$ 
with $\tilde{D}^{\alpha}$ and $D^{\alpha}(\tilde{\textbf{X}}, \textbf{X})$ both $n \times n$ matrices with entries $\tilde{D}^{\alpha} = d_{\alpha}(\tilde{X}_i, \tilde{X}_j)$ and $D^{\alpha}(\tilde{\textbf{X}}, \textbf{X})_{i,j} = d_{\alpha}(\tilde{X}_i,X_j)$. We can now define the linear map $-A: \mathbb{R}^n \to \mathbb{R}^n$ by 
$$ v \to  \begin{pmatrix} D^{\alpha} & D^{\alpha}(\tilde{\textbf{X}}, \textbf{X}) \\ D^{\alpha}(\tilde{\textbf{X}}, \textbf{X})^T & \tilde{D}^{\alpha} \end{pmatrix} \begin{pmatrix} v \\ -\frac{1}{n} 1^T v 1 \end{pmatrix} $$
and using the fact that $1^T \begin{pmatrix} v \\ -\frac{1}{n} 1^T v 1 \end{pmatrix} = 0 $, we
find that for any $v \in \mathbb{R}^n$, 
$$ v ^T-A v \leq \frac{c}{v^T v + \frac{1}{n^2} 1^T v 1  1^T v 1} = \frac{-c}{v^T v + \frac{1}{n^2} v^T 1^T 1 1^T1 v} \leq \frac{-c/2}{v^T v}$$
Therefore, due to the Min-Max Theorem, we find that the maximum Eigenvalue of $\lambda_{max}(-A) \leq -c/2$ and therefore, $\lambda_{min}(A) \geq c/2$. The only thing left in the first step of this proof is to find the kernel matrix $\tilde{k}$ generating $A$. We have that
\begin{equation}
    \begin{split}
        -w^T Av &= \begin{pmatrix} w \\ -\frac{1}{n} 1^T w 1 \end{pmatrix}  \begin{pmatrix} D^{\alpha} & D^{\alpha}(\tilde{\textbf{X}}, \textbf{X}) \\ D^{\alpha}(\tilde{\textbf{X}}, \textbf{X})^T & \tilde{D}^{\alpha} \end{pmatrix} \begin{pmatrix} v \\ -\frac{1}{n} 1^T v 1 \end{pmatrix} \\
                &= w^T D^{\alpha} v - w^T \left[\frac{1}{n} 1 1^TD^{\alpha}(\tilde{\textbf{X}}, \textbf{X}) \right] v - w^T \left[ \frac{1}{n} D^{\alpha}(\tilde{\textbf{X}}, \textbf{X})^T 1 1^T \right] v  + w^T \left[ \frac{1}{n^2} 1 1^T \tilde{D}^{\alpha} 1 1^T \right] v
            \end{split}
\end{equation} 
We can thus see that $A$ is obtained when evaluating the kernel function 
$$\tilde{k}(X,X') := \frac{1}{n} \sum_{i =1}^n d_{\alpha}(X,X_i) + d_{\alpha}(X_i,X') - \frac{1}{n^2} \sum_{i,j=1}^{n} \left(d_{\alpha}(X_i,X_j)  - d_{\alpha}(X,X') \right)$$
at $\textbf{X}$. 
\\\\
\textbf{Step 2:}
We have that $\exp(-d_{\alpha}(X,X')) = \exp(\tilde{k}(X,X')) \exp(-d_{\alpha}(X,X') - \tilde{k}(X,X')) $, with $\phi(X,X') := -d_{\alpha}(X,X') - \tilde{k}(X,X') = \frac{1}{n^2} \sum_{i,j=1}^{n} d_{\alpha}(X_i,X_j)  - \frac{1}{n} \sum_{i =1}^n \left(d_{\alpha}(X,X_i) - d_{\alpha}(X_i,X') \right)$. Next, note that $\exp(\phi(X,X'))$ is a positive definite function. Hence, by Schur's product Theorem, we have that
$$ exp(-d_{\alpha}(X,X')) = \exp(\tilde{k}(X,X')) \exp(\phi(X,X')) = \sum_{l=0}^{\infty} \frac{1}{l!} \tilde{k}(X,X')^l \exp(\phi(X,X')) $$
is a sum of positive definite functions. Therefore, it is sufficient to show that the Eigenvalues of the kernel matrix $M$ of $\tilde{k}(X,X') \exp(\phi(X,X'))$, evaluated at $\textbf{X}$, are lower bounded. Let $B$ be the kernel matrix of $\exp(\phi(X,X'))$ evaluated at $\textbf{X}$, we have that $M = A \circ B$, where $\circ$ is the Hadamard product. We make the following Claim, from which the proof follows trivially using the fact from the first step that the Eigenvalues of $A$ are lower bounded by a positive non zero constant.
\\\\
\textbf{Claim:} $B = 1/2 11^T + \tilde{B}$ with $\tilde{B}$ a positive definite matrix. 
\\\\
\textbf{Step 3: Proof of the Claim} The only thing which is left to conclude the proof is to show that the Claim holds true. Let $\psi$ be the vector with entries $\psi_i = \exp(- \frac{1}{n} \sum_{j=1}^n -d_{\alpha}(X_i,\tilde{X}_j))$. Furthermore, let $\gamma = \exp(\frac{1}{n^2} \sum_{i,j=1}^{n} d_{\alpha}(\tilde{X}_i, \tilde{X}_j))$. We can write
$$ B = \gamma \left(1 \psi^T\right) \circ \left( \psi 1^T \right) = \gamma \psi \psi^T$$
Next, due to Equation \ref{eq:tmpconineq}, we can see that $$ \left| 2^{\alpha/2} - \frac{1}{n^2} \sum_{i,j=1}^{n} d_{\alpha}(\tilde{X}_i, \tilde{X}_j)) \right| \leq \frac{(n^2-n) n^{-\beta/2}\log(n)^{1+\epsilon} + n}{n^2} \to 0 ~~~a.s. $$
where we have used the fact that $d_{\alpha}(X,X') =  2^{\alpha/2} + O(\frac{||X-X'||_2^2}{2} -1 )$.  Thus, $ \gamma \geq \exp( 2^{\alpha/2}/2) >1 ~~a.s.$, and hence, it is sufficient to show that $  \psi \psi^T - \frac{1}{2} ~ 1 1^T $ is positive definite. However, this is true if and only if $1^T \psi \psi^T 1 \geq \frac{1}{2} 1 1^T 1 1^T$, which is equivalent to saying that $ \sum_{i,j}^n  d_{\alpha}(X_i, \tilde{X}_j) \geq \frac{n^2}{2}$. However, using again the same argument as for $\gamma$, we can see that $\left|  2^{\alpha/2} - \frac{1}{n^2} \sum_{i,j}^n  d_{\alpha}(X_i, \tilde{X}_j) \right| \to 0 ~~ a.s.$, which completes the proof.
\end{proof}
