# Supplementary material for: How rotational invariance of common kernels prevents generalization in high dimensions
Source: arXiv:2104.04244 source file (2021-04-09)
Supplement: Supplementary file 7 [file Appendix_RKHS_Norm.tex]

\section{Bounded Hilbert norm assumption}
This section provides a formal discussion of the bounded Hilbert norm assumption when the dimension $d\to\infty$ (this is assumed in \cite{Liang20b,Liang20a}).  Section \ref{sec:norm} gives a formal statement of Lemma \ref{lm:rkhs} and Section \ref{sec:rkhsnorm_liang} presents a corollary combining the results from Theorem \ref{thm:main_thm} with the ones in \cite{Liang20b} showing that the functions with asymptotically bounded Hilbert norm are at most degree-2 polynomials around the sphere. 

\subsection{Precise statement of Lemma \ref{lm:rkhs} and its proof}
\label{sec:norm}
We now introduce the conditions under which Lemma \ref{lm:rkhs} holds. We consider tensor product kernels of the form 
\begin{equation*}
\label{eq:kernflrkhs}
 \kerfuncseq{\xk}{\xkd}= \prod_{j=1}^d
\kerfuncentry(x_{(j)},x'_{(j)})
\end{equation*}
with inputs $\xk,\xkd \in \XX^{\otimes d} \subset \RR^d$ 
with $\XX$ compact, for some kernel function $\kerfuncentry$ on $\XX$ which may 
change with $d$ (e.g. the scale parameter). In order to prevent the sequence of kernels $\kernf$ to diverge as $d \to \infty$, assume that there exists some probability measure on $\XX$ such that the trace of the kernel operator is bounded by $1$, i.e. $\int \kerfuncentry(x,x) d\mu(x) \leq 1$. Let $\|. \|_{\Hilbertspace_{k}}$ be the Hilbert norm induced by $k$. Then,

\begin{lemma}[Formal statement of Lemma \ref{lm:rkhs}]
  \label{lm:rkhsformal}
Let $\kernf$ satisfy the above conditions. Then, for any $f$ that is a non-constant sparsely parameterized product
function $f(\xk) = \prod_{j=1}^m f_j(\xel{j})$ for some fixed $m \in
\N$, %for any sequence $\Hilbertspace_d$ defined above,
\vspace{-0.1in}

\begin{equation*}
  \| f \|_{\Hilbertspace_k} \overset{d \to \infty}{\to} \infty.
\end{equation*}
\end{lemma}

\begin{proof}
 For any $j>m$, define $f_j = 1$. First, we note that the proof follows trivially if any of the $f_j$ is not contained in the RKHS induced by $q$ since this implies that the Hilbert norm $\|f\|_{\Hilbertspace_{k}} = \infty$. Hence, we can assume that for all $j$, $f_j$ is contained in the RKHS for all $d$. Furthermore, because $k$ is a product kernel, we can write
 $\| f \|_{\Hilbertspace_{k}} = \prod_{j=1}^d \| f_j \|_{\Hilbertspace_{q}}$ where $\|. \|_{\Hilbertspace_{q}}$ is the Hilbert norm induced by $q$ on $\XX$. Without loss of generality we can assume that $m =1$ and hence,
\begin{equation}
\label{eq:rkhsnormeq}
 \| f \|_{\Hilbertspace_{k}} = \| f_1 \|_{\Hilbertspace_{q}} (\| 1\|_{\Hilbertspace_{q}})^{d-1}.
\end{equation}
  
Next, by Mercer's theorem there exists an orthonormal eigenbasis $\{ \phi_{i} \}_{i=1}^{\infty}$ with corresponding eigenvalues $\{\lambda_{i} \}_{i=1}^{\infty}$ and $\| f \|_{\Hilbertspace_{q}} = \sum_{i=1}^{\infty} \frac{(\langle f, \phi_{i}\rangle)^2}{\lambda_{i}}$, where $\langle f, \phi_{i}\rangle = \int \phi_{i}(x) f(x) d\mu(x) $.
Note that  because the kernel $q$ depends on $d$, $\lambda_i$ and $\phi_i$ also depend on $d$. Next, because by assumption $f(x) =1$ is contained  in the RKHS, there exists $\alpha_i$ such that for every $x \in\XX$, $ 1 = \sum_{i=1}^{\infty} \alpha_{i} \phi_{i}(x)$ and $\sum_{i=1}^{\infty} \alpha_{i}^2 = 1$. Furthermore,
\begin{equation*}
\begin{split}
 1 \geq \int \kerfuncentry(x,x) d\mu(x)& = \int \sum_{i=1}^{\infty} \lambda_{i} \phi_{i}(x)\phi_{i}(x) d\mu(x) =  \sum_{i=1}^{\infty} \lambda_{i}.
\end{split}
\end{equation*}
Combining these results, we get that 
\begin{equation*}
\label{eq:rkhsnormeq2}
 \| 1\|_{\Hilbertspace_{q}} = \sum_{i =1}^{\infty} \frac{\alpha_{i}^2}{\lambda_{i}} \geq 1.
\end{equation*}
Furthermore, there exists $\beta_i$ such that $f_1(x) =
\sum_{i=1}^{\infty} \beta_{i} \phi_i(x)$. Without loss of generality
we can assume that $\sum_{i=1}^{\infty} \beta_{i}^2 = 1$ and hence
also, $\| f_j \|_{\Hilbertspace_{q}} \geq 1$.

We now show that $\|1\|_{\Hilbertspace_q} \to c> 1$ from which the proof then follows using Equation~\ref{eq:rkhsnormeq}.
We prove this fact by contradiction.
%% Assume that $\| f
%% \|_{\Hilbertspace_{k}} \leq M$ for some $M>0$.
%% Clearly, we require
First assume that $\| 1\|_{\Hilbertspace_{q}} \to 1$. This implies that
there exists a sequence $j_d \in \NN$ such that $\alpha_{j_d}^2 \to 1$
and $\lambda_{j_d} \to 1$. Next, because by assumption $f_1 \neq 1$,
there exists some constant $c_1>0$ such that for all $d$,
% Because $\| f_1 \|_{\Hilbertspace{q}} \geq 1$, we require that $(\| 1\|_{\Hilbertspace_{q}})^{d-1} \geq 1$ stays bounded. This implies that $\| 1\|_{\Hilbertspace_{q}} \to 1$ as $d$ increases, which is equivalent to saying that $ \sum_{i =1}^{\infty} \frac{\alpha_{i}^2}{\lambda_{i}} \to 1$ and using the fact that the $\sum_{i=1}^{\infty} \lambda_{i} \leq 1$ and $\sum_{i=1}^{\infty} \alpha_{i}^2 = 1$, we conclude that this implies that there  But we also have that 
\begin{equation*}
  c_1 \leq \int (1-f_1(x))^2 d\mu(x)  = \sum_{i=1}^{\infty} (\alpha_{i} - \beta_{i})^2.
\end{equation*}
Together with the fact that $\alpha_{j_d}^2 \to 1$ it then follows that
$\sum_{i \neq j_d} \beta_{i}^2$ has to be asymptotically lower bounded
by some non-negative constant $c_2$ and hence
%% , there exists some
%% constant $c_2>0$ such that for any $d$ sufficiently large, $\sum_{i
%%   \neq j_d} \beta_{i}^2 \geq c_2>0$. However, this implies that
\begin{equation*}
 \|f_1\|_{\Hilbertspace_{q}} \geq \frac{c_2}{(1- \lambda_{j_d})} \to \infty.
\end{equation*}
This contradicts the assumption that $\|f_1\|_{\Hilbertspace_{q}}$ is
upper bounded by some constant for every $d$. We have hence proven that $\|1\|_{\Hilbertspace_q} \to c > 1$ and the proof is complete.
% for any $j\leq m$.  Hence, it is sufficient if we show that Lemma \ref{lm:rkhs} holds for the case where $m=1$.
% Let $\beta_{i}$ the coefficients of $f_1$, i.e. $f_1(x) = \sum_{i=1}^{\infty} \beta_{i} \phi_{i}(x)$. Since $\| f_1 \|_{\Ell^2(\mu)} =1$, $\sum_{i=1}^{\infty} \beta_{i}^2 = 1$. Next, note that because $f_1$ is non constant,$\int (f_1(x) - 1)^2 d\mu(x) = \sum_{i=1}^{\infty} (\alpha_{i} - \beta_{i})^2 = c_f$, where $c_f >0$ is constant independent of $d$. 
% We can now prove the lemma by contradiction.
\end{proof}

\subsection{Bounded Hilbert norms and the polynomial approximation barrier}
\label{sec:rkhsnorm_liang}
Theorem 3 in \cite{Liang20b} and the subsequent remark provide a vanishing upper bound of the bias for the regime where $\inputcov = \idmat_d$ and $d \asymp n^{\beta}$ assuming that the Hilbert norm $\| \ftrue \|_{\Hilbertspace}$ of the sequence of ground truth functions $\ftrue$ remains bounded as $d \to \infty$. The following corollary states that for the same setting as in \cite{Liang20b}, with $\prob_X \in \probsetcov$ satisfy Assumption \Bdone-\Bdtwo~with $\beta = 0.9$ and $\inputcov = \idmat_d$, $\fstar$ converges in $\Ell_2(\prob_X)$ norm to a polyonmial of degree at most $2$.

\begin{cor}
\label{cr:rkhsnorm_liang}
 Let $k$ be an inner product kernel satisfying the assumptions in Theorem 3 in \cite{Liang20b} and assume that $\prob_X \in \probsetcov$ satisfy Assumption \Bdone-\Bdtwo~with $\beta = 0.9$ and $\inputcov = \idmat_d$.
 Furthermore, let $\Hilbertspace_k$ be the corresponding sequence of RKHS on the support of $\prob_X$ and assume that $\ftrue$ is a sequence of ground truth functions having bounded Hilbert norm as $d \to \infty$. Then, 
 
 \begin{equation*}
     \underset{\polyf \in
      \polyspace{2}}{\inf} \| \ftrue -
    \polyf \|_{\Ell_2(\prob_X)}\to 0
\end{equation*}
\end{cor}

\begin{proof}
 First of all, note that both the marginal distribution $\prob_X$ and the kernel function $\kernf$  satisfy the assumptions in Theorem \ref{thm:main_thm} and Theorem 3 in \cite{Liang20b}. 
% Furthermore, based on the remark after Theorem 3 in \cite{Liang20b}, we can see that any ground truth function with $\| \ftrue\|_{\Hilbertspace}$ bounded satisfies the assumptions in Theorem 3
Because by assumption $\fstar$ has bounded Hilbert norm, Theorem 3 in \cite{Liang20b} and the subsequent remark imply that for
any $\delta >0 $, with probability $1-\delta$ over the draws of $\Xs$,
 \begin{equation*}
  \Bias(\fhatinterpol) \lesssim (n^{-1}+ n^{-0.1})\frac{1}{\delta} \to 0.
 \end{equation*}
 On the other hand, because $m = \floor{2/\beta} =2$ (where we use the fact that $k$ is an inner product kernel),  Theorem \ref{thm:main_thm} and Remark \ref{rm:astoinp} show that as $n\to \infty$, with probability $\geq 1-n^2 \exp(-C \ (\log(n))^{(1+\epsilon)/2})$ over the draws of $\Xs$ and for any $\gamma >0$, 
 \begin{equation*}
     \Bias(\fhatinterpol) \geq \underset{\polyf \in
      \polyspace{2}}{\inf} \| \ftrue -
    \polyf \|_{\Ell_2(\prob_X)} -\gamma.
\end{equation*}
Hence, we can conclude the proof by combining these two results.
 
\end{proof}
