# Supplementary material for: How rotational invariance of common kernels prevents generalization in high dimensions
Source: arXiv:2104.04244 source file (2021-04-09)
Supplement: Supplementary file 9 [file Appendix_Theorem1.tex]

\section{Proof of Theorem \ref{thm:main_thm}}
\label{sec:proofmainthm}

%%%%%%%%%%%%%%%%%% Theorem %%%%%%%%%%%%%%%%%% 

In this section we first introduce generalized assumptions
that allows us to cover the case when $\bw/\effdim \to \cbw\neq 1$
and state the key concentration inequalities used throughout the proof.
We then present the proof of the (generalized) theorem.

Theorem \ref{thm:main_thm} assumes for the brevity of notation that $\bw/\effdim = 1$. 
In this section we present our results for the more general case where
\begin{equation*}
 \cnbw \define \effdim/\bw \to \cbw,
\end{equation*}
with $\cbw >0$ some constant. For this purpose, we first restate the
Assumption \Akone-\Aktwo~ and the $\beta$-dependent assumptions in
Theorem \ref{thm:main_thm}, for the case where $\cbw \neq 1$. In
particular, the local assumptions more generally center around a
sphere of radius $\cbw$ instead of $1$:

\begin{itemize}

\item[\Akonebracket] \textit{Local power expansion}: 

  The kernel $\kernf$ can be expanded as a power series
  \begin{equation}
    \label{eq:kerneldefg}
    \begin{split}
    \kerfunc{\xk}{\xkd} &= \rotkerfunc(\|\xk\|_2^2, \|\xkd\|_2^2, \xk^\top \xkd) = \sum_{j=0}^{\infty} \rotkerfunccoeffj{j}(\|\xk\|_2^2,\|\xkd\|_2^2) (\xk^\top \xkd)^j 
    \end{split}
   \end{equation}
  that converges for $\xk, \xkd$ in a neighborhood of the sphere
  $\{x\in \R^d \mid \|x\|^2 \in [\cbw-\delta,\cbw+\delta]\}$
  for some
   $\delta > 0$. Furthermore, all $g_i$ are positive semi-definite
   kernels.

\item[\Aktwobracket] \textit{Restricted Lipschitz
  continuity:} The restriction of $k$ on $\{(x,x)| x \in \R^d,
 \| x \|_2^2 \in [\cbw-\delta_L, \cbw+\delta_L]\}$ is
  a Lipschitz continuous function for some constant $\delta_L>0$.

   \item[\Akthreebracket] \textit{$\beta$-dependent assumptions:} $g_i$ is $(\floor{2/\beta}+1-i)$-times
  continuously differentiable in a neighborhood of $(\cbw,\cbw)$ and there
  exists $\jthresh > \floor{2/\beta}$ such that
  $\rotkerfunc_{\jthresh}(\cbw,\cbw) >0$.
\end{itemize}

Furthermore, we would like to point out the key
ingredient that we use throughout the proof in the following sections.
In particular, Theorem \ref{thm:main_thm} heavily relies on the concentration of
Lipschitz continuous functions of i.i.d random vectors and its
implications, summarized in the following Lemma.

\begin{lemma}
\label{lm:innerpr}
For any $\epsilon > 0$, there exists $C>0$ such that for any $\prob_X \in \probsetcov$ or $\probsetsphere$, 
\label{lm:norm}
\begin{equation}
\label{eq:innerpreq}
    \max_{i,j }\left| \x_i^\top  \x_j / \tr(\Sigma_d) - \delta_{i, j}\right| \leq n^{-\beta/2} (\log(n))^{(1+\epsilon)/2} ~~~ a.s.
\end{equation}
% and
% \begin{equation*}
%     \max_{i,j }\left|\lvert \lvert \x_i -  \x_j\rvert\rvert_2^2/ \tr(\Sigma_d)- 2(1-\delta_{i, j})\right| \leq n^{-\beta/2} (\log(n))^{(1+\epsilon)/2} ~~~ a.s.
% \end{equation*}
Furthermore, with probability $\geq 1- (n+1)^2 \exp(-C  (\log(n))^{(1+\epsilon)/2})$ over the draws of $\Xrv \sim \prob_X$, 
\label{lm:norm}
\begin{equation}
\label{eq:innerprZ}
\underset{i}{\max}\left| \x_i^\top\Xrv\right|/\tr(\Sigma_d) \leq n^{-\beta/2} (\log(n))^{(1+\epsilon)/2} \quad a.s.,
\end{equation}
and 
\begin{equation}
\label{eq:innerprZZ}
\left| \Xrv^\top \Xrv /\tr(\Sigma_d) -1 \right| \leq  n^{-\beta/2} (\log(n))^{(1+\epsilon)/2} \quad a.s..
\end{equation}
\end{lemma}

We are now ready to provide the proof of the theorem.

\begin{proof}[Proof of Theorem \ref{thm:main_thm}]

The proof of the Theorem is primarily separated into two parts
\begin{itemize}
\item We first state Theorem \ref{prop:main_thm_ext} which shows under the weaker
  assumptions in ~\Ckone, that the results of
  \ref{thm:main_thm} hold for the ridge estimate $\fhatridge$ for non-vanishing $\lambda>0$
  or the ridgeless estimate whenever the
  eigenvalues of $\kermat$ are asymptotically lower bounded.
  %% apply, given a weaker Assumption~\Ckone and that the eigenvalues
  %% of $(\kermat + \lambda \idmat)$ can be asymptotically lower
  %% bounded by a non-zero positive constant .
\item We finish the proof for the ridgeless estimate by invoking Theorem~\ref{prop:main_thm_ext}
  and showing that $\kermat$ indeed has asymptotically lower
  bounded eigenvalues under the stricter assumptions
  \Akone-\Akthree~imposed in Theorem~\ref{thm:main_thm}.
  %by invoking two propositions showing that there exists some constant $c>$ such that $\kermat \succeq c\idmat_n$.
\end{itemize}

We start by introducing the following weaker assumptions that 
%% The following theorem states the results of the Theorem
%% \ref{thm:main_thm} under the following weaker Assumption \Ckone~ and
%% that $\kermat$ has positive lower bounded eigenvalues.
%% The weaker
%% Assumption \Ckone~
allows us to jointly treat $\alpha$-exponential
kernels and kernels satisfying Assumption \Akone-\Akthree~
when the kernel eigenvalues are lower bounded in
Theorem~\ref{prop:main_thm_ext}. Note that this assumption 
implies that the kernel is rotationally invariant.

% As a second step, we replace Assumptions \Akone-\Akthree~ in the theorem by the following weaker assumption
%\Ckone and refer to the $\beta$-dependent kernel assumption as \Cktwo.

\begin{itemize}

\item[\Ckonebracket] \textit{Relaxation of Assumption \Akone}: 
    Define the neighborhood $\convergesetres{\delta}{\delta'} \subset \R^d \times \R^d$  as
  \begin{equation*}
    \convergesetres{\delta}{\delta'} := \{(\xk,\xkd) \in  \R^d \times \R^d \mid (\|\xk\|_2^2, \|\xkd\|_2^2) \in [\cbw-\delta, \cbw+\delta] \times
  [\cbw-\delta, \cbw+\delta], \xk^\top \xkd \in [-\delta',\delta']\}.
  \end{equation*}
  
  A kernel $\kernf$ has a local power expansion if $\rotkerfunc$ can be expanded as a power series
  \begin{equation}
    \label{eq:kerneldefgap}
    \kerfunc{\xk}{\xkd}= \rotkerfunc(\|\xk\|_2^2, \|\xkd\|_2^2, \xk^\top \xkd) = \sum_{j=0}^{m} \rotkerfunccoeffj{j}(\|\xk\|_2^2,\|\xkd\|_2^2) (\xk^\top \xkd)^j + (\xk^\top \xkd)^{m+1} \reminder(\|\xk\|_2^2, \|\xkd\|_2^2, \xk^\top \xkd)
   \end{equation}
   with $\mc= \floor{2/\beta}$ that converges in a neighborhood $\convergeset{\delta,\delta'}$ of the sphere for some $\delta, \delta'>0$ and where $g_i$ is
  $(\floor{2/\beta}+1-i)$-times continuously differentiable in an
   neighborhood of $(\cbw,\cbw)$ and the reminder term $\reminder$ is a continuous function around the point $(\cbw,\cbw,0)$.

\end{itemize}

\begin{theorem}[Polynomial approximation barrier]
  \label{prop:main_thm_ext}
  Assume that the kernel $\kernf$, respectively its restriction onto the hyper sphere $\kernfuncressphere{d}$, satisfies the assumption \Ckone~ and  that the eigenvalues of the kernel matrix $\kermat$ can be almost surely lower bounded by a non-zero positive constant.
  Furthermore, assume that the ground truth $\ftrue$ is bounded almost surely
  and the input distribution satisfies \Adone-\Adtwo.
  Then, for some $m \in \NN$ specified below, the following results hold for both the ridge~\eqref{eq:krr} and ridgeless estimator~\eqref{eq:constraint_min_p}. %$\fhatridge$ 
  \begin{enumerate}

  \item The bias of the kernel estimators $\fhatridge$ is
    asymptotically lower bounded, for any $\eps > 0$, as $n\to \infty$,
    \vspace{-0.05in}
  \begin{equation}
    \label{eq:apbiaslb}
    \Bias(\fhatridge) \geq \underset{\polyf \in
      \polyspace{m}}{\inf} \| \ftrue -
    \polyf \|_{\Ell_2(\prob_X)} - \eps ~~~a.s. 
  \end{equation}
\item We can find a polynomial $\polyf$ such that for any $\epsilon,\epsilon'>0$, there exits $C>0$ such that asymptotically with probability $\geq 1 - n^2 \exp(-C  (\log(n))^{(1+\epsilon)/2'})$ over the draws of $X$, 
\begin{equation}
\label{eq:appolyapprweak}
     \left| \EEobs \fhatridge(X) - \polyf(X) \right| \leq \epsilon
\end{equation}
Furthermore, for bounded kernel functions on the support of $\prob_X$ the averaged estimator $\EEobs \fhatridge$ converges in $\Ell_2(\prob_X)$ to a polynomial $\polyf  \in \polyspace{m}$  as $n \to \infty$,
  \vspace{-0.1in}
  \begin{equation}
  \label{eq:appolyapproxlp}
    \left\| \EEobs \fhatridge - \polyf \right\|_{\Ell_2(\prob_X)} \to 0
    ~~ a.s..
  \end{equation}
  \end{enumerate}
  \vspace{-0.1in}
  More precisely, if $g_i$ is
  $(\floor{2/\beta}+1-i)$-times continuously differentiable in a
  neighborhood of $(1,1)$ and there exists $\jthresh >
  \floor{2/\beta}$ such that $\rotkerfunc_{\jthresh}(1,1) >0$, then
  the bounds \eqref{eq:biaslb},\eqref{eq:polyapproxlp} hold with $m =
  2 \floor{2/\beta}$ for $\prob_X \in \probsetcov$ and $m =
  \floor{2/\beta}$ for $\prob_X \in \probsetsphere$.
\end{theorem}

The proof of this theorem can be found in Section~\ref{sec:prop1_proof}.
% 
% \begin{prop}[Polynomial approximation barrier]
%    \label{prop:main_thm_ext}
%     The results in Theorem \ref{thm:main_thm} apply for general
%     kernel functions $\kernf$ where we only require that $\kernf$, respectively its restriction onto the hyper sphere $\kernfuncressphere{d}$, satisfies assumption \Ckone~ and has lower bounded eigenvalues of the kernel matrix $\kermat$ can be almost surely lower bounded by a non-zero positive constant.
% \end{prop}
Theorem~\ref{prop:main_thm_ext} states Theorem~\ref{thm:main_thm}
under the assumption that $(\kermat+\lambda I)$ has asymptotically
lower bounded eigenvalues and weaker Assumptions in \Ckone.  For the
proof of Theorem~\ref{thm:main_thm} it thus remains to show that
Assumptions \Akone-\Akthree~of Theorem ~\ref{thm:main_thm} and the
$\alpha$-exponential kernel both
\begin{itemize}
\item[(a)] satisfy Assumption \Ckone~ and 
\item[(b)] induce kernel matrices with almost surely asymptotically positive lower bounded eigenvalues
\end{itemize}

%% To complete the proof of the theorem we now need to prove that the
%% assumptions of Theorem~\ref{prop:main_thm_ext} are satisfied under
%% the assumptions of Theorem~\ref{thm:main_thm}.  For this we need to
%% show that kernels satisfying \Akone-\Akthree~ and the
%% $\alpha$-exponential kernel both
%% \begin{itemize}
%% \item[(a)] satisfy Assumption \Ckone~ and 
%% \item[(b)] induce kernel matrices with almost surely asymptotically positive lower bounded eigenvalues
%% \end{itemize}

Point (a) is relatively simple to prove and deferred to
Section~\ref{sec:AC_lemmas}. The bulk of the work in fact lies in
showing (b) separately for the case for \Akone-\Akthree~ and
$\alpha$-exponential kernels with $\alpha \in (0,2)$ in the following
two propositions, as these two cases require two different proof
techniques. 

%% Notice that for ridge
%% regression with $\lambda >0$, Theorem~\ref{prop:main_thm_ext}
%% holds whenever (a) is satisfied. This part of the proof is relatively simple. The technical difficulty primarily lies in the proof of part (b).
%% In the following we lay out the 

%% always holds for Assumptions \Ckonebracket.  It is particularly hard to prove that the eigenvalues
%% of the kernel matrix $\kermat$ are asymptotically lower bounded.
%% The difficulty is now to verify that the assumptions in Theorem \ref{thm:main_thm} guarantee that the eigenvalues are lower bounded and hence Propositoin \ref{prop:main_thm_ext} applies. 

%% \paragraph{Lower bound of the eigenvalues for the assumptions \Akone-\Aktwo}

%We first show the eigenvalue bound given Assumption \Akone-\Akthree.
\begin{prop}
\label{prop:EVlowerbound}

Assume that the kernel $\kernf$, respectively its restriction onto the hyper sphere $\kernfuncressphere{d}$, satisfies Assumption \Akone-\Akthree~ and the distribution $\prob_X$ satisfies \Bdone-\Bdtwo.
% In addition, assume that the map $x \to g(x,x,x)$ is Lipschitz continuous in a neighborhood of $\cbw$ (extension of Assumption \Aktwo~ to general $\cbw$) and assume that for any $\xk \in   \convergesetres{\delta}{\delta'}$ (as in Assumption \Ckone), the power series from Equation \eqref{eq:kerneldefgap} can be extended to $g(\|\xk\|_2^2,\|\xk\|_2^2, \xk^\top\xk)$, i.e. $g(\|\xk\|_2^2,\|\xk\|_2^2, \xk^\top\xk) = \sum_{i=0}^{m} (\xk^\top\xkd)^i g_i(\|\xk\|_2^2,\|\xk\|_2^2) +(\xk^\top\xkd)^{m+1} \reminder(\|\xk\|_2^2,\|\xk\|_2^2, \xk^\top\xk) $. Furthermore, assume that any $g_j$ is a positive semi-definite kernel function. 
Then, for any $\gamma >0$ sufficiently small and for $m = \floor{2/\beta}$, 
\begin{equation}
\label{eq:lambdamin}
    \lambda_{min}(K) \geq g(\cbw,\cbw,\cbw) - \sum_{i =0}^m \cbw^i g_i(\cbw,\cbw) - \gamma >0  ~~~a.s.
\end{equation}
\end{prop}

%% \fy{now obsolete} It is straight forward to verify that Assumption \Akone-\Akthree ~satisfy the assumptions in Proposition \ref{prop:EVlowerbound} and hence we can conclude Theorem \ref{thm:main_thm} for any kernel which satisfied Assumption \Akone-\Akthree.

%% Hence,  
%% % .Because $g_j$ is positive semi-definite by assumption \Akone, we have that $g_j(\cbw,\cbw) \geq 0$ and because 
%% % because by assumption there exists $\jthresh >
%% % \floor{2/\beta}$ such that $\rotkerfunc_{\jthresh}(\cbw,\cbw) >0$ . 
%% in order to conclude Theorem \ref{thm:main_thm} it is only left to
%% show that Theorem \ref{prop:main_thm_ext} also applies for the
%% $\alpha$-exponential kernel with $0 < \alpha \leq 2$.

%% For this, we make use of the fact that Proposition \ref{prop:EVlowerbound} applies for the Gaussian kernel, which follows straight forwardly from $\exp(-\|\xk-\xkd\|_2^2) = \sum_{j=0}^{\infty} \frac{2^j}{j!} (\xk^\top \xkd)^j \exp(-\|\xk\|_2^2 - \|\xkd\|_2^2)$. We can then show Proposition \ref{prop:alphaexp} which leads to the desired result. 
% \fy{make sure that in Proof of this next prop., you state where you use that Gaussian kernel satisfies Ass A.1-A.3, don't need it here}
\begin{prop}
\label{prop:alphaexp}
Assume that the Assumptions B.1-B.2 hold true. Then, the minimum
eigenvalues of the kernel matrix of the $\alpha$-exponential kernel
with $\alpha\in(0,2)$ are almost surely lower bounded by some non-zero
positive constant.
\end{prop}
The proof of the Propositions~\ref{prop:EVlowerbound} and~\ref{prop:alphaexp} can be found in
the Sections~\ref{sec:proofa1toa3} and~\ref{sec:proofalphaexp} respectively which concludes the proof of
the theorem.

\end{proof}

%% \paragraph{Lower bound of the eigenvalues for the $\alpha$-exponential kernel}

\begin{remark}
\label{rm:astoinp}
The almost sure conditions are with respect to the sequence of data
sets $\textbf{X}$ induced by $n \to\infty$. As may be seen in the
proof of Lemma \ref{lm:innerpr}, we can replace the almost sure
condition with an in probability condition. I.e for any $\epsilon>0$
there exists a constant $C>0$ such that for any $n$ sufficiently
large, Equation \ref{eq:innerpreq} holds true with probability $\leq
n^2 \exp(-C \ (\log(n))^{(1+\epsilon)/2})$ over the draws of $\Xs$.
\end{remark}

% 
% In fact, as a consequence of our proof we can derive a closed form expression for the polynomial $\polyf$ in Theorem \ref{thm:main_thm}, where we can see that $\polyf$ depends also on $\Z$ only by polynomials of degree at most $2m$. 
% 
% \begin{cor}
%  \label{cr:polyexpr}
% The following polynomial $\polyf$ satisfies Equation \eqref{eq:polyapprox} and \eqref{eq:polyapproxlp} in Theorem \ref{thm:main_thm}:
% \begin{equation*}
%  \polyf = \y^\top (\mmat + \lambda \idmat)^{-1} \mvec_{\Zrv} 
% \end{equation*}
% with $\mmat$ from Proposition \ref{lm:elkarouiextension} and for $m = \floor{2/\beta}$, $\mvec_{\Zrv}$ is given by
% \begin{equation*}
%     \label{eq:Mstar} 
%      \mvec_{\Zrv} =\sum_{i=0}^m (\Z^\top  \Zrv)^{\circ i} \circ \left[
% \sum_{j =0}^{m-i} \sum_{q = 0}^{j}  \frac{g_{i}^{(q,j-q)}(1,1) (\Zrv^\top \Zrv)^{q}}{q!(j-)!} \psi^{\circ (j-q)} \right].
% \end{equation*}
% \end{cor}

%%%%%%%%%%%%%%%%%% Discussion of the assumptions %%%%%%%%%%%%%%%%%% 
\subsection{Discussion of the assumptions}
\label{sec:discussionass}
In this section we briefly discuss the assumptions \Akone-\Akthree~ and compare them with the ones in the literature.

When comparing our assumptions with the literature, it is important to
distinguish between the two domains $\XX = \R^d$ and $\XX =
\Sphere{d}$. In particular, on the sphere, many of the Assumptions simplify.

For example, when restricted to
$\XX=\Sphere{d}$ as in \cite{Ghorbani19,Ghorbani20}, we can use the fact that continuous rotationally invariant
kernels can be expressed by inner product kernels.
In this case, the Assumption~\Akone~ simplifies drastically, as
$\kernfuncressphere{d}(\xk,\xkd)=\rotkerfunc(1,1,\xk^\top \xkd) =
\sum_{j=0}^{\infty} \rotkerfunc_j~(\xk^\top \xkd)^j$.
Furthermore,~\Aktwo~ becomes vacuous.
%In this case  \Akthree~is also required by \fy{all previous works to lower bound bla}.
In order to satisfy Assumption \Akone~and \Akthree,
we require that $\rotkerfunc$ is analytic around $0$,
%which implies that $h(\xk^\top \xkd) = \sum_{j=0}^{\infty} \rotkerfunc_j~(\xk^\top\xkd)^j$
i.e. $h_j \geq 0$. These assumptions are very similar to the ones in
\cite{Ghorbani20,Liang20b}.

In the case when $\XX=\R^d$ (not considered by \cite{Ghorbani19,
  Ghorbani20}), our assumptions allow more general kernel functions
beyond the NTK and inner product kernels studied
in~\cite{Liang20a,Liang20b}.
Assumption \Akone~describes the kernel function in the neighborhood of
the sphere, which is where the distribution $\prob_X$ satisfying
Assumption \Bdone-\Bdtwo~concentrates.
%% The power series expression in
%% Assumption \Akone is the main ingredient for the proofs of Theorem
%% \ref{prop:main_thm_ext} and Proposition \ref{prop:EVlowerbound}.
%% In fact,
The power series expansion implies that $\kernf$ is
rotationally symmetric on $\convergeset{\delta}$ and is the main ingredient for the proofs of Theorem
\ref{prop:main_thm_ext} and Proposition \ref{prop:EVlowerbound}.
Further, the requirement that $g_j$ are positive
semi-definite kernel functions implies that $\kernf$ is a positive
semi-definite kernel function on the restriction
$\convergeset{\delta}$ and plays an essential role in Proposition
\ref{prop:EVlowerbound}.

Assumption \Aktwo~ allows us to approximate the diagonal matrix of the kernel
matrix $K$ in Proposition \ref{prop:EVlowerbound} where the
data concentrates in high dimensions.
Finally, Assumption \Akthree~ensures smoothness and that the eigenvalues of the
kernel matrix are lower bounded, since $(\X^\top \X)^{\circ \jthresh}
\to \idmat$ in operator norm with $\circ$ being the Hadamard
product. 
%% Assumption \Akthree: This assumption is additional regularity
%% assumptions needed for the Taylor series approximation of $g_j$ in
%% Theorem \ref{prop:main_thm_ext}. Furthermore,
%% the assumption that
In particular, the existence of $\jthresh \geq \floor{2/\beta}$ such that
$g_{\jthresh}(\cbw,\cbw) >0$ guarantees that the kernel
function does not reduce to a low degree polynomial when restricted
to the sphere. This fact is essential to show that
the eigenvalues of the kernel matrix $K$ are lower bounded in
Proposition \ref{prop:EVlowerbound}.
Similar assumptions can also be found in the previous works by \cite{Liang20b,Ghorbani20}.

For distributions in $\RR^d$ beyond the sphere, the Assumption
\Akone-\Akthree~ include the popular NTK kernels. Although the
assumptions do not include general RBF kernel functions beyond the
$\alpha$-exponential kernel (including the Gaussian kernel), we remark
that the Assumption \Ckone~ is satisfied by very general RBF kernels
(Lemma \ref{lm:AC_rbf}). Hence, Theorem \ref{prop:main_thm_ext} also
covers the settings studied in \cite{Liu20,Liang20a} where the lower
bound for the eigenvalues follows from \cite{ElKaroui10}.

\subsection{Proof of Theorem \ref{prop:main_thm_ext}}
\label{sec:prop1_proof}

As a first step we discuss the implications of the concentration inequalities from Lemma \ref{lm:innerpr}. For the brevity of the notation, we define $\z_i  = \frac{\x_i}{\sqrt{\bw}}$ and let $\Z$ to be the $n \times n$ matrix with column vectors $\z_i$. Furthermore, we define the random variable $Z = X/\sqrt{\bw}$ with $\Xrv \sim \prob_X$. For any $ j\leq \mc+1,$ $ \alpha = (i_1,i_2)$, let $g_j^{(\mathbf{\alpha})}$ denote the partial derivatives $g_j^{(\mathbf{\alpha})}(x,y) = \frac{\partial^{|\alpha|}}{\partial t_1^{i_1} t_2^{i_2}} g_j(t_1,t_2)|_{x,y}$. In the latter, we denote with $ a \lesssim b$ that there exists a constant $C>0$ such that $a \leq C b$ with $C$ independent of $n,d$.
% Let $\psi$ be the vector with entries $\psi_i = \|\z_i\|_2^2 - 1$. Finally, let $\ev_1 \in \mathbb{R}^d$ be the vector with entries $\ev_1 = (1,0, \cdots, 0)$. 

First, note that Lemma \ref{lm:innerpr} implies that
\begin{equation*}
     \max_{i,j }\left| \z_i^\top \z_j - \cnbw \right| \leq \cnbw n^{-\beta/2} (\log(n))^{(1+\epsilon)/2} ~~~ a.s.
\end{equation*}
Furthermore, define
\begin{definition}
\label{def:Uset}
 For any $\epsilon>0$, conditioned on the input data $\Z$, let $\Uset{\Z} \subset \R^d$ be the set of vectors $\Zrv$ with
\begin{equation*}
    \Uset{\Z} := \left\{ \Zrv | \left|~\|\Zrv\|_2^2- \cnbw\right|  \leq \cnbw n^{-\beta/2} (\log n)^{(1+\epsilon)/2}, ~ \max_{i} |\z_i^\top \Zrv |   \leq \cnbw n^{-\beta/2} (\log n)^{(1+\epsilon)/2} \right\}.
\end{equation*}
\end{definition}
We know from Lemma \ref{lm:innerpr} that for any $\epsilon>0$, there exists $C >0$, such that for $n$ sufficiently large, $\Uset{\Z}$ has measure \begin{equation*}
    P(\Uset{\Z}) \geq 1 - n \exp(-C (\log n)^{(1+\epsilon)/2}) ~~a.s.,
\end{equation*}
which holds true almost surely over the draws of $\Z$, and hence, $ P(\Uset{\Z}) \to 1 ~~a.s.$ as $n \to \infty$.
\begin{remark}
 \label{rm:AC_concentration}
For any $\delta, \delta'>0$, as $n \to \infty$,
\begin{equation*}
 \forall i \neq j ~~(\zind{i},\zind{j}) \in \convergesetres{\delta}{\delta'} ~~a.s.
\end{equation*}
and for any $n$ sufficiently large, for all $\zk \in \Uset{\Z}$,
\begin{equation*}
 \forall i  ~~~(\zind{i}, \zk) \in \convergesetres{\delta}{\delta'} ~~a.s.
\end{equation*}
where the almost sure statement is with respect to the draws of the input data $\Z$.  
\end{remark}
The following proof is now separated into three steps. In a first step, we derive a polynomial approximation of $\fhatridge$ for the high probability regions $\Uset{\Z}$ and in a second step we  control the resulting polynomial in the low probability regions $\Uset{\Zs}^{\comp}$. Finally, in a last step we lower bound the bias based on the results from the first two steps. \\

\textbf{Step 1:}
In a first step, assume that $\Zrv \in \Uset{\Z}$. Thus,
\begin{equation}
\label{eq:thmainxstar1}
    \max_{i}\left| \z_i^\top\Zrv\right| \lesssim n^{-\beta/2}(\log(n))^{(1+\epsilon)/2} \quad a.s.,
\end{equation}
and 
\begin{equation}
\label{eq:thmainxstar2}
    \left| \Zrv^\top\Zrv -\cnbw \right| \lesssim  n^{-\beta/2}(\log(n))^{(1+\epsilon)/2} \quad a.s.,
\end{equation}
where we have used that $\cnbw \to \cbw$ converges to $\cbw$ and hence does not diverge.  
We make use of Assumption \Ckone and the Taylor series expansion of $g_i$ around the point $(\cnbw,\cnbw)$:

\begin{equation*}
    \begin{split}
    \forall i ~~ \kvec_{i} &=  \sum_{q=0}^{m} (\z_i^\top\z_j)^q g_q(\|\z_i\|_2^2,\|\z_j\|_2^2) 
    +(\zind{i}^\top \Zrv)^{m+1} \reminder(\|\zind{i}\|_2^2, \|\Zrv\|_2^2, \zind{i}^\top \Zrv) ~~~a.s. \\
       &= \sum_{q =0}^m (\z_i^\top\Zrv)^{q} \sum_{ l_1+l_2 \leq m-q} \frac{ g_{q}^{(l_1,l_2)}(\cnbw,\cnbw)}{l_1
    ! l_2!} (\z_i^\top\z_i -\cnbw )^{l_1} (\Zrv^\top\Zrv -\cnbw)^{l_2}   \\ 
    &+ \sum_{q =0}^{m}(\z_i^\top\Zrv)^{q} \sum_{ l_1+l_2  = m+1-q} \frac{ g_{q}^{(l_1,l_2)}(\eta^{q,i}_{l_1,l_2})}{l_1
    ! l_2!} (\z_i^\top\z_i -\cnbw )^{l_1} (\Zrv^\top\Zrv -\cnbw )^{l_2}   \\ 
    &+(\zind{i}^\top \Zrv)^{m+1} \reminder(\|\zind{i}\|_2^2, \|\Zrv\|_2^2, \zind{i}^\top \Zrv) ~~~a.s..
    \end{split}
\end{equation*}
where $\eta^{q,i}_{l_1,l_2} \in B_r(\cnbw,\cnbw)$ are points contained in the closed ball around the point $(\cnbw,\cnbw)$ with radius $r^2 = (\|\z_i\|_2^2-\cnbw)^2 + (\|\Zrv\|_2^2-\cnbw)^2 \to 0~~a.s.$. Hence, using the fact that $g_i$ is $\mc+1-i$-times continuously differentiable and that $\cnbw \to \cbw$,  we can see that any $\|g_{q}^{(l_1,l_2)}(\eta^{q,i}_{l_1,l_2})\|$ is almost surely upper bounded by some constant. 
For the rest of this proof we assume for the brevity of notation that $\cnbw = \cbw =1 $. The general case follows then trivially.

Next, define the vector $\mvec_{\Zrv} \in R^{n}$
\begin{equation*}
    \begin{split}
    \mvec_{\Zrv,i} :=  \sum_{q =0}^\mc (\z_i^\top\Zrv)^{q}  \sum_{ l_1+l_2 \leq \mc-q} \frac{ g_{q}^{(l_1,l_2)}(1,1)}{l_1
    ! l_2!} (\z_i^\top\z_i -1 )^{l_1} (\Zrv^\top\Zrv -1 )^{l_2}.
    \end{split}
\end{equation*}
The goal is now to show that 
\begin{equation}
\label{eq:PB1_eq1}
    \sqrt{n}\| \mvec_{\Zrv} - \kvec \|_2 \leq n \underset{i}{\max} |\mvec_{\Zrv,i} -\kvec_i | \to 0 \quad a.s.
\end{equation}
For this, note that
\begin{equation*}
    \begin{split}
        \sqrt{n}\| \mvec_{\Zrv} - \kvec \|_2 &\lesssim n \max_{i} \underbrace{ \left|\sum_{q =0}^{\mc} (\z_i^\top\Zrv)^{q} \sum_{ l_1+l_2  = \mc+1-q} \frac{ g_{q}^{(l_1,l_2)}(\eta^{q,i}_{l_1,l_2})}{l_1
    ! l_2!} (\z_i^\top\z_i -1 )^{l_1} (\Zrv^\top\Zrv -1)^{l_2}  \right| }_{=: B_1^{i}} \\ &+ n \max_{i\neq j}\underbrace{\left|(\zind{i}^\top \Zrv)^{q+1} \reminder(\|\zind{i}\|_2^2, \|\Zrv\|_2^2, \zind{i}^\top \Zrv)   \right| }_{=: B_2^{i}} ~~ a.s.\\ 
    \end{split}
\end{equation*}
First, we show that the term $n \max\limits_{i} B^{i}_1 \to 0$. Due to the above discussion, we know $\left\| g_{q}^{(l_1,l_2)}(\eta^{q,i}_{l_1,l_2}) \right\|$ is almost surely upper bounded by some constant independent of $i$. Hence, we can apply Lemma \ref{lm:innerpr} which shows that for any positive $q,l_1$ and $l_2$ such that $q+l_1+l_2 = \mc+1$,
\begin{equation*}
    \left| (\z_i^\top\z_i -1 )^{l_1} (\Zrv^\top\Zrv -1 )^{l_2} (\z_i^\top\Zrv)^{q}\right| \lesssim (n^{-\beta/2}(\log(n))^{(1+\epsilon)/2})^{\mc+1} ~~~ a.s.
\end{equation*}
which holds true for any positive constant $\epsilon >0$.
Finally, because $\mc = \floor{2/\beta}$,  $(\beta/2)(\mc+1) > 1$, and hence 
\begin{equation*}
    n \max_{i} B^{i}_1 \lesssim n (n^{-\beta/2} (\log(n))^{(1+\epsilon)/2})^{\mc+1} \to 0~~a.s..
\end{equation*} 
Next, because $\reminder$ is a continuous function, we know that $\reminder$ has a maximum $|\reminder| \leq \Creminder$ in a closed neighborhood of $(1,1,0)$. Therefore, 
\begin{equation*}
n \max_{i} B^{i}_2 \leq n \max_{i} \left| (\z_i^\top\Zrv)^{q+1} \right| \Creminder \lesssim  n \left(n^{-\beta/2}(\log(n))^{(1+\epsilon)/2}\right)^{\mc+1} ~~~ a.s. \to 0,
\end{equation*}
where we have again used Lemma \ref{lm:innerpr}. As a result we can conclude conclude Equation \eqref{eq:PB1_eq1}.

Next, due to the representer theorem, for any $\lambda \geq 0$, we can express $\fhatridge$ as
\begin{equation*}
 \fhatridge(X) = (\kermat +\lambda \idmat_n)^{-1}k(X)
\end{equation*}
with $\kvec \in \RR^n$ the vector with entries $\kvec_i = \kernf_{\bw}(\x_i,X) = k(\z_i,\Zrv)$. Because by assumption $\lambda_{min}(K + \lambda I_n)\geq \minEV >0 ~~a.s.$,
\begin{equation*}
   \|(K + \lambda I_n)^{-1} (\kvec - \mvec_{\Zrv}) \|_1 \leq \sqrt{n}\|(K + \lambda I_n)^{-1} (\kvec - \mvec_{\Zrv}) \|_2 \leq \frac{1}{\minEV} \sqrt{n} \| \kvec - \mvec_{\Zrv}\|_2 \to 0 ~~a.s.
\end{equation*}

Because $\fhatridge$ depends only linearly on the observations,  
\begin{equation*}
 \EEobs \fhatridge = \ftrue(\X)^\top (K + \lambda I_n)^{-1} \kvec
\end{equation*}
where $\ftrue(\X)$ is the vector with entries $\ftrue(\X)_i = \ftrue(\xind{i})$ and $\kvec$ is the vector with entries $\kvec_i = \kernf(\z_i,\Zrv)$. Because all entries are bounded by assumptions, 
\begin{equation}
\label{eq:prop1_eq1}
\begin{split}
  \left|\ftrue(\X)^\top (K + \lambda I_n)^{-1} \kvec -  \ftrue(\X)^\top (K + \lambda I_n)^{-1} \mvec_{\Zrv} \right| \leq  \ubfunc \| (K + \lambda I_n)^{-1} \kvec -  (K + \lambda I_n)^{-1} \mvec_{\Zrv} \|_1 \to 0,
\end{split}
\end{equation}
where we have used that $|\ftrue| \leq \ubfunc$. As a result, we find that 
\begin{equation*}
 \polyf(\Zrv) := \ftrue(\X)^\top (K + \lambda I_n)^{-1} \mvec_{\Zrv}
\end{equation*}
 is a linear combination of the terms $(\Zrv^\top\Zrv)^{p_1}(\z_i^\top\Zrv)^{p_2}$ with $p_1 + p_2 \leq \mc$, and hence a polynomial of $\Zrv$ of degree at most $2m$. In addition, we can see that if $g_j$ are constant, i.e. the kernel is an inner product kernel then $\ftrue(\X)^\top (K + \lambda I_n)^{-1} \mvec_{\Zrv}$ only contains the terms  $(\z_i^\top\Zrv)^{l}$ and hence is a polynomial of $\Zrv$of degree at most $m$.  
 We are now going to show that the polynomial $\polyf$ satisfies point 2) in Theorem \ref{prop:main_thm_ext}. The first point, i.e. Equation \eqref{eq:appolyapprweak}, follows trivially
because the convergence in Equation \eqref{eq:prop1_eq1} is uniform for any $\Zrv \in \Uset{\Z}$. \\

\textbf{Step 2:} In order to show Equation \eqref{eq:appolyapproxlp} in Theorem \ref{prop:main_thm_ext}, we first need to control the error for regions where $\Zrv \in \Uset{\Z}^{\comp}$. Define the event
\begin{equation*}
    E_{n} = \{ \max_{i,j} |\z_i^\top \z_j |   \leq n^{-\beta/2} (\log n)^{(1+\epsilon)/2}, ~ \max_{i} \left|~\lvert\lvert\z_i \rvert\rvert_2^2- 1\right|  \leq n^{-\beta/2} (\log n)^{(1+\epsilon)/2} \}.
\end{equation*}
We know from Lemma~\ref{lm:innerpr} that conditional on $E_{n}$ the event $\Zrv \in \Uset{\Z}$ has probability
\begin{equation*}
    \begin{split}
    P(Z\in \Uset{\Z}| E_{n}) &\geq P(\{Z\in \Uset{\Z}\} \cap E_{n})\\
    &\geq 1 - (n+1)^2 \exp(-C(\log (n))^{(1 + \epsilon)/2}).
    \end{split}
\end{equation*}

Conditional on $E_{n}$, we can see from the discussion in step 1 that
\begin{equation*}
    \max_{i} \left\| \mvec_{i} \indicator_{\Zrv \in \Uset{\Z}^{\comp}} \right\|_{\Ell_2(\prob_X)} \lesssim \sum_{q + l_{1} + l_{2} \leq m} \left\| (z_{i}^\top \Zrv)^{q} (z_{i}^\top z_{i} - 1)^{l_{1}} (\Zrv^\top \Zrv - 1)^{l_{2}} \indicator_{\Zrv \in \Uset{\Z}^{\comp}} \right\|_{\Ell_2(\prob_X)}.
\end{equation*}
Define $\psi_i = \|\z_i\|_2^2 - 1$. Then, for any $q + l_{1} + l_{2} \leq m$,  
\begin{equation*}
    \begin{split}
        &~~\left\| (z_{i}^\top \Zrv)^{q} \psi_i^{l_{1}} \left( \left\|\Zrv \right\|^{2} - 1 \right)^{l_{2}} \indicator_{\Zrv \in \Uset{\Z}^{\comp}} \right\|_{\Ell_2(\prob_X)} 
        \\
        &\leq \left\| (\psi_i + 1)^{\frac{q}{2}} \left\|\Zrv \right\|^{q} \psi_i^{l_{1}} \left( \left\|\Zrv \right\|^{2} - 1 \right)^{l_{2}} \indicator_{\Zrv \in \Uset{\Z}^{\comp}} \right\|_{\Ell_2(\prob_X)}\\
        &\leq \left( 1 + n^{-\frac{\beta}{2}} (\log(n))^{(1 + \epsilon)/2}\right)^{\frac{m}{2}} \left\| \left\|\Zrv \right\|^{q} \left( \left\|\Zrv \right\|^{2} - 1 \right)^{l_{2}} \indicator_{\Zrv \in \Uset{\Z}^{\comp}} \right\|_{\Ell_2(\prob_X)}~~a.s.\\
        &\lesssim 2\left\| \left\|\Zrv \right\|^{q} \left( \left\|\Zrv \right\|^{2} - 1 \right)^{l_{2}} \indicator_{\Zrv \in \Uset{\Z}^{\comp}} \indicator_{ \left\{ \left\|\Zrv \right\|^{2} \leq 1 + n^{-\frac{\beta}{2}} (\log(n))^{ (1 + \epsilon)/2} \right\}} \right\|_{\Ell_2(\prob_X)}\\
        &+ 2\left\| \left\|\Zrv \right\|^{q} \left( \left\|\Zrv \right\|^{2} - 1 \right)^{l_{2}} \indicator_{ \left\{ \left\|\Zrv \right\|^{2} > 1 + n^{-\frac{\beta}{2}} (\log(n))^{(1 + \epsilon)/2} \right\}} \right\|_{\Ell_2(\prob_X)}~~a.s..
    \end{split}
\end{equation*}
For the first term, 
\begin{equation*}
    \begin{split}
        &~~~\left\| \left\|\Zrv \right\|^{q} \left( \left\|\Zrv \right\|^{2} - 1 \right)^{l_{2}} \indicator_{\Zrv \in \Uset{\Z}^{\comp}} \indicator_{ \left\{ \left\|\Zrv \right\|^{2} \leq 1 + n^{-\frac{\beta}{2}} (\log(n))^{(1 + \epsilon)/2} \right\}} \right\|_{\Ell_2(\prob_X)}  \\ 
        &\leq  2^{m} P(Z\in \Uset{\Z}^{\comp}| E_{n})~~a.s.\\
        &\leq  2^{m} (n+1)^2 \exp(-C(\log (n))^{(1 + \epsilon)/2})~~a.s..
    \end{split}
\end{equation*}
Furthermore, from the proof in Lemma~\ref{lm:concentration} we can see that there exists some constant $c > 0$, such that
\begin{equation*}
    P\left( \left\|\Zrv \right\|^{2} > r \right) \leq \exp(-c n^{\beta} r).
\end{equation*}
Hence, the second term satisfies that
\begin{equation*}
    \begin{split}
            \left\| \left\|\Zrv \right\|^{q} \left( \left\|\Zrv \right\|^{2} - 1 \right)^{l_{2}} \indicator_{ \left\{ \left\|\Zrv \right\|^{2} > 1 + n^{-\frac{\beta}{2}} (\log(n))^{(1 + \epsilon)/2} \right\}} \right\|_{\Ell_2(\prob_X)}^{2} &\leq \int \left\|\Zrv \right\|^{q + 2l_{2}} \indicator_{ \left\{ \left\|\Zrv \right\|^{2} > 1 + n^{-\frac{\beta}{2}} (\log(n))^{(1 + \epsilon)/2} \right\}} dP\\
            &\leq \int_{1}^{\infty} r^{q + 2l_{2}} P\left( \left\|\Zrv \right\|^{2} > r \right) dr\\ 
            &\lesssim \exp(-c n^{\beta - \gamma})\\
    \end{split}
\end{equation*}
for any $\gamma > 0$.
Therefore,
\begin{equation*}
    \begin{split}
        \left\| \polfz \indicator_{\Zrv \in \Uset{\Z}^{\comp}} \right\|_{\Ell_2(\prob_X)} 
        &= \left\| \ftrue(\X)^\top (K + \lambda I_n)^{-1} \mvec_{\Zrv} \indicator_{\Zrv \in \Uset{\Z}^{\comp}} \right\|_{\Ell_2(\prob_X)}\\
        &\lesssim \left\| \sum_{i=1}^{n} \mvec_{\Zrv,i} \indicator_{\Zrv \in \Uset{\Z}^{\comp}} \right\|_{\Ell_2(\prob_X)} \rightarrow 0 \quad a.s.,
    \end{split}
\end{equation*}
where the above inequality follows from the fact that the ground truth is bounded, the smallest eigenvalue of the kernel is lower bounded by a positive non-zero constant and Lemma \ref{lm:innerpr}. We can now use this fact to complete the proof for the second point in Theorem \ref{prop:main_thm_ext}, i.e. that   
$\left\|\EEobs \fhatridge - \polyf \right\|_{\Ell_2(\prob_X)} \to 0
    ~~ a.s.$,
given that $|\kernf|$ is bounded by some constant. We have
\begin{equation*}
\begin{split}
  \left\| \EEobs \fhatridge - \polyf \right\|_{\Ell_2(\prob_X)}^{2} 
% &=  \EE_{\Zrv} \indicator_{\Zrv \in \Uset{\Z}}(\fubias(\sqrt{\bw}\Zrv) - \polyf_z(\Zrv))^2 + \EE_{\Zrv}\indicator_{\Zrv \in \Uset{\Z}^{\comp}} ( \fubias(\sqrt{\bw}\Zrv) - \polyf_z(\Zrv))^2 \\
%   &\lesssim \EE_{\Zrv} \indicator_{\Zrv \in \Uset{\Z}}(\fubias(\sqrt{\bw}\Zrv) - \polyf_z(\Zrv))^2 
%   + \EE_{\Zrv}\indicator_{\Zrv \in \Uset{\Z}^{\comp}} ( \fubias(\sqrt{\bw}\Zrv))^2 + \EE_{\Zrv}\indicator_{\Zrv \in \Uset{\Z}^{\comp}} ( \polfz(\Zrv))^2 \\
  \lesssim \EE_{\Zrv} \indicator_{\Zrv \in \Uset{\Z}}(\fubias(\sqrt{\bw}\Zrv) - \polyf_z(\Zrv))^2 
  + n^2 P(\Uset{\Z}^{\comp})  + \EE_{\Zrv}\indicator_{\Zrv \in \Uset{\Z}^{\comp}} ( \polfz(\Zrv))^2 \to 0~~a.s.,
  \end{split}
\end{equation*}
where we have used in the second inequality the assumption that the kernel $k$ is bounded. Thus, we can conclude the second part of the proof. \\

% 

% \begin{equation*}
%     \|(K + \lambda I_n)^{-1} (\kvec - \mvec_{\Zrv}) \|_2 \leq c (\|\kvec \|_{2} + \|\mvec_{\Zrv}\|_{2}) \lesssim \sqrt{n}
% \end{equation*}
% Therefore, conditional on $E_{n}$,
% \begin{align}
%     \|(K + \lambda I_n)^{-1} (\kvec - \mvec_{\Zrv}) \|_{L^{2}(P_{\Zrv})} &\lesssim \sqrt{n} \left(n^{-\beta/2} (\log n)^{(1+\epsilon)/2}\right)^{\mc+1} P(\tilde{E_{n}} | E_{n}) + \sqrt{n} (1 - P(\tilde{E_{n}} | E_{n}))\\
%     &\lesssim \sqrt{n} \left(n^{-\beta/2} (\log n)^{(1+\epsilon)/2}\right)^{\mc+1} + n^{2} \exp(-c(\log (n+1))^{(1 + \epsilon)/2} \rightarrow 0
% \end{align}
% Furthermore, due to Proposition \ref{lm:elkarouiextension} and the fact that $\lambda_{min}(K + \lambda I_n)\geq c >0 ~~a.s.$, we get that 
% \begin{equation*}
%     \|(K + \lambda I_n)^{-1} - (M + \lambda I_n)^{-1}\|_2 \to 0~~a.s.
% \end{equation*}
% where $M$ is from Proposition \ref{lm:elkarouiextension}. \\
% Finally, note $P(E^{c}_{n}) \leq n\exp(-c(\log (n+1))^{(1 + \epsilon)/2}$, applying Borel–Cantelli lemma, we get that
% \begin{equation*}
%     \| (\lambda \In + K)^{-1} \kvec  - (\lambda \In + M)^{-1} \mvec_{\Zrv}\|_{L^{2}(P_{\Zrv})} \rightarrow 0 \quad a.s.
% \end{equation*}

\textbf{Step 3:} 
Let $\fstarz$ be the function implicitly defined by $\fstarz(\Zrv) = \fstar(\Xrv)$. Since $\fhatridge$ only depends linearly on the observations $\y$, we have
\begin{equation*}
    \Bias(\fhat) =  \EE_{\Zrv}( \fstarz(\Z)^\top (K + \lambda \In)^{-1} \kvec - \fstarz(\Zrv) )^2 =\EE_{\Zrv} ( \fubias(\sqrt{\bw}\Zrv) - \fstarz(\Zrv) )^2 , 
\end{equation*}
and based on the previous two steps of this proof, we know that, 
\begin{equation*}
 \underset{\Zrv \in \Uset{\Z}}{\max} ~ \left| \polfz(\Zrv) - \fubias(\sqrt{\Zrv}) \right| = \underset{\Zrv \in \Uset{\Z}}{\max} ~ \left| \polfz(\Zrv) -\fstarz(\Z)^\top (K + \lambda \In)^{-1} \kvec \right| \to 0 ~~a.s..
\end{equation*}
As a result, we can conclude that for any $\gamma_1 >0 $ and $n$ sufficiently large, 
\begin{equation*}
   \EE_{\Zrv} \indicator_{\Zrv \in \Uset{\Z}} \left( \fstarz(\Z)^\top (K + \lambda \In)^{-1} \kvec - \fstarz(\Zrv) \right)^2  \gtrsim \EE_{\Zrv}\indicator_{\Zrv \in \Uset{\Z}} \left( \polfz(\Zrv) - \fstarz(\Zrv) \right)^2   - \gamma_1 ~~a.s.,
\end{equation*}
where we have used that 
Furthermore, we now from the previous step that $\EE_{\Zrv}\indicator_{\Zrv \in \Uset{\Z}^{\comp}} (\polfz(\Zrv))^2 \to 0$ and furthermore because $\ftrue$ is bounded by assumption,  we have $\EE_{\Zrv}\indicator_{\Zrv \in \Uset{\Z}^{\comp}} (\polfz(\Zrv) - \fstarz(\Zrv))^2 \to 0$. Hence, for any $\gamma_2 >0$, 
% \makegray{
% \begin{equation*}
% \begin{split}
% &\EE_{\Zrv}\indicator_{\Zrv \in \Uset{\Z}} \left( \polfz(\Zrv) - \fstarz(\Zrv) \right)^2   - \gamma_1 ~~a.s. \\
%    \geq &\EE_{\Zrv}\indicator_{\Zrv \in \Uset{\Z}} \left( \polfz(\Zrv) - \fstarz(\Zrv) \right)^2  
% + \EE_{\Zrv}\indicator_{\Zrv \in \Uset{\Z}^{\comp}} \left( \polfz(\Zrv) - \fstarz(\Zrv) \right)^2 - \gamma_1 - \gamma_2 ~~a.s.
% \\
% &= \EE_{\Zrv} \left( \polfz(\Zrv) - \fstarz(\Zrv) \right)^2  -\gamma_1 - \gamma_2 ~~a.s.
% \end{split}
% \end{equation*}}
\begin{equation*}
    \begin{split}
        \Bias(\fhat) 
        &\gtrsim \EE_{\Zrv}\indicator_{\Zrv \in \Uset{\Z}} \left( \polfz(\Zrv) - \fstarz(\Zrv) \right)^2 - \gamma_1\\
        &\gtrsim \EE_{\Zrv}\indicator_{\Zrv \in \Uset{\Z}} \left( \polfz(\Zrv) - \fstarz(\Zrv) \right)^2  
+ \EE_{\Zrv}\indicator_{\Zrv \in \Uset{\Z}^{\comp}} \left( \polfz(\Zrv) - \fstarz(\Zrv) \right)^2 - \gamma_1 - \gamma_2\\
        &= \EE_{\Zrv} \left( \polfz(\Zrv) - \fstarz(\Zrv) \right)^2  -\gamma_1 - \gamma_2 \quad a.s.
    \end{split}
\end{equation*}

Hence, the result follows by definition of the infimum. 

\qed

%% PROP %%

\subsection{Proofs for the lower bound of the eigenvalues}
\label{sec:PropB1}

\subsubsection{Proof of Proposition \ref{prop:EVlowerbound}}
\label{sec:proofa1toa3}
The proof follows straight forwardly from the following Lemma \ref{lm:elkarouiextension} which gives an asymptotic description of the kernel matrix $K$ based on a similar analysis as the ones used in the proof of Theorem~2.1 and 2.2 in \cite{ElKaroui10}. In essence, it is again a consequence of the concentration inequality from Lemma \ref{lm:innerpr} and the stronger Assumption \Akone~ and in particular the power series expansion of $g$. We denote with $\circ i$ the $i$-times Hadamard product, then

\begin{lemma}
\label{lm:elkarouiextension}
% Assume that the kernel $\kernf$, respectively its restriction onto the hyper sphere $\kernfuncressphere{d}$, satisfies assumptions \Ckone~ and the distribution $\prob_X$ satisfies \Bdone-\Bdtwo. In addition, assume that the map $x \to g(x,x,x)$ is Lipschitz continuous in a neighborhood of $1$ (extension of assumption \Aktwo~ to general $1$) and assume that for any $\xk \in   \convergesetres{\delta}{\delta'}$ (as in assumption \Ckone), the power series from Equation \eqref{eq:kerneldefgap} can be extended to $g(\|\xk\|_2^2,\|\xk\|_2^2, \xk^\top\xk)$, i.e. $g(\|\xk\|_2^2,\|\xk\|_2^2, \xk^\top\xk) = \sum_{i=0}^{m} (\xk^\top\xkd)^i g_i(\|\xk\|_2^2,\|\xk\|_2^2) +(\xk^\top\xkd)^{m+1} \reminder(\|\xk\|_2^2,\|\xk\|_2^2, \xk^\top\xk) $. Furthermore, assume that any $g_j$ is a positive semi-definite kernel function. 

Assume that the kernel $\kernf$, respectively its restriction onto the hyper sphere $\kernfuncressphere{d}$, satisfies Assumption \Akone-\Akthree~ and the distribution $\prob_X$ satisfies \Bdone-\Bdtwo.
% In addition, assume that the map $x \to g(x,x,x)$ is Lipschitz continuous in a neighborhood of $1$ (extension of assumption \Aktwo~ to general $\cbw$) and assume that for any $\xk \in   \convergesetres{\delta}{\delta'}$ (as in assumption \Ckone), the power series from Equation \eqref{eq:kerneldefgap} can be extended to $g(\|\xk\|_2^2,\|\xk\|_2^2, \xk^\top\xk)$, i.e. $g(\|\xk\|_2^2,\|\xk\|_2^2, \xk^\top\xk) = \sum_{i=0}^{m} (\xk^\top\xkd)^i g_i(\|\xk\|_2^2,\|\xk\|_2^2) +(\xk^\top\xkd)^{m+1} \reminder(\|\xk\|_2^2,\|\xk\|_2^2, \xk^\top\xk) $. Furthermore, assume that any $g_j$ is a positive semi-definite kernel function. 
Then, for $m = \floor{2/\beta}$,
  \begin{equation*}
    \opnorm{ K - M} \to 0 ~~~ a.s.
\end{equation*}  
with
\begin{equation}
\label{eq:elkarouiM}
\begin{split}
    \mmat&= \idmat\left(g(\cbw,\cbw,\cbw)  - \sum_{i =0}^m \cbw^i g_i(\cbw,\cbw) \right) +  \sum_{i=0}^m (\Z^\top\Z)^{\circ i} \circ \kermat_{g_i},
\end{split}
\end{equation}
where $\kermat_{g_l}$ is a positive semi-definite matrix with entries $\kermat_{g_l,i,j} = g_l(\| z_i \|_2^2, \| z_j\|_2^2)$.
\end{lemma}

The proof of Proposition \ref{prop:EVlowerbound} follows then immediately when using Schur's product theorem which shows that 
\begin{equation*}
 \idmat\left(g(\cbw,\cbw,\cbw)  - \sum_{i =0}^m \cbw^i g_i(\cbw,\cbw) \right) +  \sum_{i=0}^m (\Z^\top\Z)^{\circ i} \circ \kermat_{g_i} \succeq \idmat\left(g(\cbw,\cbw,\cbw)  - \sum_{i =0}^m \cbw^i g_i(\cbw,\cbw) \right)
\end{equation*}
where we use that $g_i$ is positive semi-definite by Assumption \Akone. 
 In particular, $g(\cbw,\cbw,\cbw)  - \sum_{i =0}^m \cbw^i g_i(\cbw,\cbw) > 0$ because by assumption there exists $\jthresh > \floor{2/\beta}$ such that $g_{\jthresh}(\cbw,\cbw) >0$ and because the positive semi-definiteness of $g_i$ implies that $g_i(\cbw,\cbw) \geq0$.
 \qed

% 
% \begin{lemma}
% \label{lm:elkarouiextension}
% Assume that the kernel $\kernf$, respectively its restriction onto the hyper sphere $\kernfuncressphere{d}$, satisfies the assumptions \Ckone-\Cktwo and \Aktwo. Then, for $m = \floor{2/\beta}$, the following results hold for any of the marginal distributions $\prob_X \in \probsetcov$ and $\prob_X \in \probsetsphere$
%   \begin{equation*}
%     \| K - M\|_2 \to 0 ~~~ a.s.
% \end{equation*}  
% with
% \begin{equation*}
% \label{eq:elkarouiM}
% \begin{split}
%     \mmat&= \idmat\left(\kernf(\ev_1,\ev_1)  - \sum_{i =0}^m g_i(1,1) \right) +  \sum_{i=0}^m (\Z^\top\Z)^{\circ i} \circ \left[
% \sum_{j =0}^{m-i} \sum_{q = 0}^{j}  \frac{g_{i}^{(q,j-q)}(1,1)}{q!(j-q)!} \psi^{\circ k} (\psi^{\circ (m-k)})^\top \right].
% \end{split}
% \end{equation*}
% \end{lemma}

\begin{proof}[Proof of Lemma \ref{lm:elkarouiextension}]
As in \cite{ElKaroui10}, we separately analyze the off and on diagonal terms of $K$. Let $A$ be the off diagonal matrix of $K$, with diagonal entries $A_{i,j} = (1- \delta_{i,j}) K_{i,j}$ and let $D$ be the diagonal matrix of $K$ with entries $D_{i,j} = \delta_{i,j} K_{i,j}$. We have
\begin{align}
    \forall i ~~ D_{i,i} &:= K_{i,i} = g(\|\z_i\|_2^2, \|\z_i\|_2^2,\z_i^\top\z_i), \\
    \forall i\neq j ~~ A_{i,j} &:= K_{i,j} = g(\|\z_i\|_2^2, \|\z_j\|_2^2,\z_i^\top\z_j).
\end{align}

% Recall that due to Lemma \ref{lm:E1}, we can also write $g$ as in Equation \eqref{eq:kerneldefgap} with $\reminder(\cbw,\cbw,\cbw) = \sum_{j=m+1}^{\infty} \cbw^j g_j(\cbw,\cbw) >0$. In particular, $\reminder$ is a continuous and positive semi-definite function in the neighborhood of $(\cbw,\cbw)$. 

Furthermore, we have already seen in Remark \ref{rm:AC_concentration} that as $n \rightarrow \infty$, $(z_{i}, z_{j}) \in \convergesetres{\delta}{\delta'}~~a.s.$ for $1 \leq i \leq j \leq n$. 
   
% Then, we can write
% express $A$ asymptotically using the Taylor series expansion of $g_i$ around the point $(1,1)$: 
% \begin{equation*}
%     \begin{split}
%     \forall i\neq j ~~ A_{i,j} 
%     &=  \sum_{q=0}^{m} (\z_i^\top\z_j)^q g_q(\|\z_i\|_2^2,\|\z_j\|_2^2) 
%     +(\xind{i}^\top \xind{j})^{m+1} \reminder(\|\xind{i}\|_2^2, \|\xind{j}\|_2^2, \xind{i}^\top \xind{j})\\
%     &= \sum_{q =0}^m (\z_i^\top\z_j)^{q} \sum_{ l_1+l_2 \leq m-q} \frac{ g_{q}^{(l_1,l_2)}(1,1)}{l_1
%     ! l_2!} (\z_i^\top\z_i -1 )^{l_1} (\z_j^\top\z_j -1 )^{l_2}   \\ 
%     &+ \sum_{q =0}^{m}(\z_i^\top\z_j)^{q} \sum_{ l_1+l_2  = m+1-q} \frac{ g_{q}^{(l_1,l_2)}(\eta^{q,i,j}_{l_1,l_2})}{l_1
%     ! l_2!} (\z_i^\top\z_i -1 )^{l_1} (\z_j^\top\z_j -1 )^{l_2}   \\ 
%     &+(\xind{i}^\top \xind{j})^{m+1} \reminder(\|\xind{i}\|_2^2, \|\xind{j}\|_2^2, \xind{i}^\top \xind{j}).
%     % %     &+ (\z_i^\top\z_j)^{q+1} \sum_{m =q+1}^{\infty}  (\z_i^\top\z_j)^{m-(q+1)} g_{m}(\|\z_i\|_2^2,\|\z_j\|_2^2)    ~~ a.s.
%         \end{split}
% \end{equation*}
% where $\eta^{q,i,j}_{l_1,l_2}$ are contained in the closed ball $\eta^{q,i,j}_{l_1,l_2} \in B_r((1,1))$ around the point $(1,1)$ with radius $r^2 = (\|\z_i\|_2^2-1)^2 + (\|\z_j\|_2^2-1)^2 \to 0~~a.s.$, where the convergence to zero is by Lemma \ref{lm:innerpr}. Hence, using the fact that $g_i$ is $\mc+1-i$-times continuously differentiable,  we can see that $g_{q}^{(l_1,l_2)}(\eta^{q,i,j}_{l_1,l_2})$ is almost surely bounded by some constant. \\
Let $ M_A$ be the off diagonal matrix with entries
% \begin{equation*}
%     \forall i\neq j ~~~ (M_A)_{i,j} := \sum_{q =0}^\mc (\z_i^\top\z_j)^{q} \sum_{ l_1+l_2 \leq \mc-q} \frac{ g_{q}^{(l_1,l_2)}(1,1)}{l_1
%     ! l_2!} (\z_i^\top\z_i -1 )^{l_1} (\z_j^\top\z_j -1 )^{l_2} . 
% \end{equation*}
\begin{equation*}
    \forall i\neq j ~~~ (M_A)_{i,j} := \sum_{q =0}^\mc (\z_i^\top\z_j)^{q} g_q(\|z_i\|_2^2,\| z_j\|_2^2).
\end{equation*}
We have
\begin{equation*}
    \opnorm{ M_A - A} \leq \| M_A - A\|_F \leq n \underset{i,j}{\max} |M_{A,i,j} - A_{i,j} | \lesssim n\underset{i,j}{\max}| (\z_j^\top\z_j -1 )^{m+1} | \to 0 \quad a.s.,
\end{equation*}
where we have used the fact that the reminder $\reminder$ is bounded by a constant in a neighborhood of $(\cnbw,\cnbw,0)$ which follows from the continuity of $\reminder$. Furthermore, we have used the fact that $(m+1) \beta/2 > 1$.

Next, let 
\begin{equation*}
    M_D := \left[g(\cbw, \cbw, \cbw) - \sum_{q=0}^m \cbw^q g_q(\cbw, \cbw)~ +  \sum_{q=0}^m (\z_i^\top \z_j)^q g_q(\|\z_i\|_2^2,\| \z_j\|_2^2) \right] \mathrm{I}_n
\end{equation*} Because $D-M_D$ is a diagonal matrix,
\begin{equation*}
\begin{split}
    \opnorm{ D - M_D}&= \max_{i} \left|g(\| \z_i\|_2^2, \| \z_i\|_2^2,\z_i^\top\z_i) - 
    g(\cbw, \cbw, \cbw) - \sum_{q=0}^m \cbw^q g_q(\cbw, \cbw)~ +  \sum_{q=0}^m (\z_i^\top \z_j)^q g_q(\|\z_i\|_2^2,\| \z_j\|_2^2)\right|
        \\
    &\leq \underbrace{\delta_L \sqrt{3} (\| \z_i\|_2^2 -\cbw)}_{T_1} + \sum_{q=0}^m\underbrace{[(\z_i^\top \z_j)^q - \cnbw^q] g_q(\|\z_i\|_2^2,\| \z_j\|_2^2)}_{T_2} \\
    &+\sum_{q=0}^m\underbrace{[\cnbw^q - \cbw^q] g_q(\|\z_i\|_2^2,\| \z_j\|_2^2)}_{T_3}+ \underbrace{\cbw^q [ g_q(\|\z_i\|_2^2,\| \z_j\|_2^2) - g_q(\cbw, \cbw)]}_{T_4} 
\end{split}
\end{equation*}
where we have used that by assumption $g$ is $\delta_L$-Lipschitz continuous on the restriction $\{(x,x,x) | x \in [1-\delta, 1+ \delta]\} \subset \Omega$ for some $\delta_L >0$. Clearly $T_1 \to 0$ and $T_3 \to 0$ due to Lemma \ref{lm:innerpr} and because $\cnbw \to \cbw$. Furthermore, we know that for any $q \leq m$, $g_q$ is continuously differentiable by Assumption \Ckone~ and hence is also Lipschitz continuous in a closed ball around $(\cbw,\cbw)$. Hence, we can show that $T_4 \to 0$. The only thing left to show that  $ \opnorm{ D - M_D} \to 0 \quad a.s.$ and hence to conclude the proof is to show that $T_3 \to 0$. However, this follows from the following claim:
\\

\textbf{Claim:} \textit{For any $\epsilon>0$ and any $q>0$,
\begin{equation*}
 \underset{i}{\max}~ \left| \frac{(\x_i^\top \x_i)^q}{ (\trace(\Sigma_d))^q} - 1 \right| \leq  c_q\max[n^{-\beta/2} (\log(n))^{(1+\epsilon)/2}, n^{-q\beta/2}(\log(n))^{q((1+\epsilon)/2)}] \quad a.s.
 \end{equation*}
where $c_q$ is a constant only depending on $q$.}
\\\\

\textbf{Proof of the claim:}
Due to Lemma \ref{lm:innerpr}, for every $q>0$
\begin{equation*}
 \underset{i}{\max}~ \left| \left[\frac{(\x_i^\top \x_i)}{\trace(\Sigma_d)} - 1\right]^q \right| \leq ( n^{-\beta/2} (\log(n))^{(1+\epsilon)/2})^q.
 \end{equation*}
We proof the the claim by induction. The case where $q=1$ holds trivially with $c_q = 1$. For $q>1$, 
\begin{equation*}
    \underset{i}{\max}~  \left| \left[\frac{(\x_i^\top \x_i)}{\trace(\Sigma_d)} - 1\right]^q \right| =  \underset{i}{\max}~  \left| \frac{(\x_i^\top \x_i)^q}{ (\trace(\Sigma_d))^q} + \sum_{j=1}^q (-1)^j {q \choose j }  \left(\frac{\x_i^\top \x_i}{\trace(\Sigma_d)}\right)^{q-j}\right| \leq  (n^{-\beta/2} (\log(n))^{(1+\epsilon)/2})^q.
\end{equation*} 
Next, by induction, $ \underset{i}{\max}~ \left| \frac{(\x_i^\top \x_i)^q}{ (\trace(\Sigma_d))^q} - 1 \right| \leq  c_1\max\left[n^{-\beta/2} (\log(n))^{(1+\epsilon)/2}, n^{-q\beta/2}(\log(n))^{q((1+\epsilon)/2)}\right]$. Furthermore, $\sum_{j=1}^q(-1)^j {q\choose j} = -1$, which shows that
\begin{equation*}
\begin{split}
 &\underset{i}{\max}~ \left| \frac{(\x_i^\top \x_i)^q}{ (\trace(\Sigma_d))^q} + \sum_{j=1}^q (-1)^j {q \choose j } \left( \frac{(\x_i^\top \x_i)^q}{ (\trace(\Sigma_d))^q}\right)^{q-j} \right| \\ =  &\underset{i}{\max}~ \left| \frac{(\x_i^\top \x_i)^q}{ (\trace(\Sigma_d))^q} + \sum_{j=1}^q (-1)^j {q \choose j } \right[ \left( \frac{(\x_i^\top \x_i)^q}{ (\trace(\Sigma_d))^q}\right)^{q-j} -1 \left]+ \sum_{j=1}^q (-1)^j {q \choose j }  \right|\\
 \leq &\underset{i}{\max}~ \left| \frac{(\x_i^\top \x_i)^q}{ (\trace(\Sigma_d))^q} -1 \right| + \sum_{j=1}^q {q \choose j }  c_j\max\left[n^{-\beta/2} (\log(n))^{(1+\epsilon)/2}, n^{-j\beta/2}(\log(n))^{j((1+\epsilon)/2)}\right].
 \end{split}
 \end{equation*}
 Hence, combining these two results, 
 \begin{equation*}
      \underset{i}{\max}~ \left| \frac{(\x_i^\top \x_i)^q}{ (\trace(\Sigma_d))^q} -1\right| \leq (n^{-\beta/2} (\log(n))^{(1+\epsilon)/2})^q + \sum_{j=1}^q {q \choose j }  c_j\max \left[n^{-\beta/2} (\log(n))^{(1+\epsilon)/2}, n^{-j\beta/2}(\log(n))^{j((1+\epsilon)/2)} \right],
 \end{equation*}
which completes the induction and thus the proof.

\end{proof}

\subsubsection{Proof of Proposition \ref{prop:alphaexp}}
\label{sec:proofalphaexp}
We use again the notation $z_i = \frac{1}{\sqrt{\bw}} \x_i$ and $\Zrv = \frac{1}{\sqrt{\bw}} \Xrv$ and $\Zs = \frac{1}{\sqrt{\bw}} \Xs$.
In addition, define $D^{\alpha}$ to be the $n\times n$ matrix with entries $D^{\alpha}_{i,j} = d_{\alpha}(z_i, z_j) := \| z_i - z_j \|_2^{\alpha}$.

We start with a well known technical lemma 
\begin{lemma}
\label{lm:usefulint}
For all $t\geqslant0$ and $0<\alpha<2$,
\begin{equation*}
    t^{\alpha}=c_\alpha\int_0^\infty(1-e^{-t^2x^2})x^{-1-\alpha}\df x
\end{equation*}
with 
\begin{equation*}
    c_\alpha:=\left(\int_0^\infty(1-e^{-x^2})x^{-1-\alpha}\df x\right)^{-1}>0.
\end{equation*}
\end{lemma}
\begin{proof} For $t=0$, the integral is zero. So it is true. We only need to prove for the case when $t>0$. First, use $1-e^{-t^2x^2}\leqslant t^2x^2$ to imply that the integral exists:
\begin{equation*}
    0\leqslant\int_0^\infty(1-e^{-t^2x^2})x^{-1-\alpha}\df x\leqslant\int_0^1t^2x^{1-\alpha}+\int_1^\infty x^{-1-\alpha}\df x<\infty.
\end{equation*}
Substitute $y:=tx$, so $t^{-1}\df y=\df x$.
\begin{align*}
    \int_0^\infty(1-e^{-t^2x^2})x^{-1-\alpha}\df x &=\int_0^\infty(1-e^{-y^2})y^{-1-\alpha}t^{1+\alpha}t^{-1}\df y\\
    &=t^{\alpha}\int_0^\infty(1-e^{-y^2})y^{-1-\alpha}\df y.
\end{align*}
Hence, the result holds.
\end{proof}

\begin{lemma}
\label{lm:alphaexpbound}
Assume that $\prob_X$ satisfies the Assumption \Bdone-\Bdtwo. The eigenvalues of $D^{\alpha}$ are bounded away from zero by a positive non-zero constant $c>0$ independent of $n$, i.e. $\underset{i \leq n}{\min} \left|\lambda_i(D^{\alpha}) \right| \geq c$. 
\end{lemma}

\begin{proof}[Proof of Lemma \ref{lm:alphaexpbound}]
Apply Lemma \ref{lm:usefulint} to $t:=\Vert z_i-z_j\Vert_2^\alpha\geqslant0$:
$$\Vert z_i-z_j\Vert_2^\alpha=c_\alpha\int_0^\infty(1-e^{-x^2\Vert z_i-z_j\Vert_2^2})x^{-1-\alpha}\df x$$
Take any $\mu \in\mathbb{R}^n$ with $\sum_{1\leqslant i\leqslant n}\mu_i=0$. Then, 
 \begin{align*}
    \mu^\top D^{\alpha} \mu = \sum_{1\leqslant i,j\leqslant n}\Vert z_i-z_j\Vert_2^\alpha\mu_i\mu_j & = \sum_{1\leqslant i,j\leqslant n}\mu_i\mu_jc_\alpha\int_0^\infty(1-e^{-x^2\Vert z_i-z_j\Vert_2^2})x^{-1-\alpha}\df x\\
    & = -c_\alpha\int_0^\infty x^{-1-\alpha} \sum_{1\leqslant i,j\leqslant n}\mu_i\mu_j e^{-x^2\Vert z_i-z_j\Vert_2^2}\df x.
\end{align*}
Next, note that the $\alpha$-exponential kernel with $\alpha=2$
(i.e. the Gaussian kernel) satisfies Assumptions \Akone-\Akthree~ since
$\exp(-\|\xk-\xkd\|_2^2) = \sum_{j=0}^{\infty} \frac{2^j}{j!}
(\xk^\top \xkd)^j \exp(-\|\xk\|_2^2 - \|\xkd\|_2^2)$. Hence, we can conclude from Proposition \ref{prop:EVlowerbound} that the minimum eigenvalue $\lambda_{min}(K) \geq c_G > 0$ of the
kernel matrix $\kermat$ of the Gaussian kernel is lower bounded
 by some positive non-zero constant
independent of $n$. Hence, for every $x \in
\mathbb{R}_+$, $\sum_{1\leqslant i,j\leqslant n}\mu_i\mu_j
e^{-x^2\Vert z_i-z_j\Vert_2^2} \geq \| \mu \|_2^2 c_{G,x} > 0$. Where $c_{G,x}$ is
some positive constant independent of $n$. Thus, we can conclude that
there exists a constant $\tilde{c} >0 $ independent of $n$, such that
\begin{equation}
\label{eq:eqalphaexpbound}
    \mu^\top D^{\alpha} \mu \leq -\tilde{c}\| \mu \|_2^2.
\end{equation}

Because the set of vectors $\mu^T1 = 0$ span a $n-1$ dimensional subspace, we can apply the Courant–Fischer–Weyl min-max principle. Hence, we can see that the second large eigenvalue of the matrix $D^{\alpha}$ satisfies
$\lambda_{n-1} < -\tilde{c}$. Since the sum of the eigenvalues
$\sum_{i=1}^{n} \lambda_{i} = \trace(D^{\alpha}) = 0$, $\lambda_{n} > \tilde{c}$, which concludes the proof.
\end{proof}

For simplicity, we show that the result holds true for $\cbw =
1$. The general case then follows immediately from the proof. We note that we already know from Lemma \ref{lm:alphaexpbound} that
the eigenvalues of the matrix $D^{\alpha}$ are all bounded away from
zero by some constant $c_{\alpha} >0$ independent of $n$. The proof heavily makes use of this fact. We separate the remaining proof into three steps. In a first step we
construct a positive semi-definite kernel $\tilde{k}$ such that both
\begin{equation*}
 \exp(-\lvert\lvert \xk-\xkd\rvert\rvert_2^{\alpha}) =
\exp(\tilde{k}(\xk,\xkd)) \exp(-\lvert\lvert
\xk-\xkd\rvert\rvert_2^{\alpha} - \tilde{k}(\xk,\xkd)) 
\end{equation*}
and
$\exp(-\lvert\lvert \xk-\xkd\rvert\rvert_2^{\alpha} -
\tilde{k}(\xk,\xkd))$
are positive semi-definite function with a kernel matrix $A$ which has lower bounded eigenvalues when evaluating at $\Zs$. 
Step 2 and 3 then proof the proposition based on the results from step 1. 
% Then, we show
% that the eigenvalues of the kernel matrix of
% $\exp(\tilde{k}(\xk,\xkd))$ are lower bounded and finally, in a last
% step, we show that this implies that the eigenvalues of the kernel
% matrix of $\exp(-\lvert\lvert \xk-\xkd\rvert\rvert_2^{\alpha})$ are
% lower bounded. \\\\ 
\\

\textbf{Step 1:} 
%Let $d_{\alpha}(\xk,\xkd) =
%\lvert\lvert \xk-\xkd\rvert\rvert_2^{\alpha}$. 
% We know from Chapter~3
% Theorem~2.2 \cite{Berg84} that this is a conditionally negative
% definite function, i.e. for every $v \in \mathbb{R}^n$ with $1^\top v =
% 0$, $v^\top D^{\alpha}v \leq 0$.
We know from Chapter~3
Theorem~2.2 in \cite{Berg84} that this is a conditionally negative
definite function, i.e. for every $v \in \mathbb{R}^n$ with $1^\top v =
0$, $v^\top D^{\alpha}v \leq 0$.
A function is called conditionally negative if for any $m\in \NN\setminus 0$ and any $\{x_1,...,\x_m\}$, the corresponding kernel matrix $A$ is conditionally negative, i.e. for any $v \in \mathbb{R}^m$ with $v^T 1 = 0$,  $v^T A v \leq 0$.
As shown in Chapter~3 Lemma~2.1
in \cite{Berg84}, a kernel function $\phi(\xk,\xkd)$ is conditionally
negative definite, if and only if for any $z_0$, 
\begin{equation*}
 (\xk,\xkd) \to  \phi(\xk,\z_0) +
\phi(\z_0,\xkd) -\phi(\xk,\xkd) - \phi(\z_0,\z_0)
\end{equation*}
is a positive semi-definite
function. Hence, for any $\z_0$, the kernel defined by 
$(\xk,\xkd) \to  d_{\alpha}(\xk,\z_0) +
d_{\alpha}(\z_0,\xkd) -d_{\alpha}(\xk,\xkd) - d_{\alpha}(\z_0,\z_0)$
 is positive semi-definite. 
% 
% 
% Let $A$ be the corresponding kernel matrix
% evaluated at $\Zs$ and let $\z_0$ be some additional vector in $\RR^n$. It is shown in the proof of Chapter~3 Lemma~2.1
% \cite{Berg84} that for any $v \in \mathbb{R}^n$,
% \begin{equation*}
%      - v^\top A v = 
%      \begin{pmatrix}
%      v^\top & - 1^\top v
%      \end{pmatrix} 
%      \begin{pmatrix} 
%      D^{\alpha} & d_{\alpha}(\Zs, \z_0) \\ 
%      d_{\alpha}(\Zs, \z_0)^\top & d_{\alpha}(\z_0,\z_0) 
%      \end{pmatrix}
%      \begin{pmatrix}
%      v \\ 
%      - 1^\top v
%      \end{pmatrix} 
%      \leq 0
% \end{equation*}
% 
% where $d_{\alpha}(\Zs,\z_0)$ is the vector with entries
% $d_{\alpha}(\Zs,\z_0)_i = d_{\alpha}(\z_i,\z_0)$. Note that inequality
% $\leq 0$ follows from the fact that $d_{\alpha}$ is conditionally
% negative definite and $1^\top \begin{pmatrix}v \\ - 1^\top v\end{pmatrix} =
%   0$.  
  
The goal is now to construct a kernel $\tilde{k}$ based on this idea such that the eigenvalues of the corresponding kernel matrix $A$ can be lower bounded by a positive non-zero constant. We can use the same argument as used in Lemma \ref{lm:innerpr} to show that there exists almost surely over the draws of $\Zs$ an additional vector $z_0$ such that for any two vectors $\zk,\zkd \in \Zs \cup\{\z_0\}$, 
\begin{equation}
\label{eq:tmpconineq}
    | \zk^\top \zkd - \delta_{\zk = \zkd} | \lesssim n^{-\beta/2} (\log(n))^{(1+\epsilon)/2} \quad a.s.
\end{equation}
Hence, for any two vectors $\xk,\xkd \in \RR^n$, we can define
\begin{equation*}
 \tilde{k}(\xk,\xkd) =  d_{\alpha}(\xk,\z_0) +
d_{\alpha}(\z_0,\xkd) -d_{\alpha}(\xk,\xkd) - d_{\alpha}(\z_0,\z_0).
\end{equation*}

Next, it is straight forward to verify that the Equation \eqref{eq:eqalphaexpbound} from Lemma \ref{lm:alphaexpbound} also applies for the matrix 
\begin{equation*}
 D^{\alpha}(\Zs,\z_0) = \begin{pmatrix} 
     D^{\alpha} & d_{\alpha}(\Zs, \z_0) \\ 
     d_{\alpha}(\Zs, \z_0)^\top & d_{\alpha}(\z_0,\z_0) 
     \end{pmatrix}.
\end{equation*}
 Therefore, there exists $\tilde{c}>0$ such that for any $v \in \RR^n$, 
     \begin{equation}
     \label{eq:alpha1}
   \begin{pmatrix} v^{T} &  -1^\top  v\end{pmatrix}   D^{\alpha}(\Zs,\z_0)\begin{pmatrix} v^{T} \\  -1^\top v \end{pmatrix} \leq -c_{\lambda} \| \begin{pmatrix} v^{T} \\  1^\top v \end{pmatrix}\|_2^2,
\end{equation}
where we have used that $1^T \begin{pmatrix} v^{T} \\  -1^\top v \end{pmatrix} = 0$. Next, note that
\begin{equation}
\label{eq:alpha2}
\begin{split}
      &\begin{pmatrix} v^{T} &  -1^\top  v\end{pmatrix}   D^{\alpha}(\Zs,\z_0)
      \begin{pmatrix} v^{T} \\  -1^\top v \end{pmatrix} \\  
                = &v^\top  D^{\alpha} v - v^\top  \left[\frac{1}{n} 1 1^\top D^{\alpha}(\z_0, \Zs) \right] v - v^\top  \left[ \frac{1}{n} D^{\alpha}(\z_0, \Zs)^\top  1 1^\top  \right] v  + v^\top  \left[ \frac{1}{n^2} 1 1^\top  \tilde{D}^{\alpha} 1 1^\top  \right] v. \\ 
                = & v^\top \underbrace{\left[  D^{\alpha}  -  \frac{1}{n} 1 1^\top D^{\alpha}(\z_0, \Zs)   -    \frac{1}{n} D^{\alpha}(\z_0, \Zs)^\top  1 1^\top     +    \frac{1}{n^2} 1 1^\top  \tilde{D}^{\alpha} 1 1^\top   \right]}_{= -A} v,
\end{split}
\end{equation}
where $A$ is the kernel matrix of $\tilde{k}$ evaluated at $\Zs$. 
Hence, when combining Equation \eqref{eq:alpha1} and \eqref{eq:alpha2} we can see that 
\begin{equation*}
 v^T A v \geq \tilde{c}~ (v^Tv + v^T11^Tv) \geq  \tilde{c} ~v^Tv,
\end{equation*}
and hence using the Courant–Fischer–Weyl min-max principle we can see that $A$ has lower bounded eigenvalues $\geq \tilde{c}$. \\

\textbf{Step 2:}
We can write $\exp(-d_{\alpha}(x,\xkd)) = \exp(\tilde{k}(x,\xkd)) \exp(\phi(\xk,\xkd)) $ with $\phi(x,\xkd) := -d_{\alpha}(x,\xkd) - \tilde{k}(x,\xkd) =  d_{\alpha}(\z_0,\z_0)    -d_{\alpha}(x,z_0)  -d_{\alpha}(z_0,\xkd) $. It is straight forward to verify that $\exp(\phi(x,\xkd))$ is a positive semi-definite function. Hence, due to Schur's product theorem, the following sum is a sum of positive semi-definite functions
\begin{equation*}
    \exp(-d_{\alpha}(\xk,\xkd)) = \exp(\tilde{k}(\xk,\xkd)) \exp(\phi(x,\xkd)) = \sum_{l=0}^{\infty} \frac{1}{l!} \tilde{k}(x,\xkd)^l \exp(\phi(x,\xkd)).
\end{equation*} 
 Therefore, it is sufficient to show that the eigenvalues of the kernel matrix $M$ of $\tilde{k}(x,\xkd) \exp(\phi(x,\xkd))$, evaluated at $\Zs$, are lower bounded. Let $B$ be the kernel matrix of $\exp(\phi(x,\xkd))$ evaluated at $\Zs$, we have that $M = A \circ B$, where $\circ$ is the Hadamard product with matrix $A$ from the previous step. 
 We make the following claim from which the proof follows trivially using the fact shown in the first step that the eigenvalues of $A$ are lower bounded by a positive non-zero constant.
\\\\
\textbf{Claim:} \textit{$B = \frac{1}{2\exp(2)} 11^\top  + \tilde{B}$ with $\tilde{B}$ a positive semi-definite matrix.}
\\\\
\textbf{Step 3: Proof of the claim} Let $\psi$ be the vector with entries $\psi_i = \exp(-  d_{\alpha}(\z_i,\z_0))$. Furthermore, let $\gamma = \exp(d_{\alpha}(\z_0, \z_0))$. We can write

\begin{equation*}
    B = \gamma \left(1 \psi^\top \right) \circ \left( \psi 1^\top  \right) = \gamma \psi \psi^\top .
\end{equation*}
Next, using Lemma \ref{lm:innerpr} and the fact that
% Next, due to Equation \ref{eq:tmpconineq}, we can see that 
% \begin{equation*}\label{sumconcentrate}
%     \left| 2^{\alpha/2} - \frac{1}{n^2} \sum_{i,j=1}^{n} d_{\alpha}(\tilde{\z}_i, \tilde{\z}_j)) \right| \leq \frac{(n^2-n) n^{-\beta/2}(\log(n))^{(1+\epsilon)/2} + n}{n^2} \to 0 \quad a.s.
% \end{equation*}
 $d_{\alpha}(x,\xkd) =  2^{\alpha/2} + O(\frac{\lvert\lvert x-\xkd\rvert\rvert_2^2}{2} -1 )$, we can see that $ \gamma \geq \exp( 2^{\alpha/2}/2) >1 ~~a.s.$. Hence, it is sufficient to show that $  \psi \psi^\top  - \frac{1}{2e^{2}} ~ 1 1^\top  $ is positive semi-definite. However, this is true if and only if $1^\top  \psi \psi^\top  1 \geq \frac{1}{2e^{2}} 1^\top 11^\top  1$, which is equivalent to saying that $ \left( \sum_{i=1}^{n} \exp(-d_{\alpha}(\z_i, \z_0)) \right)^{2} \geq \frac{n^2}{2e^{2}}$. However, using again the same argument as for $\gamma$, we can see that $\left|  2^{\alpha/2} -  d_{\alpha}(z_i, \z_0) \right| \to 0 ~~ a.s.$ for any $1 \leq i \leq n$, which completes the proof.
\qed

\subsection{Proof of Corollary \ref{cor:kernels}}
\label{sec:proofcrkernels}

We only show this corollary for the case where $\bw =\effdim$. The general case where $\bw \asymp \effdim$ then follows trivially. First, note that the Assumption \Akone-\Aktwo~straight forwardly hold true for the exponential inner product kernel with $\kernf(\xk,\xkd) = \exp(\xk^\top \xkd) = \sum_{j=0}^{\infty} \frac{1}{j!} (\xk^\top \xkd)^j$ and for the Gaussian kernel with 
\begin{equation*}
 \kernf(\xk,\xkd) = \exp(-\|\xk -\xkd \|_2^2 ) = \sum_{j=0}^{\infty} \frac{2^j}{j!} (\xk^\top \xkd)^j \exp(-\|\xk\|_2^2)\exp(-\|\xkd\|_2^2). 
\end{equation*}
Next, note that the $\alpha$-exponential kernel with $\alpha <2$ is already explicitly covered in Theorem \ref{thm:main_thm}. Hence, the only thing left to show is that Theorem \ref{thm:main_thm} also applies for the Relu-NTK kernel.

We use the definition of the Neural Tangent Kernel presented in \cite{Arora19,Lee18}. Let $L$ be the depth of the NTK and $\sigma: \mathbb{R} \to \mathbb{R}$ the activation function which is assumed to be almost everywhere differentiable. For any $i>0$, define the recursion
\begin{equation*}
  \begin{split}\Sigma^{(0)}(\xk,\xkd) &:= \xk^\top  \xkd \\
\Lambda^{(i)}(\xk,\xkd) &:= \begin{pmatrix} \Sigma^{(i-1)}(\xk,\xk) & \Sigma^{(i-1)}(\xk,\xkd) \\ \Sigma^{(i-1)}(\xk,\xkd) & \Sigma^{(i-1)}(\xkd,\xkd)\end{pmatrix} \\
\Sigma^{(i)}(\xk,\xkd) &:= c_{\sigma} \underset{(u,v) \sim \mathcal{N}(0, \Lambda^{(i)})}{\mathbb{E}}~\left[ \sigma(u) \sigma(v) \right] 
\end{split}
\end{equation*}
with $c_{\sigma} := \left[ \underset{v \sim \mathcal{N}(0, 1)}{\mathbb{E}}~\left[ \sigma(v)^2 \right] \right]^{-1}$. 
Furthermore, define
\begin{equation*}
     \dot{\Sigma}^{(i)} := c_{\dot{\sigma}} \underset{(u,v) \sim \mathcal{N}(0, \Lambda^{(i-1)})}{\mathbb{E}} ~\left[ \dot{\sigma}(u) \dot{\sigma}(v) \right] 
\end{equation*}
with $c_{\dot{\sigma}} := \left[ \underset{v \sim \mathcal{N}(0, 1)}{\mathbb{E}}~\left[ \dot{\sigma}(v)^2 \right] \right]^{-1}$ 
where $\dot{\sigma}$ is the derivative of $\sigma$. The NTK $k_{\textrm{NTK}}$ is then defined as
\begin{equation*}
     k_{\textrm{NTK}}(\xk,\xkd) := \sum_{i=1}^{L+1} \Sigma^{(i-1)}(\xk,\xkd) \prod_{j=i}^{L+1} \dot{\Sigma}^{(j)}(\xk,\xkd). 
\end{equation*}
We call a function $\sigma$ \textit{k-homogeneous}, if for any $\xk \in \mathbb{R}$ and any $a >0$, $\sigma(a\xk) = a^k \sigma(\xk)$. We can now show the following result:

\begin{prop}
\label{prop:ntkass}
Assume that the activation function $\sigma$ is $k$-homogeneous and both the activation function and its derivative posses a Hermite-polynomial series expansion (see \cite{Daniely16}) where there exits $\jthresh \geq 2\floor{2/\beta}$ such that the $\jthresh$-th coefficient $a_{\jthresh} \neq 0$. Then, the NTK kernel satisfies the Assumption \Akone-\Akthree~and hence Theorem \ref{thm:main_thm} applies. 
\end{prop}

In fact, we can easily see that any non linear activation function which is homogeneous and both the activation function and its derivative posses a Hermite polynomial extension satisfies the assumptions in Proposition \ref{prop:ntkass}. In particular, this includes the popular Relu activation function $\sigma(x) = \max(x,0)$ where the explicit expression for the Hermite polynomial extension of the Relu activation function can be found in \cite{Daniely16}.

\subsubsection{Proof of Proposition \ref{prop:ntkass}}

% As a consequence of the $k$-homogeneity of $\sigma$, we can see from Theorem~3.1 \cite{Arora19} that when we restrict $\x$ to the unit ball, i.e. $\lvert\lvert \x \rvert\rvert_2^2$... \mw{Here don't forget to finish it.}

% As a first step of the proof of Proposition \ref{prop:ntkass}, we make the following remark.

We start the proof with the a discussion on existing results in the literature which we use  for this proof. 
First of all, we note that $\dot{\sigma}$ is a $k-1$-homogeneous function and has also a Hermite polynomial extension by assumption. Based on the results shown in Appendix~E.1 in \cite{Arora19}. Hence, due to the homogeneity of $\sigma$ and $\dot{\sigma}$ we can write
\begin{equation}
\label{eq:ntksimp1}
     \Sigma^{(i)}(\x,\xkd) = c_{\sigma} \left(\Sigma^{(i-1)}(\x,\x) \Sigma^{(i-1)}(\xkd,\xkd)  \right)^{k/2}t_{\sigma}\left( \frac{\Sigma^{(i-1)}(\x,\xkd)}{\sqrt{\Sigma^{(i-1)}(\x,\x) \Sigma^{(i-1)}(\xkd,\xkd)}} \right),
\end{equation}
with 
\begin{equation*}
\label{eq:hatsimga}
   t_{\sigma}(\rho) = \underset{(u,v) \sim \mathcal{N}(0, \tilde{\Lambda}(\rho))}{\mathbb{E}}~\left[ \sigma(u) \sigma(v) \right] 
\end{equation*}
and 
$\tilde{\Lambda}(\rho) = \begin{pmatrix} 1& \rho \\ \rho & 1 \end{pmatrix} $. Furthermore, we can similarly write
\begin{equation*}
\label{eq:ntkdotsigma}
    \dot{\Sigma}^{(i)} =c_{\sigma} (\x^\top \x)^{\frac{k^{i-1}(k-1)}{2}}(\xkd^\top \xkd)^{\frac{k^{i-1}(k-1)}{2}} t_{\dot{\sigma}}\left( \frac{\Sigma^{(i-1)}(\x,\xkd)}{(\x^\top \x)^{\frac{k^{i-1}}{2}}(\xkd^\top \xkd)^{\frac{k^{i-1}}{2}}} \right),
\end{equation*}
with $t_{\dot{\sigma}}(\rho) = \underset{(u,v) \sim \mathcal{N}(0, \tilde{\Lambda}(\rho))}{\mathbb{E}}~\left[ \dot{\sigma}(u) \dot{\sigma}(v) \right] $. The function $t_{\sigma}$ is called the dual of the activation function (Definition~4 in \cite{Daniely16}). In particular, since by assumption $\sigma$ and $\dot{\sigma}$ have a Hermite polynomial extension, Lemma~11 in \cite{Daniely16} provides some useful properties for $t_{\sigma}$ and remark that any of the following properties hold also true for $t_{\dot{\sigma}}$:
\begin{enumerate}
    \item Let $a_i \in \mathbb{R}$ be the coefficients of the Hermite polynomial extension of $\sigma$, then $t_{\sigma}(\rho) = \sum_{i=0}^{\infty} a_i^2 \rho^i$
    \item $t_{\sigma}$ is continuous in $[-1,1]$ and smooth in $(-1,1)$
    \item The image of $t_{\sigma}$ is $[-\gamma, \gamma ]$ with $\gamma = \underset{v \sim \mathcal{N}(0, 1)}{\mathbb{E}}~\left[ \sigma(v)^2 \right] = 1/c_{\sigma}$
    \item We have that $t_{\sigma}(1) = \underset{v \sim \mathcal{N}(0, 1)}{\mathbb{E}}~\left[ \sigma(v)^2 \right] = c_{\sigma}$
\end{enumerate}

Based on this discussion, we can now show the following lemma.
\begin{lemma} 
\label{lm:ntk1}
% For any constant scale $\tau_0>0$ and for any for any $\xk, \xkd \neq 0$, we can express $k_{\textrm{NTK},\tau_0}$ as
The NTK $\kernf_{\textrm{NTK}}$ posses a power series expansion
\begin{equation*}
\label{eq:ntk1}
    k_{\textrm{NTK}}(\xk,\xkd) = \sum_{j=0}^{\infty} (\xk,\xkd)^j g_j(\lvert\lvert \xk \rvert\rvert_2^2, \lvert\lvert \xkd \rvert\rvert_2^2),
\end{equation*}
which converges for any $\xk,\xkd \in \RR^d$, $\xk,\xkd \neq 0$. Furthermore, for any $\xk,\xkd \in \RR_+$,
\begin{equation*}
    \label{eq:ntkgi}
    g_j(x,\xkd) = \sum_{i = -\infty}^{\infty} \eta_{j,i} (\xk \xkd)^{i/2}
\end{equation*}
and $\eta_{j,i} \geq 0 $. 
\end{lemma}

\begin{proof}
 In a first step, a closed form expression for $\Sigma^{(i)}(\x,\x)$ is derived. Based on the discussion above and particularly  Equation \eqref{eq:ntksimp1} we can see that
\begin{equation*}
    \Sigma^{(i)}(\x,\x) = \left(\Sigma^{(i-1)}(\x,\x)\right)^k, 
\end{equation*} 
and by induction, we get that
\begin{equation}
\label{eq:ntklipschitz}
    \Sigma^{(i)}(\x,\x) = (\x^\top \x)^{k^i}.
\end{equation}
Therefore, Equation \eqref{eq:ntksimp1} becomes 
\begin{equation*}
\label{eq:ntkproof2}
    \Sigma^{(i)}(\x,\xkd) = c_{\sigma} (\x^\top \x)^{\frac{k^{i-1}}{2}}(\xkd^\top \xkd)^{\frac{k^{i-1}}{2}}t_{\sigma}\left( \frac{\Sigma^{(i-1)}(\x,\xkd)}{(\x^\top \x)^{\frac{k^{i-1}}{2}}(\xkd^\top \xkd)^{\frac{k^{i-1}}{2}}} \right).
\end{equation*} 
The goal is now to show that whenever $\xk,\xkd \neq 0$, $\Sigma^{(i)}(\x,\xkd)$ can be expressed as an sum of the form
\begin{equation*}
\label{eq:ntkgi}
    \begin{split}
        \Sigma^{(i)}(\xk,\xkd) 
        &= \sum_{j=0}^{\infty} (\xk^\top \xkd)^j \sum_{l=-{\infty}}^{\infty} \eta_{j,l}^{(i)} (\lvert\lvert \xk\rvert\rvert_2^2 \lvert\lvert \xkd\rvert\rvert_2^2)^{l/2}
    \end{split}
\end{equation*} 
with $\eta_{j,l}^{(i)} \geq 0$. 
We proof by induction. In a first step, note that the case where $i=0$ holds trivially true.
Next, due to the above discussion, $t_{\sigma}$ can be expressed as a Taylor series around $0$ with positive coefficients $a_i^2$. Thus, 
\begin{equation*}
    \begin{split}
\Sigma^{(i+1)}(\x,\xkd) &= c_{\sigma} (\x^\top \x)^{\frac{k^{i}}{2}}(\xkd^\top \xkd)^{\frac{k^{i}}{2}} \sum_{m=0}^{\infty} a_m^2 \left(\frac{\Sigma^{(i)}(\x,\xkd)}{(\lvert\lvert \xk\rvert\rvert_2^2\lvert\lvert \xkd\rvert\rvert_2^2)^{\frac{k^{i}}{2}}} \right)^m \\
&= c_{\sigma} (\lvert\lvert \x\rvert\rvert_2^2)^{\frac{k^{i}}{2}}(\lvert\lvert \xkd\rvert\rvert_2^2)^{\frac{k^{i}}{2}} \sum_{m=0}^{\infty} a_m^2 \left(\frac{\sum_{j=0}^{\infty} (\x^\top \xkd)^j \sum_{l=-\infty}^{\infty} \eta_{j,l}^{(i)} (\lvert\lvert \xk \rvert\rvert_2^2\lvert\lvert \xkd\rvert\rvert_2^2)^{l/2}}{(\lvert\lvert \xk\rvert\rvert_2^2\lvert\lvert \xkd\rvert\rvert_2^2)^{\frac{k^{i}}{2}}} \right)^m \\
&=c_{\sigma} (\lvert\lvert \x\rvert\rvert_2^2)^{\frac{k^{i}}{2}}(\lvert\lvert \xkd\rvert\rvert_2^2)^{\frac{k^{i}}{2}} \sum_{m=0}^{\infty} a_m^2 \left(\sum_{j=0}^{\infty} (\x^\top \xkd)^j \sum_{l=-\infty}^{\infty} \eta_{j,l}^{(i)} (\lvert\lvert \xk \rvert\rvert_2^2\lvert\lvert \xkd\rvert\rvert_2^2)^{l/2 - k^{i}/2} \right)^m \\
&= \sum_{j=0}^{\infty} (\xk^\top \xkd)^j \sum_{l=-{\infty}}^{\infty} \eta_{j,l}^{(i+1)} (\lvert\lvert \xk\rvert\rvert_2^2 \lvert\lvert \xkd\rvert\rvert_2^2)^{l/2}.
    \end{split}
\end{equation*} 
For the last line, we have used the fact that the series converges
absolutely. To see this, first of all note that
$\eta^{(i+1)}_{j,l}\geq 0$ because by assumption
$\eta_{j,l}^{(i)}\geq0$. Furthermore, given that $d>1$,
for any $\xk,\xkd$ we can find $\tilde{\xk},\tilde{x}'$ such that
$\lvert\lvert \xk \rvert\rvert_2^2 =\lvert\lvert \tilde{\xk}
\rvert\rvert_2^2$, $\lvert\lvert \xkd \rvert\rvert_2^2 =\lvert\lvert
\xkd\rvert\rvert_2^2$ and $\tilde{\xk}^\top \tilde{\xk}' = \lvert
\xk^\top \xkd \rvert$. Hence, we can conclude that $\sum_{j=0}^{\infty}
(\tilde{\xk}^\top \tilde{\xk}')^j \sum_{l=-{\infty}}^{\infty}
\eta_{j,l}^{(i+1)} (\lvert\lvert \tilde{\xk}\rvert\rvert_2^2
\lvert\lvert \tilde{\xk}'\rvert\rvert_2^2)^{l/2}$ is a sum of non
negative coefficients and hence the multi series converges
absolutely. Hence, we can conclude the induction.  \\ Next, note
that any of the properties 1-4 from the above discussion also
hold true for $t_{\dot{\sigma}}$. Therefore, we can use exactly the same
argument for $\dot{\Sigma}^{(i)}$ to show that for any $\xk, \xkd \neq
0$,
\begin{equation*}
    \dot{\Sigma}^{(i)}(\xk,\xkd) = 
    \sum_{j=0}^{\infty} (\xk^\top \xkd)^j \sum_{l=-{\infty}}^{\infty} \dot{\eta}_{j,l}^{(i)} (\lvert\lvert \xk\rvert\rvert_2^2 \lvert\lvert \xkd\rvert\rvert_2^2)^{l/2}.
\end{equation*}
with $\dot{\eta}_{j,l}^{(i+1)} \geq 0$. Finally, we can conclude the proof because 
\begin{equation*}
     k_{\textrm{NTK}}(\xk,\xkd) := \sum_{i=1}^{L+1} \Sigma^{(i-1)}(\xk,\xkd) \prod_{j=i}^{L+1} \dot{\Sigma}^{(j)}(\xk,\xkd)
\end{equation*}
when using the same argument as used above in the induction to show that the resulting multi sum converges absolutely. 
\end{proof}

We are now ready to prove Proposition \ref{prop:ntkass}.
First of all, we note that due to the above discussion, both $t_{\sigma}$ and $t_{\dot{\sigma}}$ are continuous functions. Hence, for any $\xk,\xkd \neq 0$, $\Sigma^{(i)}$ and $\dot{\Sigma}^{(i)}$ are compositions of continuous functions and thus also continuous. Hence, $k_{\textrm{NTK}}$ is also a continuous function. Next, note that the Lipschitz continuity (Assumption \Aktwo) follows straight forwardly from Equation \eqref{eq:ntklipschitz}. 

In order to show that any $g_j$ from Lemma \ref{lm:ntk1} is smooth, recall that 
\begin{equation*}
    g_j(x,y) = \sum_{l=-{\infty}}^{\infty} \eta_{j,l}^{(i+1)} (xy)^{l/2} =: h_j(x y).
\end{equation*}
Therefore, $h_j$ is a Puisaux power series with divisor $2$. Furthermore, the function $\tilde{h}_j(t) := h_j(t^2) = \sum_{l=-{\infty}}^{\infty} \eta_{j,l}^{(i+1)} (t)^{l}$ is a Laurent series which converges for every $t \neq 0$. Hence, we can conclude that $\tilde{h}_j$ is smooth for any $t \neq 0$ and thus also $h_j$. Finally, because $(x,y) \to xy$ is trivially also a smooth function, we can conclude that any $g_j$ is a smooth function for any $x,y \neq 0$. 
Next, since for any $l \in \mathbb{Z}$, $(x,y) \to \alpha (xy)^{l/2}$ is trivially a positive semi-definite (PSD) function whenever $\alpha \geq 0$ and sums of PSD functions are again PSD, we can conclude that the $g_j(x,y) = \sum_{l=-{\infty}}^{\infty} \eta_{j,l}^{(i+1)} (x y)^{l/2} $ is PSD for any $j$. Therefore, we can conclude that Assumption \Akone~ holds as well. 

The only thing left to show is Assumption \Akthree. While we have already shown that $g_j$ are smooth in a neighborhood of $(1,1)$, we still need to show that there exists $\jthresh> \floor{2/\beta}$ such that $g_{\jthresh}(1,1) >0$. However, this follows straight forwardly from the proof of Lemma \ref{lm:ntk1} and the fact that by assumption there exists $\jthresh> \floor{2/\beta}$ such that $a_{\jthresh} \neq$ where $a_j$ are the Hermite coefficients of the activation function. 
\qed
