# Supplementary material for: How rotational invariance of common kernels prevents generalization in high dimensions
Source: arXiv:2104.04244 source file (2021-04-09)
Supplement: Supplementary file 11 [file Appendix_Technical_Preliminaries_old.tex]

\section{Additional Results and Preliminaries}
\subsection{Concentration Inequalities}
\label{sec:technical_prel}
\begin{remark}
The proofs from this section closely follow the ideas presented in Appendix~A \cite{ElKaroui10}
\end{remark}

\begin{lemma}[Concentration of quadratic forms of bounded R.V.]
\label{lm:concentration}
Suppose the vector $\x \in \mathbb{R}^d$, of some dimension $d \in \mathbb{N}_+$, is a random vector with i.i.d distributed bounded entries $|\x[i]| \leq c_Z $ of zero mean and unit variance. Let $M$ be any symmetric matrix. Let $M = M_+ - M_{-}$ be the decomposition of $M$ into two positive semi-definite matrix $M_+$ and $M_-$ with $\|M_+\|_2, \|M_-\|_2 \leq 1$. Define
\begin{equation} 
\zeta = \frac{128 exp(4\pi) c_Z^2}{\trace(M_+)} \end{equation}
Then, for any $r/2 > \zeta$
\begin{equation}
    \begin{split}
        &P(|z^T M z/\trace(M_+) - \trace(M)/\trace(M_+)| > r)  \\\leq &8 \exp(4\pi) [\exp(-\trace(M_+)(r/2 - \zeta)^2/(32(1+\sqrt{\|M\|_2})^2  c_z^2) +  \exp(-\trace(M_+)/(32(1+\sqrt{\|M\|_2})^2 c_z^2))].
    \end{split}
\end{equation}
\end{lemma}
\begin{proof}
Note that we can decompose $M = M_+ - M_-$ in two positive semi definite matrix $M_+$ and $M_-$. Let 
\begin{equation}f: \mathbb{R}^d \to \mathbb{R}, \x -> \sqrt{\x^T M_+ \x / \trace(M_+)} =\frac{1}{\sqrt{\trace(M_+)}}\|M_+^{1/2} \x\|_2.
\end{equation}

We know that $f$ is a $\lambda_{\max}(M_+)/\sqrt{\trace(M)}$-Lipschitz continuous and hence also a $\sqrt{\|M\|_2}/\sqrt{\trace(M)}$-Lipschitz continuous. Using the simple fact that the norm is convex, we can apply Corollary~4.10 \cite{Ledoux2001}. The rest is obtained by straight forward following line by line the proof of Lemma~A.2 \cite{ElKaroui10}. We only highlight one intermediate step from the proof which will again be needed in this paper. For any $r>0$, one can show that
\begin{equation}
    \label{eq:concentration}
    P \left( \left|\sqrt{z^T M z/\trace(M_+)} - \sqrt{\trace(M)/\trace(M_+)} \right| > r \right) \leq 4 \exp(4 \pi) \exp(-\trace(M_+) r^2 /(16 c_z^2 \|M\|_2)).
\end{equation}
\end{proof}

\begin{lemma}[Concentration of quadratic forms of Gaussian R.V.]
\label{lm:concentrationgaussian}
Suppose the vector $\x \in \mathbb{R}^d$, of some dimension $d \in \mathbb{N}_+$, is a random vector with i.i.d normal distributed entries of zero mean and unit variance. Let $M$ be any symmetric matrix. Let $M = M_+ - M_{-}$ be the decomposition of $M$ into two positive semi-definite matrix $M_+$ and $M_-$ with $\|M_+\|_2, \|M_-\|_2 \leq 1$. Define
\begin{equation}
     \zeta = \frac{128 exp(4\pi)}{\trace(M_+)} 
\end{equation}
Then, for any $r/2 > \zeta$
\begin{equation}
    \begin{split}
        &P(|z^T M z/\trace(M_+) - \trace(M)/\trace(M_+)| > r)  \\\leq & \exp(-\trace(M_+)(r/2 - \zeta)^2/(32(1+\sqrt{\|M\|_2})^2 )) +  \exp(-\trace(M_+)/(32(1+\sqrt{\|M\|_2})^2 )).
    \end{split}
\end{equation}
\end{lemma}
\begin{proof}
The proof is essentially the same as the proof of Lemma \ref{lm:concentration}. However, note that because $\tilde{\x}_{(i)}$ are normally distributed, we can directly apply Theorem~\rom{5}.\rom{1} \cite{Milman86}. As a consequence, we can replace Equation \ref{eq:concentration} with
\begin{equation}
   P\left( \left|\sqrt{z^T M z/\trace(M_+)} - \sqrt{\trace(M)/\trace(M_+)} \right| > r \right) \leq  \exp(-\trace(M_+)r^2/(2 \|M\|_2).
\end{equation}
The proof follows then again from the proof of Lemma~A.2 \cite{ElKaroui10}.

\end{proof}
As a consequence, let
\begin{cor}
\label{cr:simplebound}
Let $\x_i,\x_j$ be distributed as given in Assumption A.1. Then, there exists generic constants $C_1,C_2,C_3 > 0$ such that for $\zeta = \frac{C_1}{\trace(\Sigma_n)}$, and any $r > \zeta$,
\begin{equation}
    P(|\x_i^T \x_j/\trace(\Sigma_n) - \delta_{i,j}| > r)  \leq C_3[\exp(-C_2\trace(\Sigma_n)(r/2 - \zeta)^2) +  \exp(-C_2\trace(\Sigma_n)].
\end{equation}
\end{cor}
\begin{proof}
The case where $i = j$ is straight forward when applying \ref{lm:concentration} respectively \ref{lm:concentrationgaussian}. For the other case, note that we can choose $M = \begin{pmatrix} 0 & \Sigma_n \\ \Sigma_n & 0 \end{pmatrix}$ and $M_+ = \frac{1}{2}\begin{pmatrix} \Sigma_n & \Sigma_n \\ \Sigma_n & \Sigma_n \end{pmatrix}$,  $M_- =  \frac{1}{2}\begin{pmatrix}0 & \Sigma_n \\ \Sigma_n & 0  \end{pmatrix}$ and $ v = (\tilde{\x}_i, \tilde{\x}_j)$ with $x_i$,$x_j$ distributed as given in Assumption A.1. The result then follows from $v^T M v = \x_i^T \x_j$ and $\trace(M) =0$, $\trace(M_+)= \trace(\Sigma_n)$. 
\end{proof}


\begin{proof}[Proof of Lemma \ref{lm:innerpr}]
We make us of the Borell-Cantelli Lemma and Corollary \ref{cr:simplebound}. For any $\epsilon > 0$, let $r(n) = n^{-\beta/2} \ (\log(n))^{1+\epsilon} $ and note that because $ \trace(\Sigma_n) \asymp n^{\beta}$, for any $n$ sufficiently large $r(n)/2 > \zeta \to 0$. In particular, we have that $\zeta$ decays at rate $n^{-\beta}$. Hence, making use of Corollary \ref{cr:simplebound}, we can see that there exists some generic constant $C>0$ such that for any $n$ sufficiently large
\begin{equation*}
    \begin{split}
        &P(|\x_i^T \x_j/\trace(\Sigma_n) - \delta_{i,j}| > r(n))  \\  \leq &C_3 [\exp(-C_2\trace(\Sigma_n)(r/2 - \zeta)^2) +  \exp(-C_3\trace(\Sigma_n))] \\ &\leq \exp(-C \ (\log(n))^{1+\epsilon}).
    \end{split}
\end{equation*}
Using the union bound, we get
\begin{equation*}
    \begin{split}
        P(\underset{i,j}{\max} |\x_i^T \x_j/\trace(\Sigma_n) - \delta_{i,j}| > r(n)) \leq n^2 \exp(-C \ (\log(n))^{1+\epsilon} /(288c_z^2).
    \end{split}
\end{equation*}
And because $\epsilon>0$, for any $N \in \mathbb{N}_+$, we have that \begin{equation}
\sum_{n=N}^{\infty}  n^2 \exp(-C \ (\log(n))^{1+\epsilon}) < \infty.
\end{equation}
which allows us to apply the Borel Cantelli Lemma, and hence,
\begin{equation}
\underset{i,j}{\max} \left|\x_i^T \x_j /\trace(\Sigma_d) - \delta_{i,j}\right| \leq
n^{-\beta/2}  (\log(n))^{1+\epsilon} ~ ~~ a.s.
\end{equation}
which concludes the proof for the random variable $\x_i^T \x_j$. \\
For $\lvert\lvert \x_i - \x_j \rvert \rvert_2^2/\trace(\Sigma_d) $, we can write
\begin{equation}
    \lvert\lvert \x_i - \x_j \rvert \rvert_2^2/\trace(\Sigma_d) =  \x_i^T x_i/\trace(\Sigma_d) + \x_j^T x_j/\trace(\Sigma_d) -2 \x_i^T x_j/\trace(\Sigma_d).
\end{equation}
Hence, the proof follows when taking the triangular inequality.
\end{proof}

\begin{cor}\mw{Haven't seen proof of the main theorem, but maybe this cor is not necessary}
\label{cr:testsample}
Let $\Xrv$ be independently drawn form the same distribution as the input vectors $\X$. Then, for any $\epsilon > 0$ and $n$ sufficiently large, there exists some constant $C>0$ such that, with probability $\leq n^2 \exp(-C  (\log(n))^{1+\epsilon})$ over the draws of $\X$, 
\label{lm:norm}
\begin{equation}
\underset{i}{\max}\left| \x_i^TX\right|/\tr(\Sigma_d) \leq n^{-\beta/2} (\log(n))^{1+\epsilon} \quad a.s.
\end{equation}
and 
\begin{equation}
\left| (\Xrv)^\top \Xrv /\tr(\Sigma_d) -1 \right| \leq  n^{-\beta/2} (\log(n))^{1+\epsilon} \quad a.s.
\end{equation}
\end{cor}
\begin{proof}
Denote with $\mathcal{E}_{\textbf{X}}$ the set of input samples $\mathbb{X}$ which satisfy the concentration inequality from Lemma \ref{lm:innerpr} and with $\mathcal{E}_{\textbf{X},X} \subset \mathcal{E}_{\textbf{X},X} $ the event where also the concentration inequalities from Corollary \ref{cr:testsample} hold true for an independent random variable $X$ drawn from the same distribution. 
 We already know from the proof of Lemma \ref{lm:innerpr} that for any $n$ sufficiently large, $P(\mathcal{E}_{\textbf{X}}) \geq 1-  n^2 \exp(-C \ (\log(n))^{1+\epsilon})$. Furthermore, we can use again the same argument as used in the proof of Lemma \ref{lm:innerpr} to show that
 $P(\mathcal{E}_{\textbf{X},X} \geq 1 -  (n+1)^2 \exp(-C \ (\log(n))^{1+\epsilon})$. The proof then follows form the simple fact that 
 \begin{equation}
 \begin{split}
      P(\mathcal{E}_{\textbf{X}, \Xrv} | \textbf{X} \in \mathcal{E}_{\textbf{X}}) P(\mathcal{E}_{\textbf{X}}) = P(\mathcal{E}_{\textbf{X}, \Xrv})  &\geq 1 -  (n+1)^2 \exp(-C \ (\log(n))^{1+\epsilon}) \\
      P(\mathcal{E}_{\textbf{X}, \Xrv} | \textbf{X} \in \mathcal{E}_{\textbf{X}}) &\geq  \frac{1}{ P(\mathcal{E}_{\textbf{X}}) } \left[1 -  (n+1)^2 \exp(-C \ (\log(n))^{1+\epsilon}) \right]\\
        P(\mathcal{E}_{\textbf{X}, \Xrv} | \textbf{X} \in \mathcal{E}_{\textbf{X}}) &\geq  1 -  (n+1)^2 \exp(-C \ (\log(n))^{1+\epsilon})
      \end{split}
 \end{equation}
Where we have used that $\mathcal{E}_{\textbf{X}, \Xrv} \subset \mathcal{E}_{\textbf{X}}$. 
 
\end{proof}



\begin{cor}
\label{cr:exponentialbound}
Let $\Xrv$ be independently drawn from the same distributions as the samples $\X$. Then there exists a generic constant $C>0$ such that:
\begin{equation}
    P\left( \left| \sqrt{\Xrv^T \Xrv}/\trace(\Sigma_d) -1  \right| > r \right) \leq \exp(-C n^{\beta} r^2).
    \end{equation}
    \end{cor}
\begin{proof}
For the spherical input data this follows immediat. For the other case, the proof follows straight forwardly from the proof of Lemma \ref{lm:concentration}. 
\end{proof}



\begin{cor}
\label{cr:concentrationh}
For any $\epsilon>0$ and any $k>0$, we have
\begin{equation}
 \underset{i}{\max}~ \left| \frac{(\x_i^T \x_i)^k}{ (\trace(\Sigma_d))^k} - 1 \right| \leq  c_k\max[n^{-\beta/2} (\log(n))^{1+\epsilon}, n^{-k\beta/2}log(n)^{k(1+\epsilon)}] \quad a.s.
 \end{equation}
where $c_k$ is a constant only depending on $k$.
\end{cor}

\begin{proof}
By Lemma \ref{lm:concentration}, we have for every $k>0$
\begin{equation}
 \underset{i}{\max}~ \left| \left[\frac{(\x_i^T \x_i)}{\trace(\Sigma_d)} - 1\right]^k \right| \leq ( n^{-\beta/2} (\log(n))^{1+\epsilon})^k.
 \end{equation}
We proof the the claim by induction. The case where $k=1$ holds trivially with $c_k = 1$. For $k>1$, we have
\begin{equation*}
    \underset{i}{\max}~  \left| \left[\frac{(\x_i^T \x_i)}{\trace(\Sigma_d)} - 1\right]^k \right| =  \underset{i}{\max}~  \left| \frac{(\x_i^T \x_i)^k}{ (\trace(\Sigma_d))^k} + \sum_{j=1}^k (-1)^j {k \choose j }  \left(\frac{\x_i^T \x_i}{\trace(\Sigma_d)}\right)^{k-j}\right| \leq  (n^{-\beta/2} (\log(n))^{1+\epsilon})^k.
\end{equation*} 
Note that we know by induction that $ \underset{i}{\max}~ \left| \frac{(\x_i^T \x_i)^k}{ (\trace(\Sigma_d))^k} - 1 \right| \leq  c_k n^{-\beta/2}log(n)^{k(1+\epsilon)}$. Furthermore, we have $\sum_{j=1}^k(-1)^j {k\choose j} = -1$ which shows that
\begin{equation}
\begin{split}
 &\underset{i}{\max}~ \left| \frac{(\x_i^T \x_i)^k}{ (\trace(\Sigma_d))^k} + \sum_{j=1}^k (-1)^j {k \choose j } \left( \frac{(\x_i^T \x_i)^k}{ (\trace(\Sigma_d))^k}\right)^{k-j} \right| \\ =  &\underset{i}{\max}~ \left| \frac{(\x_i^T \x_i)^k}{ (\trace(\Sigma_d))^k} + \sum_{j=1}^k (-1)^j {k \choose j } \right[ \left( \frac{(\x_i^T \x_i)^k}{ (\trace(\Sigma_d))^k}\right)^{k-j} -1 \left]+ \sum_{j=1}^k (-1)^j {k \choose j }  \right|\\
 \leq &\underset{i}{\max}~ \left| \frac{(\x_i^T \x_i)^k}{ (\trace(\Sigma_d))^k} -1 \right| + \sum_{j=1}^k {k \choose j }  c_j\max\left[n^{-\beta/2} (\log(n))^{1+\epsilon}, n^{-j\beta/2}log(n)^{j(1+\epsilon)}\right].
 \end{split}
 \end{equation}
 Hence, combining these two results, we have that 
 \begin{equation}
      \underset{i}{\max}~ \left| \frac{(\x_i^T \x_i)^k}{ (\trace(\Sigma_d))^k} -1\right| \leq (n^{-\beta/2} (\log(n))^{1+\epsilon})^k + \sum_{j=1}^k {k \choose j }  c_j\max \left[n^{-\beta/2} (\log(n))^{1+\epsilon}, n^{-j\beta/2}log(n)^{j(1+\epsilon)} \right]
 \end{equation}
which completes the induction and thus the proof. 
\end{proof}


\begin{cor}\mw{Never used.}
\label{lm:innerpSphere}
For any $\epsilon > 0$, we have that asymptotically
\label{lm:norm}
\begin{equation}
\max_{i,j }\left| \left(\frac{\x_i}{\|\x_i\|_2}  \right)^T \frac{\x_j}{\|\x_j\|_2} - \delta_{i, j}\right| \leq 4 n^{-\beta/2} (\log(n))^{1+\epsilon} ~~~ a.s.
\end{equation}
\end{cor}

\begin{proof}
The case where $i = j$ holds trivially true. Let $s_i = \frac{\x_i}{\|\x_i\|_2}$ and $\z_i = \frac{\x_i}{\sqrt{\trace(\Sigma_n)}}$. Since we are in the Euclidean space, the inner product is given by
\begin{equation} 
(s_i^Ts_i)^2 = (\cos(\alpha))^2 
\end{equation}
and 
\begin{equation} 
(\z_i^T\z_j)^2 = (\cos(\alpha))^2 \|\z_i\|_2^2 \|\z_j\|_2^2 
\end{equation}
with $\alpha \in [0, 2\pi]$. Let $l(n) := n^{-\beta/2}  (\log(n))^{1+\epsilon}$, then by Lemma \ref{lm:innerpr} we have that $|~ \|\z_i\|_2^2 -1 | \leq l(n)  ~ a.s.$.Therefore,
\begin{equation}
    \begin{split}
        |(s_i^Ts_i)^2 - (\z_i^T\z_j)^2| &= (\cos(\alpha))^2 |1 - \|\z_i\|_2^2 \|\z_j\|_2^2|\\
        &\leq  |1 - \|\z_i\|_2^2| + \|\z_i\|_2^2 |1 - \|\z_j\|_2^2|\\
        &\leq 2l(n) + (l(n))^2
    \end{split}
\end{equation}
which concludes the proof.
\end{proof}




\subsection{Lemmas}
\label{sec:AC_lemmas}

% We now present some additional lemmas used for the proof of Theorem \ref{thm:main_thm}.

\begin{proof}[Proof of Lemma \ref{lm:AC_assumptions}]
 The only point which does not follow immediately is to show that $\reminder$ is a continuous function. For this, write $g$ as a function of the variables $x,y,z$, i.e.
 \begin{equation}
  \rotkerfunc(x,y,z) =  \sum_{j=0}^{\infty} \rotkerfunccoeffj{j}(x,y) z^j.
   \end{equation}
For every $x,y$, define the function $\rotkerfunc_{x,y}(z) = g(x,y,z)$. Due to the series expansion, we can make use the theory on the Taylor expansion theory implying that for any $x,y$, $\rotkerfunc_{x,y}$ is a smooth function in the interior of $\convergeset{\delta}$ (using the definition form Assumption \Akone). Hence, we can conclude that there exists a function $\reminder$ such that 
\begin{equation}
 \rotkerfunc_{x,y}(z) =   \sum_{j=0}^{m} \rotkerfunccoeffj{j}(x,y) z^j + (z)^{m+1} \reminder_{x,y}(z)
\end{equation}
In particular, the smoothness of $\rotkerfunc_{x,y}(z)$ implies that $\reminder_{x,y}$ is continuous in the interior of $\{z : (x,y,z) \in \convergeset{\delta} \}$. Next, define
$\reminder(x,y,z) = \reminder_{x,y}(z)$ and note that that the continuity of $\rotkerfunc$ implies that $\reminder$ is continuous everywhere except for the plane $z=0$. Finally, because $ \reminder_{x,y}(0)$ exists point wise, we conclude that $\reminder$ exists and is a continuous function in the interior of $\convergeset{\delta}$. Hence the proof follows. 
\end{proof}




\begin{proof}[Proof of Lemma \ref{lm:AC_rbf}]
By assumption $h$ is locally analytic, we know that $h$ has a local Taylor series around $2$, i.e.
\begin{equation}
\label{eq:lemmaRBFass1}
    h(\| \xk - \xkd \|_2^2) = \sum_{j=0}^{\infty} h_j ~ (\| \xk - \xkd \|_2^2-2)^j,
\end{equation}
which converges for any $\left|\| \xk - \xkd \|_2^2-2 \right| \leq \tilde{\delta}$ where $\tilde{\delta}>0$ is the convergence radius of the Taylor series approximation. In particular, we know that the series converges absolutely for any $\xk,\xkd$ with 
$\left|\| \xk - \xkd \|_2^2-2 \right| < \tilde{\delta}$. The Next, using $\| \xk - \xkd \|_2^2 -2 = \| \xk \|_2^2 -1 + \|  \xkd \|_2^2 -1 -2 \xk^\top\xkd$, we can make use of the Binomial series, which shows us that
\begin{equation}
\label{eq:lemmaRBFass1}
    h(\| \xk - \xkd \|_2^2) = \sum_{j=0}^{\infty}  h_j \sum_{i=0}^j  \sum_{l=0}^i {j \choose i} {i \choose l} (\| \xk \|_2^2 -1)^l  (\|  \xkd \|_2^2 -1)^{i-l} (-2 \xk^\top\xkd)^{j-i}
\end{equation}
The goal is now to show that this multi series converges absolutely. For this, whenever $d>1$, we can choose $\tilde{\xk},\tilde{\xkd} \in \mathbb{R}^{d}$ such that $ \| \tilde{\xk}  \|_2^2 -1>0$ , $\| \tilde{\xkd}  \|_2^2 -1 >0$ and $ \tilde{\xk}^\top\tilde{\xkd} <0$. As a result, we can see that for any $j$, the sum
\begin{equation}
\sum_{i=0}^j  \sum_{l=0}^i {j \choose i} {i \choose l} (\|  \tilde{\xk} \|_2^2 -1)^l  (\|  \tilde{\xkd} \|_2^2 -1)^{i-l} (-2 \tilde{\xk}^\top\tilde{\xkd})^{j-i}
\end{equation}
is a sum of non zero summands. Hence, we get that the sum
\begin{equation}\label{eq:commentF1}
\sum_{j=0}^{\infty}  h_j \sum_{i=0}^j  \sum_{l=0}^i {j \choose i} {i \choose l} (\|  \tilde{\xk} \|_2^2 -1)^l  (\|  \tilde{\xkd} \|_2^2 -1)^{i-l} (-2 \tilde{\xk}^\top\tilde{\xkd})^{j-i}
\end{equation} 
converges absolutely. Hence, we can arbitrarily reorder the summands in the sum:
\begin{equation}
\label{eq:lemmaRBFass2}
\begin{split}
    h(\|  \tilde{\xk} - \tilde{\xkd} \|_2^2) &=  \sum_{j=0}^{\infty} (\tilde{\xk}^\top\tilde{\xkd})^{j}  \sum_{i=j}^{\infty}   \sum_{l=0}^{i-j}  h_{i} (-2)^j {i \choose j} {i-j \choose l} (\|  \tilde{\xk} \|_2^2 -1)^l  (\|  \tilde{\xkd} \|_2^2 -1)^{i-l-j} \\
    &=:\sum_{j=0}^{\infty}(\tilde{\xk}^\top\tilde{\xkd})^{j} g_j(\|  \tilde{\xk} \|_2^2, \|  \tilde{\xkd} \|_2^2)
    \end{split}
\end{equation} 
In particular, we obtain that the sum from Equation \ref{eq:lemmaRBFass2} converges absolutely for any $\xk,\xkd$ with $ \| \tilde{\xk}  \|_2^2 -1> \left|\| \xk  \|_2^2 -1\right|$ , $\| \tilde{\xkd}  \|_2^2 -1 > \left|\| \xkd  \|_2^2 -1 \right|$ and $ -\tilde{\xk}^\top\tilde{\xkd} > \left|\xk^\top\xkd\right|$. In fact, we can always find $\delta,\delta' >0$ such that any  $(\xk,\xkd) \in \mathbb{R}^d \times \mathbb{R}^d$, with $(\| \xk\|_2^2, \| \xkd\|_2^2) \in  [1-\delta, 1+\delta] \times [1-\delta, 1+\delta]$ and $\xk^\top \xkd \in  [-\delta',\delta']$ satisfies these constraints and hence the sum from Equation \ref{eq:lemmaRBFass2} converges absolutely. We can then conclude the proof when noting that the functions $g_i$ are implicitly defined using the Taylor series expansion. Therefore, we can conclude that $g_i$ are smooth functions. Finally, we obtain the reminder term $\reminder$ when from the same argument as used in Lemma \ref{lm:AC_assumptions} and hence we can show that the \makepurple{assumption \Ckone}  holds true. 
\end{proof}

% 
% \begin{proof}[Corollary \ref{cr:polyexpr}]
% 
% \kd{This is quite obvious, add a few sentences here}
% 
% 
% \end{proof}
% 


%\begin{cor}
%\label{cr:exponentialbound}
%For any $\x \in \mathbb{R}^{d(n)}$  generated from the same distribution as $\x_i$ \makepurple{from Assumption A.1}, we have %that
%$$
%P\left( \left| \sqrt{\x_i^T \x_j} \right| > r \right) \leq \exp(-\trace(\Sigma) (r-1)^2 /(32 c_z^2))$$ 
%\end{cor}
%\begin{proof}
%The proof follows straight forward from the proof of Lemma \ref{lm:concentration}. 
%\end{proof}

% %%%
% \begin{cor}
% \label{lm:consistent}
% Let $\hat{t}_n := \frac{1}{n} \sum_{i=1}^n \x_i^T \x_i $. For any $\epsilon >0$ and  $n$ sufficiently large, we have that for any $i \in \{1,...,n\}$,
% $$\left| \frac{\x_i^T \x_i}{\hat{t}} - \frac{\x_i^T \x_i}{\trace(\Sigma_n)} \right| \leq  3  n^{-\beta/2} (\log(n))^{1+\epsilon} ~~a.s.$$
% \end{cor}
% \begin{proof}
% Due to Lemma \ref{lm:innerpr}, we get for any $\epsilon > 0$
% $$ \left|\frac{\hat{t}}{\trace(\Sigma_n)} - 1 \right| = \left|\frac{1}{n} \sum_{i =1}^n \frac{\x_i^T\x_i}{\trace(\Sigma_n)} - 1 \right| \leq  n^{-\beta/2} (\log(n))^{1+\epsilon} ~~~ a.s
% $$
% and thus, 
% \begin{equation}
% \begin{split}
%     \left|\frac{\x_i^T \x_i}{\hat{t}} - \frac{\x_i^T \x_i}{\trace(\Sigma_n)}) \right| &=  \left|\frac{\x_i^T \x_i (\trace(\Sigma_n)- \hat{t})}{\hat{t} \trace(\Sigma_n)} \right| = 
%     \left|\frac{\frac{\x_i^T \z_i}{\trace(\Sigma_n)} (\frac{\hat{t}}{\trace(\Sigma_n)}-1)}{\frac{\hat{t}}{\trace(\Sigma_n)}} \right| \\
%     &\leq \frac{(1+  n^{-\beta/2} (\log(n))^{1+\epsilon})  n^{-\beta/2} (\log(n))^{1+\epsilon}}{1-  n^{-\beta/2} (\log(n))^{1+\epsilon}} ~~~ a.s.\\
%     &\leq 3  n^{-\beta/2} (\log(n))^{1+\epsilon} ~~~ a.s.
% \end{split}
% \end{equation}
% where we choose $n$  sufficiently large such that $ n^{-\beta/2} (\log(n))^{1+\epsilon} \leq 0.5$
% \end{proof}
% %%%
