# Supplementary material for: How rotational invariance of common kernels prevents generalization in high dimensions
Source: arXiv:2104.04244 source file (2021-04-09)
Supplement: Supplementary file 12 [file Appendix_NTK.tex]

\section{Neural Tangent Kernels}
We use the definition of the Neural Tangent Kernel presented in \cite{Arora19,Lee18}. Let $L$ be the depth of the NTK and $\sigma: \mathbb{R} \to \mathbb{R}$ any differentiable $k$-homogeneos activation function, i.e. where for all $x \in  \mathbb{R}$, $\sigma(a x) = a^k$.
activation function. For any $i>0$, define the recursion
\begin{equation}
  \begin{split}\Sigma^{(0)}(X,X') &:= X^T X' \\
\Lambda^{(i)}(X,X') &:= \begin{pmatrix} \Sigma^{(i-1)}(X,X) & \Sigma^{(i-1)}(X,X') \\ \Sigma^{(i-1)}(X,X') & \Sigma^{(i-1)}(X',X')\end{pmatrix} \\
\Sigma^{(i)}(X,X') &:= c_{\sigma} \underset{(u,v) \sim \mathcal{N}(0, \Lambda^{(i)})}{\mathbb{E}}~\left[ \sigma(u) \sigma(v) \right] 
\end{split}
\end{equation}
with 
$$ c_{\sigma} := \left[ \underset{v \sim \mathcal{N}(0, 1}{\mathbb{E}}~\left[ \sigma(v)^2 \right] \right]^{-1}$$
Furthermore, define
$$ \dot{\Sigma}^{(i)} := c_{\sigma} \underset{(u,v) \sim \mathcal{N}(0, \Lambda^{(i-1)})}{\mathbb{E}} ~\left[ \dot{\sigma}(u) \dot{\sigma(v)} \right]  $$
with $\dot{\sigma}$ being the derivative of $\sigma$.
The NTK kernel$ h_{\textrm{NTK}}$ is then defined to be
$$ h_{\textrm{NTK}}(X,X') = \sum_{i=1}^{L+1} \Sigma^{(i-1)}(X,X') \prod_{j=i}^{L+1} \dot{\Sigma}^{(j)}(X,X')$$
As in \cite{Arora19}, we can set $\dot{\Sigma}^{(L+1)}(X,X') = 1$. There exists many theoretical results showing that deep Neural Networks trained with Gradient Descent at initialisation enter the NTK regime when increasing the width to infinte. For a recent result, we refer to \cite[Theorem~3.1]{Arora19}, which only holds true for the case where $||X||_2 \leq 1$ and $||X'||_2 \leq 1$. This is clearly not the case for the data set $\textbf{X}$, which is centred around $1$. However, we can see that for $n$ sufficiently large and for any $\tau >1 $, we have that $ |\frac{X_i}{\tau} | \leq 1 ~ a.s.$. Hence, we let
$$ k_{\textrm{NTK},\tau}(X,X') = h_{\textrm{NTK}}(\frac{X}{\tau}, \frac{X'}{\tau})$$
For $n$ sufficiently large, $k_{\textrm{NTK},\tau}$almost surely satisfies the assumptions in \cite[Theorem~3.1]{Arora19} if $\tau >1$ for $\textbf{X}$ as input data and $\tau \geq 1$ for $\textbf{S}$ as input data. We can now show the following important Corollary:
\begin{cor}
\label{cr:ntk2}
Assume that $\sigma(x) = \max(0,x)$ is the Relu activation function and let $\tau >1$. Then, $k_{\textrm{NTK},\tau}$ satisfies the assumptions from Theorem \ref{th:elkarouiextension}
\end{cor}
In order to proof this corollary, we begin with the following Lemma. 
\begin{lemma} 
\label{lm:ntk1}
Assume that $\sigma$ is chosen such that the map $\hat{t}(\rho) : [-1,1] \to \mathbb{R}$,
$$\hat{t}_{\sigma}(\rho) = \underset{(u,v) \sim \mathcal{N}(0, \tilde{\Lambda}(\rho))}{\mathbb{E}}~\left[ \sigma(u) \sigma(v) \right] $$
with $\tilde{\Lambda}(\rho) = \begin{pmatrix} 1& \rho \\ \rho & 1 \end{pmatrix} $ has image $\{ \hat{t}(x) | x\in [-1,1] \} \subset [-\frac{1}{c_{\sigma}},\frac{1}{c_{\sigma}}]$. Furthermore, define $\dot{t}(\rho) : [-1,1] \to \mathbb{R}$, 
$$\hat{t}_{\dot{\sigma}}(\rho) = \underset{(u,v) \sim \mathcal{N}(0, \tilde{\Lambda}(\rho))}{\mathbb{E}}~\left[ \dot{\sigma}(u) \dot{\sigma}(v) \right] $$
Assume that $\hat{t}_{\sigma}$ and $\hat{t}_{\dot{\sigma}}$ may be expressed in form of a power series around $0$ which converges absolutely for every $\rho \in [-1,1]$ to $\hat{t}_{\sigma}$ respectively $\hat{t}_{\dot{\sigma}}$. Let $\tau >1$, and let $\delta  =  \min(1/4, \tau -1)$. Then, for any $X,X' \in \mathbb{R}^d$ with $|~||X||_2^2 -1 | \leq \delta$, $|~||X'||_2^2 -1 | \leq \delta$, the kernel $k_{\textrm{NTK},\tau}$ from Equation \ref{eq:ntkdef} satisfies Assumption \ref{ass:kernel} with 
\begin{equation}
    \label{eq:gi}
    g_m(x,y) = \sum_{l = I_m}\frac{1}{\tau^m}  \eta_{m}^l (\frac{1}{\sqrt{\tau}} x)^{\alpha_{m}^{l}} (\frac{1}{\sqrt{\tau}}  y)^{\alpha_{m}^{l}}
\end{equation}
where $I_m$ is a possibly infinite index set and $\eta_{m}^l, \alpha_{m}^{l} \in \mathbb{R} $ are such that the series converges absolutely for any $(x,y) \in [\frac{1-\delta}{\tau},\frac{1+\delta}{\tau}]^2$
\end{lemma}


\begin{proof}
 Let $\tilde{X} = \frac{1}{\tau} X$ and $\tilde{X}' = \frac{1}{\tau} X'$.
The proof is separated into several steps:\\\\
\textbf{Step 1:} In a first step, a closed form expression for $\Sigma^{(i)}(\tilde{X},\tilde{X})$ is derived. As already shown in \cite[Section~E.1]{Arora19}, for any $i>0$
\begin{equation}
    \label{eq:rec1}
     \Sigma^{(i)}(\tilde{X},\tilde{X}') = c_{\sigma} \left(\Sigma^{(i-1)}(\tilde{X},\tilde{X}) \Sigma^{(i-1)}(\tilde{X}',\tilde{X}')  \right)^{k/2} \hat{t}\left( \frac{\Sigma^{(i-1)}(\tilde{X},\tilde{X}')}{\sqrt{\Sigma^{(i-1)}(\tilde{X},\tilde{X}) \Sigma^{(i-1)}(\tilde{X}',\tilde{X}')}} \right)
\end{equation}
where the fact is used that $\sigma$ is $k$-homogeneous.
Plugging in the definition of $\hat{t}$ and $c_{\sigma}$ shows that
$$ \Sigma^{(i)}(\tilde{X},\tilde{X}) = \left(\Sigma^{(i-1)}(\tilde{X},\tilde{X})\right)^k $$ 
and by induction, we get that
$$\Sigma^{(i)}(\tilde{X},\tilde{X}) = (\tilde{X}^T\tilde{X})^{k^i}$$
Thus, Equation \ref{eq:rec1} becomes 
\begin{equation}
\label{eq:ntkproof2}
    \Sigma^{(i)}(\tilde{X},\tilde{X}') = c_{\sigma} (\tilde{X}^T\tilde{X})^{\frac{k^i}{2}}(\tilde{X}'^T\tilde{X}')^{\frac{k^i}{2}} \hat{t}_{\sigma}\left( \frac{\Sigma^{(i-1)}(\tilde{X},\tilde{X}')}{(\tilde{X}^T\tilde{X})^{\frac{k^{i-1}}{2}}(\tilde{X}'^T\tilde{X}')^{\frac{k^{i-1}}{2}}} \right) 
\end{equation} 
 At this point, note that the recursion from Equation \ref{eq:rec1} is well defined for arbitrary $\tilde{X},\tilde{X}'$. Indeed, we have that $$\frac{\Sigma^{(i-1)}(\tilde{X},\tilde{X}')}{(\tilde{X}^T\tilde{X})^{\frac{k^{i-1}}{2}}(\tilde{X}'^T\tilde{X}')^{\frac{k^{i-1}}{2}}} \leq 1$$ which follows by induction when using the assumption that the image of $\hat{t}_{\sigma}$ is contained in the subset $\{\hat{t}_{\sigma}(\rho|\rho\in[-1,1]\} \subset [-\frac{1}{c_{\sigma}},\frac{1}{c_{\sigma}}]$
 
\textbf{Step 2:} The next step is to derive an expression for the case where $\tilde{X}, \tilde{X}'$ are not necessarily the same. 
The goal is to show that $\Sigma^{(i)}(\tilde{X},\tilde{X}')$ can be written in the form of an absolute converging sum of the form of 
\begin{equation}
\label{eq:ntkgi}
    \begin{split}
        \Sigma^{(i)}(\tilde{X},\tilde{X}') 
        &= \sum_{j=0}^{\infty} (\tilde{X}^T\tilde{X}')^j \sum_{l \in I_{j,i}} \eta_{j,i}^l ((||\tilde{X}||_2^2)^{\alpha_{j,i}^{l}} (||\tilde{X}'||_2^2)^{\alpha_{j,i}^{l}}) \\
    \end{split}
\end{equation} 
 In particular, we show that the index set $I_i$ and $\alpha_{i}^{l}, \eta_{i}^l \in \mathbb{R}$ are such that the sum
\begin{equation}
    \label{eq:gi}
    \sum_{l = I_{j,i}} \eta_{j,i}^l x^{\alpha_{j,i}^{l}} y^{\alpha_{j,i}^{l}}
\end{equation}
converges absolutely for any $x,y \in (0,1]$. The proof is by induction. In a first step, note that the case where $i=0$ holds trivially true. Next, assume that $\Sigma^{(i)}(X,X')$ can be written as an absolute converging series of the form of Equation \ref{eq:ntkgi}
satisfying the assumptions above. We can now use the fact that $\hat{t}$ has an absolute converging Taylor series expansion around $0$, i.e.
$$\hat{t}_{\sigma}(x) = \sum_{i=0}^{\infty} t_i x^i$$
with $t_i$ being the Taylor series coefficients. In combination with Equation \ref{eq:ntkproof2}, we can see that 
\begin{equation*}
    \begin{split}
        \Sigma^{(i+1)}(\tilde{X},\tilde{X}') &= c_{\sigma} (\tilde{X}^T\tilde{X})^{\frac{k^{i}}{2}}(\tilde{X}'^T\tilde{X}')^{\frac{k^{i}}{2}} \sum_{m=0}^{\infty} t_m \left(\frac{\Sigma^{(i)}(\tilde{X},\tilde{X}')}{(\tilde{X}^T\tilde{X})^{\frac{k^{i-1}}{2}}(\tilde{X}'^T\tilde{X}')^{\frac{k^{i-1}}{2}}} \right)^m \\
        &= c_{\sigma} (\tilde{X}^T\tilde{X})^{\frac{k^{i}}{2}}(\tilde{X}'^T\tilde{X}')^{\frac{k^{i}}{2}} \sum_{m=0}^{\infty} t_m \left(\frac{\sum_{j=0}^{\infty} (\tilde{X}^T\tilde{X}')^j g_j (||\tilde{X}||_2^2, ||\tilde{X}'||_2^2)}{(\tilde{X}^T\tilde{X})^{\frac{k^{i-1}}{2}}(\tilde{X}'^T\tilde{X}')^{\frac{k^{i-1}}{2}}} \right)^m \\
        &= c_{\sigma} (||\tilde{X}||_2^2)^{\frac{k^{i}}{2}}(||\tilde{X}'||_2^2)^{\frac{k^{i}}{2}} \sum_{m=0}^{\infty} t_m \left(\frac{\sum_{j=0}^{\infty} (\tilde{X}^T\tilde{X}')^j \sum_{l \in I_{j,i}} \eta_{j,i}^l (||\tilde{X}||_2^2)^{\alpha_{j,i}^{l}} (||\tilde{X}'||_2^2)^{\alpha_{j,i}^{l}}}{(||\tilde{X}||_2^2)^{\frac{k^{i-1}}{2}}(||\tilde{X}'||_2^2)^{\frac{k^{i-1}}{2}}} \right)^m \\
        &= c_{\sigma}  \sum_{m=0}^{\infty} t_m \left(
        \sum_{j=0}^{\infty} (\tilde{X}^T\tilde{X}')^j \sum_{l \in I_{j,i}} \eta_{j,i}^l (||\tilde{X}||_2^2)^{\left(\alpha_{j,i}^{l} - \frac{k^{i-1}}{2} + \frac{k^i}{2m}\right)} (||\tilde{X}'||_2^2)^{\left(\alpha_{j,i}^{l} - \frac{k^{i-1}}{2} +\frac{k^i}{2m} \right)}
         \right)^m
    \end{split}
\end{equation*} 
where in the last line  we have used  that $\tilde{X}^T\tilde{X} = ||\tilde{X}||_2^2$. Finally, we can complete the induction by using that each of the sums converge absolutely. 
\\
\textbf{Step 3:} We can repeat exactly the same argument for $\dot{\Sigma}^{(i)}$. It is well known that if $\sigma$ is a $k$-homogeneous function, the derivative $ \dot{\sigma}$ is a $k-1$-homogeneous function. Hence, we have that 
$$\dot{\Sigma}^{(i)} =c_{\sigma} (\tilde{X}^T\tilde{X})^{\frac{k^{i-1}(k-1)}{2}}(\tilde{X}'^T\tilde{X}')^{\frac{k^{i-1}(k-1)}{2}} \hat{t}_{\dot{\sigma}}\left( \frac{\Sigma^{(i-1)}(\tilde{X},\tilde{X}')}{(\tilde{X}^T\tilde{X})^{\frac{k^{i-1}}{2}}(\tilde{X}'^T\tilde{X}')^{\frac{k^{i-1}}{2}}} \right)  $$
and using the same argument as before, we can see that $\dot{\Sigma}^{(i)}$ can also be expressed as an absolute converging sum of the form of Equation \ref{eq:ntkgi}.\\
Recall that by definition
$$ k_{\textrm{NTK},\tau}(X,X') = h_{\textrm{NTK}}(\tilde{X},\tilde{X}') = \sum_{i=1}^{L+1} \Sigma^{(i-1)}(\tilde{X},\tilde{X}') \prod_{j=i}^{L+1} \dot{\Sigma}^{(j)}(\tilde{X},\tilde{X}') $$
We are now using the fact that for every $i>0$, every sum in the expressions of $\Sigma^{(i-1)}(\tilde{X},\tilde{X}')$ and $\dot{\Sigma}^{(i)}(\tilde{X},\tilde{X}')$ is an absolute converging sums of the form of Equation \ref{eq:ntkgi}. Hence $h_{\textrm{NTK}}(\tilde{X},\tilde{X}')$ is also an absolute converging sum of the form of 
\begin{equation}
    \label{eq:posdefntk}
      h_{\textrm{NTK}}(\tilde{X},\tilde{X}') = \sum_{j=0}^{\infty} (\tilde{X}^T\tilde{X}')^j \sum_{l \in I_{j}} \eta_{j}^l (||\tilde{X}||_2^2)^{\alpha_{j}^{l}} (||\tilde{X}'||_2^2)^{\alpha_{j}^{l}})
\end{equation}
Furthermore, we can see that 2) from Assumption \ref{ass:1} holds true when inserting the binomial series $$(||\tilde{X}||_2^2)^{\alpha_{j}^{l}} = \sum_{q=0}^{\infty} (||\tilde{X}||_2^2-1)^q {\alpha_{j}^{l} \choose q} $$
which converges absolutely for any choices of $\alpha_{i}^{l}$ since $||\tilde{X}||_2^2 \in (0,1]$. Thus, we there exits $\hat{\eta}^{l,q}_j \in \mathbb{R}$ such that
\begin{equation}
    \label{eq:ntknotposdef}
     h_{\textrm{NTK}}(\tilde{X},\tilde{X}') = \sum_{j=0}^{\infty} (\tilde{X}^T\tilde{X}')^j \sum_{l = 0}^{\infty} \sum_{q = 0}^{\infty} \hat{\eta}^{l,q}_j (||\tilde{X}||_2^2 -1 )^l (||\tilde{X}'||_2^2 -1 )^q 
\end{equation}
which proves the second point of Assumption \ref{ass:1}. 
\\
\textbf{Step 4:} In this step, we show that the first point of Assumption \ref{ass:1} holds true, i.e. that $g$ from Equation \ref{eq:ntkproof} is Lipschitz continuous on $\Omega_B := \{(x,x,x) | x \in [1-\delta,1+\delta]\}$. For this, recall that 
$$\Sigma^{(i)}(\tilde{X},\tilde{X}) = (||\tilde{X}||_2^2)^{k^i}$$ and note that 
$$\dot{\Sigma}^{(i)} = c_{\sigma} (||\tilde{X}||_2^2)^{k^{i-1}(k-1)} \hat{t}_{\dot{\sigma}}\left( 1 \right)  
$$
therefore, we have that 
\begin{equation}
    \begin{split}
        k_{\textrm{NTK}, \tau}(X,X) &=  \sum_{i=1}^{L+1} \Sigma^{(i-1)}(\tilde{X},\tilde{X}) \prod_{j=i}^{L+1} \dot{\Sigma}^{(j)}(\tilde{X},\tilde{X}) \\
        &= \sum_{i=1}^{L+1} (||\tilde{X}||_2^2)^{k^i} \prod_{j=i}^{L+1} c_{\sigma} (||\tilde{X}||_2^2)^{k^{i-1}(k-1)} \hat{t}_{\dot{\sigma}}\left( 1 \right)  
    \end{split}
\end{equation}
Hence, by definition of $g$, we have that for any $x \in [1-\delta, 1+\delta]$,
$$g(x,x,x) = \sum_{i=1}^{L+1} (\frac{x}{\tau})^{k^i} \prod_{j=i}^{L+1} c_{\sigma} (\frac{x}{\tau})^{k^{i-1}(k-1)} \hat{t}_{\dot{\sigma}}\left( 1 \right)  $$
which is Lipschitz continuous since $\delta \leq 1/4$. \\
\textbf{Step 5:} The only thing which is left to show is that $k_{\textrm{NTK},\tau}$ is continuous on the restriction to $|~||X||_2^2 -1 | \leq \delta$, $|~||X'||_2^2 -1 | \leq \delta$. This fact follows trivially when noting that for any $i>0$, $\Sigma^{(i-1)}(X,X')$ and $\dot{\Sigma^{(i)}}(X,X')$ are both concatenations of continuous functions. 
\end{proof}







In order to apply Lemma \ref{lm:ntk1} for the case where $\sigma(x) = \max(0,x)$ is the popular Relu activation function, we need to use the following technical lemma.
\begin{lemma}
\label{lm:taylor}
For any $x \in [-1,1]$, we have that
\begin{enumerate}
    \item $$ \arcsin(x) = \sum_{j=0}^{\infty} \frac{(2j)!}{(2^j j!)^2} \frac{x^{2j+1}}{2j+1}$$\\
    \item $$\sqrt{1-x^2} + x \arcsin(x) = 1+ \frac{x^2}{2} + \sum_{j=1}^{\infty} \frac{ x^{2j+2}(j!)^2  }{2^{2j+1} (1/2-1)\dots(1/2-j)(2^j j!)^2 (2j+1) (j+1)!}  $$
\end{enumerate}
In particular, both series converge absolutely for any $x \in [-1,1]$.
\end{lemma}
\begin{proof}
The first equation is a well known to have a convergence radius of $1$. In particular, it is well known that $\sum_{j=0}^{\infty} \frac{(2j)!}{(2^n n!)^2 \frac{x^{2n+1}}{2n+1}}$ exists for $x = 1$. Because all the coefficients are positive, this implies that the series converges also absolutely for the cases $x=1$ and $x= -1$. \\ 
For the second case, we can use the binomial series, giving
$$ \sqrt{1-x^2} = \sum_{j= 0}^{\infty} (-x^2)^j { 1/2 \choose j } $$
which converges absolutely for any $x \in [-1,1]$. Hence,
\begin{equation}
    \begin{split}
        \sqrt{1-x^2} + x \arcsin(x) &= \sum_{j=0}^{\infty} \frac{(2j)!}{(2^j j!)^2 }\frac{x^{2j+2}}{2j+1} +(-1)^{j} x^{2j} {  1/2 \choose j } \\
        &= 1 + \sum_{j=0}^{\infty}x^{2j+2} \left( \frac{(2j)!}{(2^j j!)^2 (2j+1)} +(-1)^{j+1} {  1/2 \choose j+1 } \right)
    \end{split}
\end{equation} 
converges also absolutely for any $x \in [-1,1]$.
We can further simplify
\begin{equation}
\label{eq:temp1}
    \begin{split}
         & \frac{(2j)!}{(2^j j!)^2 (2j+1)} +(-1)^{j+1} {  1/2 \choose j+1 } = \frac{(2j)!}{(2^j j!)^2 (2j+1)} +(-1)^{j+1} \frac{(1/2)(1/2-1)\dots(1/2-j)}{(j+1)!}\\
         &= \frac{(2j)!(j+1)! + (-1)^{j+1}  (1/2)(1/2-1)\dots(1/2-j) 
        (2^j j!)^2 (2j+1)   }{(2^j j!)^2 (2j+1) (j+1)!} \\
         &= (j!)^2 \frac{\frac{(j+1) \dots (2j)}{(2^j j!)^2 (1/2-1)\dots(1/2-j)} (j+1) +(-1)^{j+1}
         \frac{2j+1}{2} }{4^j (1/2-1)\dots(1/2-j)(2^j j!)^2 (2j+1) (j+1)!}
    \end{split}
\end{equation}
for $j = 0$ the term gives $1/2$. The goal is now to show that for any $j>0$, $\frac{(j+1) \dots (2j)}{(2^j j!)^2 (1/2-1)\dots(1/2-j)}  = (-1)^{j}$. We proof by induction. Clearly, the case where $j = 1$ holds true. Next, note that
$$
\frac{(j+2) \dots (2j) (2j+1) (2j+2)}{4^j 4 (1/2-1)\dots(1/2-j) (1/2 - j-1)} = \frac{(j+1) \dots (2j) }{4^j (1/2-1)\dots(1/2-j)}  \frac{(2j+1)(2j+2)}{4(j+1) (1/2-j-1)} = (-1)^{j+1}
$$
Using the trivial fact that $(-1)^j$ has the same signature as $(1/2-1)\dots(1/2-j)$, Equation \ref{eq:temp1} becomes
$$ = (j!)^2 \frac{(j+1) - \frac{2j+1}{2} }{4^j (1/2-1)\dots(1/2-j)(2^j j!)^2 (2j+1) (j+1)!}$$
and therefore,
$$        \sqrt{1-x^2} + x \arcsin(x) = 1+ \frac{x^2}{2} + \sum_{j=1}^{\infty} x^{2j+2}(j!)^2 \frac{(j+1) - \frac{2j+1}{2} }{4^j (1/2-1)\dots(1/2-j)(2^j j!)^2 (2j+1) (j+1)!}  \\
$$
which completes the proof. 
\end{proof}
We are finally ready to give the proof for Corollary \ref{cr:ntk2}. 
\begin{proof}[Proof of Corollary \ref{cr:ntk2}]
In a first step, we show that the assumptions in Lemma \ref{lm:ntk1} are satisfied, which implies that the assumptions in Proposition \ref{prop:elkarouiextension} are also satisfied for $k_{\textrm{NTK},\tau}$. The only thing which is then left to show that the empirical kernel matrix $K$ with entries $K_{i,j} = k_{\textrm{NTK},\tau}(X_i,X_j)$ has almost surely asymptotically positive non zero lower bounded Eigenvalues.  We prove this by showing the Assumptions from Corollary \ref{cr:posdef} hold true. In particular, we need to show that every $g_i$ from Equation \ref{eq:gi} from the proof of Lemma \ref{lm:ntk1} is positive definite. The proof follows then when observing that for all $i$, $g_i(1,1) > 0$. \\\\
We begin with some facts from \cite[Lemma~E.1]{Arora19}, where it is shown that
$$\hat{t}_{\sigma}(\rho) = \frac{\sqrt{1-\rho^2} + \rho \arcsin(\rho)}{\pi}$$
and
$$ \hat{t}_{\dot{\sigma}}(\rho) = \frac{1}{2} +\frac{\arcsin(\rho)}{\pi}$$
In addition, it is shown that $c_{\sigma}=2$. Note that the image of $\hat{t}_{\sigma}$ is contained in $[-1/2,1/2] = [-1/c_{\sigma}, 1/c_{\sigma}]$. Finally, the Assumptions from Lemma \ref{lm:ntk1} hold follow form Lemma \ref{lm:taylor}. Hence, it is only left to show that Corollary \ref{cr:posdef} applies. For this, note that any coefficients in the power series form Lemma \ref{lm:taylor} are positive. As a consequence, we can see that any coefficient  the sum of Equation \ref{eq:posdefntk} is positive $\eta_{i}^{l} >0$. Note that the same does not necessarily hold true for $\hat{\eta}_i^l$ in Equation \ref{eq:ntknotposdef} since the coefficients of the Binomial series ${ \alpha_i^l \choose l}$ can be negative. We can then conclude the proof by showing that $\eta_{i}^{l} >0$ implies that the function
$$
  g_j(||X||_2^2,||X'||_2^2) =  \sum_{l \in I_{j}} \eta_{j}^l (||\frac{1}{\tau} X ||_2^2)^{\alpha_{j}^{l}} (||\frac{1}{\tau} X'||_2^2)^{\alpha_{j}^{l}})
  $$
  is positive definite and $g_j(1,1) >0$. In a first step, since $\eta_{i}^{l} >0$, we can define 
  $$ h^{l}_j(x) = \sqrt{\eta_{j}^l} (x)^{\alpha_{j}^{l}} $$
  and note that 
  $$ \eta_{j}^l (||\frac{1}{\tau} X ||_2^2)^{\alpha_{j}^{l}} (||\frac{1}{\tau} X'||_2^2)^{\alpha_{j}^{l}}) = h^{l}_j(||X||_2^2) h^{l}_j(||X'||_2^2)$$
  It is now straight forward to verify that $h(x,x') = h^{l}_j(x) h^{l}_j(x')$ is a positive definite function for every $x \neq 0, x' \neq 0$. It is well known that any finite sum of positive definite kernels is again a positive definite kernel. Due to the fact that the sum in the expression of $g_j$ converges absolutely and because positive definiteness is a non strict inequality, we note that the statement holds also true if the sum is over an countable index set $I_j$. Finally, we have 
  $$g(1,1)= \sum_{l \in I_{j}} \eta_{j}^l > 0$$
  which concludes the proof. 
\end{proof}
