# Supplementary material for: How rotational invariance of common kernels prevents generalization in high dimensions
Source: arXiv:2104.04244 source file (2021-04-09)
Supplement: Supplementary file 13 [file Appendix_Section3.tex]

\section{Proofs Section \ref{sec:norm}}
\begin{proof}[Proof of Lemma \ref{lm:norm}]
 Let $\overline{f}_{l,j}$ be the Fourier series coefficients of $\overline{f}_l$, i.e. for any $X \in [0,1]$ and any $l \leq m$
$$\overline{f}_l(X) = \sum_{j = -\infty}^{\infty} f_{j} \exp(2\pi i j X)) $$ 
Following a similar argumentation as in \cite[Proposition~12.24]{Wainwright19}, it is not difficult to see that 
$$  \langle f,f\rangle_k = \prod_{l = 1}^m \left( \sum_{j=-\infty}^{\infty} \frac{f_{l,j}^2}{q^d_j} \right) \prod_{l = m+1}^d \frac{1}{q^d_0} $$
and because $f$ is assumed to be non linear, there exists some $f_{\hat{l},\hat{j}}^2 > 0$ with $\hat{j} \neq 0$ and $\hat{l} \leq m$. Since $f$ is by assumption not the zero function and $m$ is constant, there exists a constant $c >0$ independent of $d$, such that 
$$  \langle f,f\rangle_k \geq  c \frac{f_{\hat{l},\hat{j}}^2}{q^d_{\hat{j}}} \prod_{l = m+1}^d \frac{1}{q^d_0} $$
We can now show by contradiction this term goes to infinity as $d$ increases. Assume that there exists a constant $M$ such that for every $d \geq m$, $ c \frac{f_{\hat{l},\hat{j}}^2}{q^d_{\hat{j}}} \prod_{l = m+1}^d \frac{1}{q^d_0} \leq M $. Since any $q_j^d \leq 1$, we have that $c \frac{f_{\hat{l},\hat{j}}^2}{q^d_{\hat{j}}} \geq c f_{\hat{l},\hat{j}}^2$, and therefore, we require that $\left(\frac{1}{q^d_0} \right)^{d-m} \leq  \frac{M}{c f_{\hat{l},\hat{j}}^2} $, which implies that 
$ q_0^d \geq \left( \frac{c f_{\hat{l},\hat{j}}^2}{M} \right)^{\frac{1}{d-m}} $
However, since $q^d_{\hat{j}} \leq 1 - q^d_0  \leq 1-\left( \frac{c f_{\hat{l},\hat{j}}^2}{M} \right)^{\frac{1}{d-m}} $,
$ \frac{f_{\hat{l},\hat{j}}^2}{q^d_{\hat{j}}} \geq\frac{f_{\hat{l},\hat{j}}^2}{1 -  \left( \frac{c f_{\hat{l},\hat{j}}^2}{M} \right)^{\frac{1}{d-m}} }$, which goes to infinity because $  \frac{c f_{\hat{l},\hat{j}}^2}{M}  \to 0$ as $d \to \infty$. Hence, we can conclude the proof.
\end{proof}
