# Supplementary material for: How rotational invariance of common kernels prevents generalization in high dimensions
Source: arXiv:2104.04244 source file (2021-04-09)
Supplement: Supplementary file 14 [file Appendix_Section4.1.tex]

\section{Proofs Section \ref{sec:lowerboundofEV}}

\subsection{Proof of Proposition \ref{prop:elkarouiextension}}
\begin{proof}
The proposition is actually a consequence of Lemma \ref{lm:innerpr}. Inspired by \cite{el2010spectrum}, we separately analyse the off and on diagonal terms of $K$. Let $A$ be the off diagonal matrix of $K$, with diagonal entries $A_{i,j} = (1- \delta_{i,j}) K_{i,j}$ and let $D$ be the diagonal matrix of $K$ with entries $D_{i,j} = \delta_{i,j} K_{i,j}$. \\
We can now make use of Remark \ref{rm:kalmostsureg}:
\begin{equation}
    \begin{split}
    \forall i ~~ D_{i,i} := K_{i,i} = g(||X_i||_2^2, ||X_i||_2^2,X_i^TX_i) ~~a.s.
    \end{split}
\end{equation}
Furthermore, due to Assumption \ref{ass:1}, we can express $A$ using the Taylor series expansion of $g_i$ around the point $(1,1)$:
\begin{equation}
    \begin{split}
    \forall i\neq j ~~ A_{i,j} &:=  \sum_{m=0}^{\infty} (X_i^TX_j)^m g_m(||X_i||_2^2,||X_j||_2^2)\\ 
    &= \sum_{m =0}^p (X_i^TX_j)^{m} \sum_{ l_1+l_2 \leq p-m} \frac{ g_{m}^{(l_1,l_2)}(1,1)}{l_1
    ! l_2!} (X_i^TX_i -1 )^{l_1} (X_j^TX_j -1 )^{l_2}   \\ 
    &+ \sum_{m =0}^{p}(X_i^TX_j)^{m} \sum_{ l_1+l_2  = p+1-m} \frac{ g_{m}^{(l_1,l_2)}(\eta^{m,i,j}_{l_1,l_2})}{l_1
    ! l_2!} (X_i^TX_i -1 )^{l_1} (X_j^TX_j -1 )^{l_2}   \\ 
    &+ (X_i^TX_j)^{p+1} \sum_{m =p+1}^{\infty}  (X_i^TX_j)^{m-(p+1)} g_{m}(||X_i||_2^2,||X_j||^2_2)    ~~ a.s.\\ 
        \end{split}
\end{equation}
where $\eta^{m,i,j}_{l_1,l_2}$ are contained in the closed ball $\eta^{m,i,j}_{l_1,l_2} \in B_r((1,1))$ around the point $(1,1)$ with radius $r^2 = (||X_i||_2^2-1)^2 + (||X_j||_2^2-1)^2 \to 0~~a.s.$, where the convergence to zero is by Lemma \ref{lm:innerpr}. Hence, using the fact that $g_i$ is $p+1-i$-times continuously differentiable,  we can see that $g_{m}^{(l_1,l_2)}(\eta^{m,i,j}_{l_1,l_2})$ is almost surely bounded by some constant. \\
The remaining proof is separated into three steps. In a first and second step, we find matrices $M_A$ and $M_D$ such that $||A- M_A||_2\to 0$ and $||D- M_D||_2$,  both depending only on polynomials of $X_i^TX_j$ up to the degree $p$. Finally, in a third step, we combine $M_A$ and $M_D$ in order to reach the desired expression for $M$ given in Proposition \ref{prop:elkarouiextension}. \\\\
\textbf{Step 1:}
Let 
\begin{equation}
    M_D := g(1,1,1)~ \mathrm{I}_n. 
\end{equation} Because $D-M_D$ is a diagonal matrix, we have that 
\begin{equation}
    ||D - M_D||_2 = \max_{i} |g(||X_i||_2^2, ||X_i||_2^2,X_i^TX_i) - g(1,1,1)|  \leq L \sqrt{3} (||X_i||_2^2 -1) ~~ a.s..
\end{equation}
Where we have used that by Assumption \ref{ass:1}, $g$ is $L$-Lipschitz continuous on the restriction $\{(x,x,x) | x \in [1-\delta, 1+ \delta]\} \subset \Omega$. Finally, due to Lemma \ref{lm:innerpr}, we can see that this term goes to zero almost surely and thus,
$$ ||D - M_D||_2 \to 0$$
as desired. \\ \\
\textbf{Step 2:} 
Let $ M_A$ be the off diagonal matrix with entries
\begin{equation}
    \forall i\neq j ~~~ (M_A)_{i,j} := \sum_{m =0}^p (X_i^TX_j)^{m} \sum_{ l_1+l_2 \leq p-m} \frac{ g_{m}^{(l_1,l_2)}(1,1)}{l_1
    ! l_2!} (X_i^TX_i -1 )^{l_1} (X_j^TX_j -1 )^{l_2} . 
\end{equation}
The goal of this step is to show that 
\begin{equation}
    ||M_A - A||_2 \leq ||M_A - A||_F \to n \underset{i,j}{\max} |M_{A,i,j} - A_{i,j} | \to 0.
\end{equation} \\
We have
\begin{equation}
    \begin{split}
         ||M_A - A ||_F &\leq n \max_{i\neq j} \left[ \underbrace{\left|\sum_{m =0}^{p} (X_i^TX_j)^{m} \sum_{ l_1+l_2  = p+1-m} \frac{ g_{m}^{(l_1,l_2)}(\eta^{m,i,j}_{l_1,l_2})}{l_1
    ! l_2!} (X_i^TX_i -1 )^{l_1} (X_j^TX_j -1 )^{l_2}  \right|}_{=: B_1^{i,j}} \right] \\ &+ n \max_{i\neq j}\left[\underbrace{ \left|
     (X_i^TX_j)^{p+1} \sum_{m =p+1}^{\infty}(X_i^TX_j)^{m-(p+1)} g_{m}(||X_i||_2^2,||X_j||^2_2)   \right| }_{=: B_2^{i,j}}\right] ~~ a.s.\\ 
    \end{split}
\end{equation}
First, we show that the term $n B^{i,j}_1 \to 0$. Note that due to the above discussion, we know $g_{m}^{(l_1,l_2)}(\eta^{m,i,j}_{l_1,l_2})$ is almost surely upper bounded by some constant. Furthermore, since $i \neq j$, we can apply Lemma \ref{lm:innerpr} which shows that for any positive $m,l_1$ and $l_2$ such that $m+l_1+l_2 = p+1$,
\begin{equation}
\label{eq:weneedp}
    \left| (X_i^TX_i -1 )^{l_1} (X_j^TX_j -1 )^{l_2} (X_i^TX_j)^{m}\right| \leq (n^{-\beta/2}log(n)^{1+\epsilon})^{p+1} ~~~ a.s.
\end{equation}
which holds true for any positive constant $\epsilon >0$. Finally, because $p = \floor{2/\beta}$, we have that $(\beta/2)(p+1) > 1$. Therefore,  
\begin{equation}
    \label{eq:weneedp}
    n \max_{i\neq j} B^{i,j}_1 \lesssim (n^{-\beta/2}log(n)^{1+\epsilon})^{p+1} \to 0~~a.s..
\end{equation} 
Next, note that we have not made the assumption that the series from Equation \ref{eq:g} converges absolutely. However, since $\Omega$ is a compact set and because $g$ is a continuous function, there exists some constant $C_G>0$ such that $\forall x,y,z \in \Omega: |g(x,y,z)| \leq C_G$. Hence, for any $j \geq 0$, there exists a constant $C_{j} >0 $ such that for all $x,y,z \in \Omega$,
\begin{equation}
    g(x,y,z) = \sum_{i=0}^{j-1} z^i g_i(x,y) + z^j \sum_{i=j}^{\infty} z^{i-j}g_i(x,y) \leq \sum_{i=0}^{j-1} z^i g_i(x,y) + z^j  C_{j}.
\end{equation}
As a consequence, we have that 
\begin{equation}
    \label{eq:weneedp2}
     \left|\sum_{m =p+1}^{\infty} g_{m}(||X_i||_2^2,||X_j||^2_2)   (X_i^TX_j)^{m-p+1}\right| \leq C_{p+1} ~~~ a.s.,
\end{equation}
and therefore, 
\begin{equation}
    \label{eq:weneedp2}
n \max_{i\neq j} B^{i,j}_2 \leq n \max_{i\neq j} \left| (X_i^TX_j)^{p+1} \right| C_{S,p+1} \lesssim  \left(n^{-\beta/2}log(n)^{1+\epsilon}\right)^{p+1} ~~~ a.s. \to 0,
\end{equation}
where we have again used Lemma \ref{lm:innerpr}. As a result, we can conclude the second step of the proof. \\\\
\textbf{Step 3:} Combining step 1 and 2, we get that 
\begin{equation}
    ||A+D - M_A - M_D ||_2 \to 0
\end{equation}
While $M_A$ and $M_D$ are already both only dependent on polynomials of $X_i^TX_j$ up to degree $p$, the goal of this step is to further simplify in order to obtain the expression for $M$ from Equation \ref{eq:elkarouiM}. Define $\tilde{D}$ to be the diagonal matrix with entries
\begin{equation}
\tilde{D}_{i,i} := \sum_{m =0}^p \sum_{ l_1+l_2 \leq p-m} \frac{ g_{m}^{(l_1,l_2)}(1,1)}{l_1
    ! l_2!} (X_i^TX_i -1 )^{l_1} (X_i^TX_i -1 )^{l_2} (X_i^TX_i)^{m} 
    \end{equation}
We have that
\begin{equation*}
    \begin{split}
       \tilde{D}_{i,i} - \sum_{m =0}^p g_m(1,1)  \leq
         \sum_{m =0}^p  \left| g_{m}(1,1) \left[(X_i^TX_i)^{m} -1 \right]\right|
        \\ + \sum_{m =0}^p \sum_{ 1\leq l_1+l_2 \leq p-m} \left|\frac{ g_{m}^{(l_1,l_2)}(1,1)}{l_1
    ! l_2!} (X_i^TX_i -1 )^{l_1} (X_i^TX_i -1 )^{l_2} (X_i^TX_i)^{m} \right|
    \end{split}
\end{equation*}
Following the same discussion as in the first part of the proof, it is easy to see that 
\begin{equation}
\sum_{m =0}^p \sum_{ 1\leq l_1+l_2 \leq p-m} \left|\frac{ g_{m}^{(l_1,l_2)}(1,1)}{l_1
    ! l_2!} (X_i^TX_i -1 )^{l_1} (X_i^TX_i -1 )^{l_2} (X_i^TX_i)^{m} \right| \to 0
    \end{equation}
    Furthermore, using Corollary \ref{cr:concentrationh}, we can also see that 
    \begin{equation}
\sum_{m =0}^p  \left| g_{m}(1,1) \left[(X_i^TX_i)^{m} -1\right] \right| \to 0
\end{equation}
     and hence, we get that
\begin{equation}
||\tilde{D} - \textrm{I}_n\left( \sum_{m =0}^p g_m(1,1)  \right)||_2 \to 0
\end{equation}
     Hence, we find that
\begin{equation}
 || K -  \underbrace{ \left[ M_A +M_D + \tilde{D} -  \textrm{I}_n \left( \sum_{m =0}^p g_m(1,1)  \right) \right] }_{=:M}||_2 \to 0
 \end{equation}
    Putting everything together, we have
\begin{equation}
 M_{i,j} =   \delta_{i,j}\left( g(1,1,1) - \sum_{m =0}^p g_m(1,1)   \right) + \sum_{m =0}^p (X_i^TX_j)^{m} \sum_{ l_1+l_2 \leq p-m} \frac{ g_{m}^{(l_1,l_2)}(1,1)}{l_1
    ! l_2!} (X_i^TX_i -1 )^{l_1} (X_j^TX_j -1 )^{l_2} 
\end{equation}
    which is exactly the expression from Equation \ref{eq:elkarouiM} and thus concludes the proof. 
\end{proof}

\subsection{Proof of Corollary \ref{cr:posdef}}
\begin{proof}
We make use of the same notation as in the proof of Proposition \ref{prop:elkarouiextension}. Let $\tilde{M}$ be the matrix with entries
\begin{align}
    \tilde{M}_{i,j} :=  
    \sum_{m =0}^{p}(X_i^TX_j)^{m} \sum_{ l_1+l_2  = p+1-m} \frac{ g_{m}^{(l_1,l_2)}(\eta^{m,i,j}_{l_1,l_2})}{l_1
    ! l_2!} (X_i^TX_i -1 )^{l_1} (X_j^TX_j -1 )^{l_2}   ~~ a.s.
\end{align}
where $\eta^{m,i,j}_{l_1,l_2}\in \mathbb{R}$ are chosen such that 
\begin{align*}
    K_{i,j} &= \tilde{M}_{i,j} + \sum_{m =0}^p (X_i^TX_j)^{m} \sum_{ l_1+l_2 \leq p-m} \frac{ g_{m}^{(l_1,l_2)}(1,1)}{l_1
    ! l_2!} (X_i^TX_i -1 )^{l_1} (X_j^TX_j -1 )^{l_2}   \\ 
    &+ (X_i^TX_j)^{p+1} \sum_{m =p+1}^{\infty}  (X_i^TX_j)^{m-(p+1)} g_{m}(||X_i||_2^2,||X_j||^2_2)  ~~ a.s.
\end{align*}
In a first step, the goal is to show that $||\tilde{M}||_2 \to 0$. We already know form the proof of Proposition \ref{prop:elkarouiextension} that this is true for the off diagonal matrix of $\tilde{M}$. Hence, we only need to show that $||D_{\tilde{M}}||_2 \to 0$, where $D_{\tilde{M}}$ is the diagonal matrix of $\tilde{M}$. However, again using the same argumentation as in the proof of Proposition \ref{prop:elkarouiextension} and by the fact that $ l_1+l_2 \geq 1$, we can see that
\begin{equation}
    \sum_{m =0}^{p} \sum_{ l_1+l_2  = p+1-m} \left|  \frac{ g_{m}^{(l_1,l_2)}(\eta^{m,i,j}_{l_1,l_2})}{l_1
    ! l_2!} (X_i^TX_i -1 )^{l_1+l_2} (X_i^TX_i)^{m} \right| \to 0
\end{equation}
from which the claim follows. Therefore, we have that 
\begin{equation}
    || K - (M + \tilde{M})||_2 \to 0
\end{equation}
Next, note that we have
\begin{equation}
    M + \tilde{M} =  \textbf{I}_n\left(g(1,1,1)  - \sum_{i =0}^p g_i(1,1) \right) +  \sum_{i=0}^p (\textbf{X}^T\textbf{X})^{\circ i} \circ K_{g_i}
\end{equation}
with $K_{g_m}$ the matrix with entries $K_{g_m, i,j} = g_m(||X_i||_2^2, ||X_j||_2^2)$, which is positive semi definite since $g_m$ is a positive definite function by assumption. Hence, by Schur's Product Theorem, we get that $ (\textbf{X}^T\textbf{X})^{\circ i} \circ K_{g_i}$ is positive semi definite, and therefore, 
\begin{equation}
    M + \tilde{M} \succeq \textbf{I}_n\left(g(1,1,1)  - \sum_{i =0}^p g_i(1,1) \right). 
\end{equation}
The proof then follows from the fact that $g(1,1,1) = \sum_{i =0}^{\infty} g_i(1,1) >\sum_{i =0}^p g_i(1,1) $, which holds true since by assumption $g_i \geq 0$ and there exists $j \geq p+1$ such that $g_j >0$.
\end{proof}


\subsection{Proof of Lemma \ref{lm:alphaexp}}
We start with a well known technical lemma 
\begin{lemma}
\label{lm:usefulint}
For all $t\geqslant0$ and $0<\alpha<2$,
$$t^{\alpha}=c_\alpha\int_0^\infty(1-e^{-t^2x^2})x^{-1-\alpha}\df x$$
with 
$$c_\alpha:=\left(\int_0^\infty(1-e^{-x^2})x^{-1-\alpha}\df x\right)^{-1}>0.$$
\end{lemma}
\begin{proof} For $t=0$, the integral is zero. So it is true. We only need to prove for the case when $t>0$. First, use $1-e^{-t^2x^2}\leqslant t^2x^2$ to imply that the integral exists:
$$0\leqslant\int_0^\infty(1-e^{-t^2x^2})x^{-1-\alpha}\df x\leqslant\int_0^1t^2x^{1-\alpha}+\int_1^\infty x^{-1-\alpha}\df x<\infty.$$
Substitute $y:=tx$, so $t^{-1}\df y=\df x$.
$$\int_0^\infty(1-e^{-t^2x^2})x^{-1-\alpha}\df x =\int_0^\infty(1-e^{-y^2})y^{-1-\alpha}t^{1+\alpha}t^{-1}\df y$$
$$=t^{\alpha}\int_0^\infty(1-e^{-y^2})y^{-1-\alpha}\df y.$$
Hence, the result. 
\end{proof}

For $\alpha \in (0,2)$, let $D^{\alpha}$ be the matrix with entries $D^{\alpha}_{i,j} = ||X_i- X_j||^{\alpha}$. 
\begin{lemma}
\label{lm:alphaexpbound}
The Eigenvalues of $D^{\alpha}$ are bounded away form zero by a positive non zero constant $c>0$ independent of $n$. Hence, $\underset{i \leq n}{\min} \left|\lambda_i(D^{\alpha}) \right| \geq c$. 
\end{lemma}
\begin{proof}
Apply Lemma \ref{lm:usefulint} to $t:=\Vert x_i-x_j\Vert_2^\alpha\geqslant0$:
$$\Vert x_i-x_j\Vert_2^\alpha=c_\alpha\int_0^\infty(1-e^{-x^2\Vert x_i-x_j\Vert_2^2})x^{-1-\alpha}\df x$$
Take any $\mu \in\mathbb{R}^n$ with $\sum_{1\leqslant i\leqslant n}\mu_i=0$. Then, 
 \begin{align*}
    \mu^T D^{\alpha} \mu = \sum_{1\leqslant i,j\leqslant n}\Vert x_i-x_j\Vert_2^\alpha\mu_i\mu_j & = \sum_{1\leqslant i,j\leqslant n}\mu_i\mu_jc_\alpha\int_0^\infty(1-e^{-x^2\Vert x_i-x_j\Vert_2^2})x^{-1-\alpha}\df x\\
    & = -c_\alpha\int_0^\infty x^{-1-\alpha} \sum_{1\leqslant i,j\leqslant n}\mu_i\mu_j e^{-x^2\Vert x_i-x_j\Vert_2^2}\df x
\end{align*}
Next, note that we already know from Corollary \ref{cr:posdef} and the subsequent discussion, that the minimum Eigenvalue of the kernel matrix $K$ of the Gaussian kernel is lower bounded $\lambda_{min}(K) \geq c_G > 0$ by some positive non zero constant, independent of $n$. Hence, we have that for every $x \in \mathbb{R}_+$, $\sum_{1\leqslant i,j\leqslant n}\mu_i\mu_j e^{-x^2\Vert x_i-x_j\Vert_2^2} \geq c_{G,x} > 0$. Where $c_{G,x}$ is some positive constant independent of $n$. Thus, we can conclude that there exists a constant $\tilde{c} >0 $ independent of $n$, such that 
$$\mu^T D^{\alpha} \mu \leq \tilde{c}$$
The proof then follows from the Max-Min Theorem and the fact that $\trace(D^{\alpha}) = 0$. 
\end{proof}

\begin{proof}[Proof of Lemma \ref{lm:alphaexp}]
For simplicity, we show that the result holds true for $\tau_0 = 1$. It is then not difficult to see that it holds also true for the more general case where $\tau_0 >0$ is some constant. In a first step, we note that we already know from Lemma \ref{lm:alphaexpbound} that the Eigenvalues of the matrix $D^{\alpha}$ are all bounded away from zero by some constant $c_{\alpha} >0$ independent of $n$. The goal of this proof is to make use of this fact in order to show the desired result. The proof is separated in several steps. In a first step, we construct a kernel positive definite kernel $\tilde{k}$ such that $\exp(-||X-X'||^{\alpha}) = \exp(\tilde{k}(X,X')) \exp(-||X-X'||^{\alpha} - \tilde{k}(X,X')) $ and $\exp(-||X-X'||^{\alpha} - \tilde{k}(X,X')) $ is a positive definite function. Then, we show that the Eigenvalues of the kernel matrix of $\exp(\tilde{k}(X,X'))$ are lower bounded and finally, in a last step, we show that this implies that the Eigenvalues of the kernel matrix of $\exp(-||X-X'||^{\alpha})$ are lower bounded. \\\\
\textbf{Step 1:}
Let $d_{\alpha} = ||X-X'||^{\alpha}$. We know from 
\cite[Chapter~3,Theorem~2.2]{Berg84} that this is a conditionally negative definite function, i.e. for every $v \in \mathbb{R}^n$ with $1^T v = 0$, $v^T D^{\alpha}v \geq 0$. As shown in \cite[Chapter~3,Lemma~2.1]{Berg84}, a kernel function $\phi(X,X')$ is conditionally negative definite, if and only if for any $X_0$, $ \phi(X,X_0) + \phi(X_0,X') -\phi(X,X') - \phi(X_0,X_0)$ is a positive definite function. Hence, we know that  $ d_{\alpha}(X,0) + d_{\alpha}(X_0,X') -d_{\alpha}(X,X') - d_{\alpha}(X_0,X_0)$ is positive definite. Let $A$ be the corresponding kernel matrix evaluated at $\textbf{X}$. It is shown in the proof of \cite[Chapter~3,Lemma~2.1]{Berg84} that for any $v \in \mathbb{R}^n$,
$$ - v^T A v = \begin{pmatrix}v \\ - 1^Tv\end{pmatrix} \begin{pmatrix} D^{\alpha} & d_{\alpha}(X_0, \textbf{X}) \\ d_{\alpha}(X_0, \textbf{X})^T & d_{\alpha}(X_0,X_0) \end{pmatrix}\begin{pmatrix}v \\ - 1^Tv\end{pmatrix} \leq 0
$$
where $d_{\alpha}(X_0, \textbf{X})$ is the vector with entries $d_{\alpha}(X_0, \textbf{X})_i = d_{\alpha}(X_i,X_0)$. Note that inequality $\leq 0$ follows from the fact that $d_{\alpha}$ is conditionally negative definite and $1^T \begin{pmatrix}v \\ - 1^Tv\end{pmatrix} = 0$. The issue now is that even when the matrix $\begin{pmatrix} D^{\alpha} & d_{\alpha}(X_0, \textbf{X}) \\ d_{\alpha}(X_0, \textbf{X})^T & d_{\alpha}(X_0,X_0) \end{pmatrix}$ has Eigenvalues bounded away from zero, we can not conclude that this is also the case for $A$. The reason is because the vector $v = \frac{1}{\sqrt{n}} 1$ has $||v||_2 = 1$ but $1^T v = \sqrt{n}$. Thus, this would only imply that $- v^T A v \leq \frac{-c}{n}$. \\
The goal is now to construct a kernel function $\tilde{k}$ based on the same idea which, however, satisfies $- v^T A v \leq c$ for some constant $c>0$ and $A$ again the kernel matrix of $\tilde{k}$ evaluated at $\textbf{X}$. In a first step, note that we can extend the proof of Lemma \ref{lm:innerpr} to see that there exists almost surely with respect to the draws of $\textbf{X}$ a set of $n$ vectors $\tilde{\textbf{X}}$, such that for any two vectors $X,X' \in \textbf{X} \cup \tilde{\textbf{X}}$, we have that
\begin{equation}
\label{eq:tmpconineq}
    | X^TX' - \delta_{X = X'} | \leq n^{-\beta/2} \log(n)^{1+\epsilon} 
\end{equation}
Next, note that because $\textbf{X} \cup \tilde{\textbf{X}}$ are in total $2 n$ vectors, we can use the proof of Lemma \ref{lm:alphaexpbound} to the find there exists some constant $c_{\lambda} > 0$ independent of $n$ such that for any $v \in \mathbb{R}^{2n}$ with $||v||_21$ and $1^T v = 0$, 

$$v^T  \begin{pmatrix} D^{\alpha} & D^{\alpha}(\tilde{\textbf{X}}, \textbf{X}) \\ D^{\alpha}(\tilde{\textbf{X}}, \textbf{X})^T & \tilde{D}^{\alpha} \end{pmatrix} v \leq -c_{\lambda}$$ 
with $\tilde{D}^{\alpha}$ and $D^{\alpha}(\tilde{\textbf{X}}, \textbf{X})$ both $n \times n$ matrices with entries $\tilde{D}^{\alpha} = d_{\alpha}(\tilde{X}_i, \tilde{X}_j)$ and $D^{\alpha}(\tilde{\textbf{X}}, \textbf{X})_{i,j} = d_{\alpha}(\tilde{X}_i,X_j)$. We can now define the linear map $-A: \mathbb{R}^n \to \mathbb{R}^n$ by 
$$ v \to  \begin{pmatrix} D^{\alpha} & D^{\alpha}(\tilde{\textbf{X}}, \textbf{X}) \\ D^{\alpha}(\tilde{\textbf{X}}, \textbf{X})^T & \tilde{D}^{\alpha} \end{pmatrix} \begin{pmatrix} v \\ -\frac{1}{n} 1^T v 1 \end{pmatrix} $$
and using the fact that $1^T \begin{pmatrix} v \\ -\frac{1}{n} 1^T v 1 \end{pmatrix} = 0 $, we
find that for any $v \in \mathbb{R}^n$, 
$$ v ^T-A v \leq \frac{c}{v^T v + \frac{1}{n^2} 1^T v 1  1^T v 1} = \frac{-c}{v^T v + \frac{1}{n^2} v^T 1^T 1 1^T1 v} \leq \frac{-c/2}{v^T v}$$
Therefore, due to the Min-Max Theorem, we find that the maximum Eigenvalue of $\lambda_{max}(-A) \leq -c/2$ and therefore, $\lambda_{min}(A) \geq c/2$. The only thing left in the first step of this proof is to find the kernel matrix $\tilde{k}$ generating $A$. We have that
\begin{equation}
    \begin{split}
        -w^T Av &= \begin{pmatrix} w \\ -\frac{1}{n} 1^T w 1 \end{pmatrix}  \begin{pmatrix} D^{\alpha} & D^{\alpha}(\tilde{\textbf{X}}, \textbf{X}) \\ D^{\alpha}(\tilde{\textbf{X}}, \textbf{X})^T & \tilde{D}^{\alpha} \end{pmatrix} \begin{pmatrix} v \\ -\frac{1}{n} 1^T v 1 \end{pmatrix} \\
                &= w^T D^{\alpha} v - w^T \left[\frac{1}{n} 1 1^TD^{\alpha}(\tilde{\textbf{X}}, \textbf{X}) \right] v - w^T \left[ \frac{1}{n} D^{\alpha}(\tilde{\textbf{X}}, \textbf{X})^T 1 1^T \right] v  + w^T \left[ \frac{1}{n^2} 1 1^T \tilde{D}^{\alpha} 1 1^T \right] v
            \end{split}
\end{equation} 
We can thus see that $A$ is obtained when evaluating the kernel function 
$$\tilde{k}(X,X') := \frac{1}{n} \sum_{i =1}^n d_{\alpha}(X,X_i) + d_{\alpha}(X_i,X') - \frac{1}{n^2} \sum_{i,j=1}^{n} \left(d_{\alpha}(X_i,X_j)  - d_{\alpha}(X,X') \right)$$
at $\textbf{X}$. 
\\\\
\textbf{Step 2:}
We have that $\exp(-d_{\alpha}(X,X')) = \exp(\tilde{k}(X,X')) \exp(-d_{\alpha}(X,X') - \tilde{k}(X,X')) $, with $\phi(X,X') := -d_{\alpha}(X,X') - \tilde{k}(X,X') = \frac{1}{n^2} \sum_{i,j=1}^{n} d_{\alpha}(X_i,X_j)  - \frac{1}{n} \sum_{i =1}^n \left(d_{\alpha}(X,X_i) - d_{\alpha}(X_i,X') \right)$. Next, note that $\exp(\phi(X,X'))$ is a positive definite function. Hence, by Schur's product Theorem, we have that
$$ exp(-d_{\alpha}(X,X')) = \exp(\tilde{k}(X,X')) \exp(\phi(X,X')) = \sum_{l=0}^{\infty} \frac{1}{l!} \tilde{k}(X,X')^l \exp(\phi(X,X')) $$
is a sum of positive definite functions. Therefore, it is sufficient to show that the Eigenvalues of the kernel matrix $M$ of $\tilde{k}(X,X') \exp(\phi(X,X'))$, evaluated at $\textbf{X}$, are lower bounded. Let $B$ be the kernel matrix of $\exp(\phi(X,X'))$ evaluated at $\textbf{X}$, we have that $M = A \circ B$, where $\circ$ is the Hadamard product. We make the following Claim, from which the proof follows trivially using the fact from the first step that the Eigenvalues of $A$ are lower bounded by a positive non zero constant.
\\\\
\textbf{Claim:} $B = 1/2 11^T + \tilde{B}$ with $\tilde{B}$ a positive definite matrix. 
\\\\
\textbf{Step 3: Proof of the Claim} The only thing which is left to conclude the proof is to show that the Claim holds true. Let $\psi$ be the vector with entries $\psi_i = \exp(- \frac{1}{n} \sum_{j=1}^n -d_{\alpha}(X_i,\tilde{X}_j))$. Furthermore, let $\gamma = \exp(\frac{1}{n^2} \sum_{i,j=1}^{n} d_{\alpha}(\tilde{X}_i, \tilde{X}_j))$. We can write
$$ B = \gamma \left(1 \psi^T\right) \circ \left( \psi 1^T \right) = \gamma \psi \psi^T$$
Next, due to Equation \ref{eq:tmpconineq}, we can see that $$ \left| 2^{\alpha/2} - \frac{1}{n^2} \sum_{i,j=1}^{n} d_{\alpha}(\tilde{X}_i, \tilde{X}_j)) \right| \leq \frac{(n^2-n) n^{-\beta/2}\log(n)^{1+\epsilon} + n}{n^2} \to 0 ~~~a.s. $$
where we have used the fact that $d_{\alpha}(X,X') =  2^{\alpha/2} + O(\frac{||X-X'||_2^2}{2} -1 )$.  Thus, $ \gamma \geq \exp( 2^{\alpha/2}/2) >1 ~~a.s.$, and hence, it is sufficient to show that $  \psi \psi^T - \frac{1}{2} ~ 1 1^T $ is positive definite. However, this is true if and only if $1^T \psi \psi^T 1 \geq \frac{1}{2} 1 1^T 1 1^T$, which is equivalent to saying that $ \sum_{i,j}^n  d_{\alpha}(X_i, \tilde{X}_j) \geq \frac{n^2}{2}$. However, using again the same argument as for $\gamma$, we can see that $\left|  2^{\alpha/2} - \frac{1}{n^2} \sum_{i,j}^n  d_{\alpha}(X_i, \tilde{X}_j) \right| \to 0 ~~ a.s.$, which completes the proof.
\end{proof}
