# Supplementary material for: How rotational invariance of common kernels prevents generalization in high dimensions
Source: arXiv:2104.04244 source file (2021-04-09)
Supplement: Supplementary file 15 [file Appendix_Section4.2.tex]

\section{Proof Section \ref{sec:biasbound}}
\subsection{Proof of Theorem \ref{th:main}}

\begin{proof}
Assume that $X^* \in \mathcal{U}$. Hence, we can make use of the following two inequalities:
\begin{equation}
\label{eq:thmainxstar1}
    \max_{i}\left| X_i^TX^*\right| \leq n^{-\beta/2}log(n)^{1+\epsilon} ~~~ a.s.,
\end{equation}
and 
\begin{equation}
\label{eq:thmainxstar2}
    \left| (X^*)^TX^* -1 \right| \leq  n^{-\beta/2}log(n)^{1+\epsilon}. 
\end{equation}
The proof is essentially again based on same ideas as used in the proof of Proposition \ref{prop:elkarouiextension}, i.e. to applying the Taylor expansion and then make use of Lemma \ref{lm:innerpr}. Let $\psi^* = ((X^*)^T X^* -1 ) \textrm{1}$. Following the same argument as in the proof of Proposition \ref{prop:elkarouiextension} and because, we have that
\begin{equation}
    \begin{split}
    \forall i ~~ K^*_{i} &= \sum_{m =0}^p (X_i^TX^*)^{m} \sum_{ l_1+l_2 \leq p-m} \frac{ g_{m}^{(l_1,l_2)}(1,1)}{l_1
    ! l_2!} (X_i^TX_i -1 )^{l_1} ((X^*)^TX^* -1 )^{l_2}   \\ 
    &+ \sum_{m =0}^{p} (X_i^TX^*)^{m} \sum_{ l_1+l_2  = p+1-m} \frac{ g_{m}^{(l_1,l_2)}(\eta^{m,i,j}_{l_1,l_2})}{l_1
    ! l_2!} (X_i^TX_i -1 )^{l_1} (X_j^TX^* -1 )^{l_2}   \\ 
    &+ (X_i^TX_j)^{p+1} \sum_{m =p+1}^{\infty}(X_i^TX^*)^{m-(p+1)} g_{m}(||X_i||_2^2,||X^*||^2_2)     ~~ a.s.\\ 
        \end{split}
\end{equation}
Next, define 
\begin{equation}
    \begin{split}
    M^* :=  \sum_{m =0}^p (X_i^TX^*)^{m}  \sum_{ l_1+l_2 \leq p-m} \frac{ g_{m}^{(l_1,l_2)}(1,1)}{l_1
    ! l_2!} (X_i^TX_i -1 )^{l_1} ((X^*)^TX^* -1 )^{l_2}.
    \end{split}
\end{equation}
Following exactly the same argument as used in the second step of the proof of Proposition \ref{prop:elkarouiextension}, we get that
\begin{equation}
    \sqrt{n} ||K^* - M^*||_2 \leq n \max_{i} |K^* - M^*| \lesssim \left(n^{-\beta/2} \log(n)^{1+\epsilon}\right)^{p+1} \to 0
\end{equation}
Note that this inequality also implies that $||K^* - M^*||_1 \to 0$. Next, note that by assumption $\lambda_{min}(K + \lambda I_n)\geq c >0 ~~a.s.$ is almost surely lower bounded by some non zero positive constant $c$. Therefore,
\begin{equation}
   ||(K + \lambda I_n)^{-1} (K^* - M^*) ||_1 \leq \sqrt{n}||(K + \lambda I_n)^{-1} (K^* - M^*) ||_2 \leq c \sqrt{n} ||K^* - M^*||_2 \to 0 ~~a.s.
\end{equation}
Furthermore, due to Proposition \ref{prop:elkarouiextension} and the fact that $\lambda_{min}(K + \lambda I_n)\geq c >0 ~~a.s.$, we get that 
\begin{equation}
    ||(K + \lambda I_n)^{-1} - (M + \lambda I_n)^{-1}||_2 \to 0~~a.s.
\end{equation}
where $M$ is from Proposition \ref{prop:elkarouiextension}. \\
Finally, note that we have only used Equation \ref{eq:thmainxstar1} and \ref{eq:thmainxstar2} involving $X^*$. Therefore, the convergence holds uniformly for all $X^* \in \mathcal{X}$ and hence, we can conclude the proof. 
\end{proof}

\begin{proof}[Proof of Corollary \ref{cr:biaslimit}]
Let 
\begin{equation}
    \mathcal{P}_l = \left\{ \sum_{j=0}^l\sum_{i=1}^{d} c_{j,i} X[i]^j | c_{j,i} \in \mathbb{R}\right\}
\end{equation}
be the space of polynomials of degree at most $l$. Due to Theorem \ref{th:main} and the subsequent discussion, we find that there exists a polynomial $\hat{p}_{l}$ with $l = 2p = 2 \floor{2/\beta}$ such that for any $X^* \in \mathcal{U}$, 
\begin{equation}
    \underset{X^* \in \mathcal{U}}{\max} ~ |\hat{p}_l(X^*) - \hat{f}_{\lambda}(X^*)| \to 0 ~~a.s.
\end{equation}
Hence, we can conclude that for any $\gamma_1 >0 $ and $n$ sufficiently large, 
\begin{equation}
    \mathbb{E}_{X^*} ~ \textbf{1}_{X^* \in \mathcal{U}}\left[ \hat{f}_{\lambda}(X^*) -f^*(X^*)\right] - \gamma_1 \geq  \mathbb{E}_{X^*} ~ \textbf{1}_{X^* \in \mathcal{U}}\left[ \hat{p}_l(X^*) -f^*(X^*)\right] ~~a.s.
\end{equation}
Next, note that 
\begin{equation}
\begin{split}
        \mathbb{E}_{X^*} \left( f^*(X^*) - \overline{P}_{l,C}(X^*)\right)^2  &\leq \mathbb{E}_{X^*} \textbf{1}_{X^* \in \mathbb{U}} \left( f^*(X^*) - \overline{P}_{l,C}(X^*)\right)^2 + (1-P(\mathcal{U}))2 C \\ 
        &\to \mathbb{E}_{X^*} \textbf{1}_{X^* \in \mathbb{U}} \left( f^*(X^*) - \overline{P}_{l,C}(X^*)\right)^2
        \end{split}
\end{equation}
Therefore, we can conclude that for every $\gamma_2>0$, $\gamma_3 >0$ and $n$ sufficiently large,
\begin{equation}
\begin{split}
           \underset{p_l \in \mathcal{P}_{l}}{\min} \left[\mathbb{E}_{X^*} \textbf{1}_{X^* \in \mathcal{U}}\left( f^*(X^*) - p_l(X^*)\right)^2 \right] + \gamma_2+ \gamma_3 &\geq \mathbb{E}_{X^*} \textbf{1}_{X^* \in \mathcal{U}}\left( f^*(X^*) -\overline{P}_{l,C}(X^*)\right)^2  + \gamma_3 \\
       &\geq \mathbb{E}_{X^*} \left( f^*(X^*) -\overline{P}_{l,C}(X^*)\right)^2 
  \end{split}
\end{equation}
where we have used the fact that $C \geq \underset{d}{\max}~||f^*||_{\infty}$. Hence, we can conclude the proof when choosing $\gamma_1+\gamma_2+\gamma_3 \leq \gamma$. 
\end{proof}
