# Supplementary material for: How rotational invariance of common kernels prevents generalization in high dimensions
Source: arXiv:2104.04244 source file (2021-04-09)
Supplement: Supplementary file 16 [file Appendix_Section5.tex]

\section{Proofs Section \ref{sec:additionalresults}}

\begin{lemma}
The matrix $\begin{pmatrix} -D^{\alpha} & 1 \\ 1^T & 0 \end{pmatrix}^{-1}$ has $n-1$ positive and one negative Eigenvalue. Furthermore, $1^T D^{\alpha,-1} 1>0$ and therefore, we can write
\begin{equation}
    \hat{f}_{\textrm{fl}}(X^*) = Y^T \left[ -D^{\alpha,-1}+ \frac{D^{\alpha,-1} 1 1^T D^{\alpha,-1}}{1^T D^{\alpha,-1} 1}  \right] v^* +  \frac{Y^T D^{\alpha,-1} 1}{1^T D^{\alpha,-1} 1} 
\end{equation}
\end{lemma}

\begin{proof}
Let  $d_{\alpha}(X,Y) = ||X-Y||_2^{\alpha}$ with $\alpha \in (0,2)$. We already know from lemma \ref{lm:alphaexpbound} that the matrix $D^{\alpha}$ with entries $D^{\alpha}_{i,j} = d_{\alpha}(X_i,X_j)$ has $n-1$ positive Eigenvalues and one negative Eigenvalue. In particular, we have that $\underset{i \leq n}{\lambda} \left| \lambda_i(D^{\alpha}_{i,j}) \right| \geq c_{\lambda} >0$, where $c_{\lambda}$ is some positive constant independent of $n$. Next, note that because $D^{\alpha}$ has full rank, we can conclude from \cite[Theorem~3.1]{Ikramov00} that the matrix $\begin{pmatrix} -D^{\alpha} & 1 \\ 1^T & 0 \end{pmatrix}$ has $n$ positive Eigenvalues and one negative. Hence, the fact that
$$ \det(\begin{pmatrix} - D^{\alpha} & 1 \\ 1^T & 0 \end{pmatrix}) = \det(-D^{\alpha})(1^T D^{\alpha,-1} 1) \neq 0 $$
implies that $1^TD^{\alpha,-1}1 > 0$. As a result, we can use the Woodbury matrix identity to obtain the desired result. 
\end{proof}
Recall the definition of $\mathcal{U}$ given by
\begin{equation}
    \mathcal{U} = \left\{ X^* | \left|~||X^*||_2^2-1\right|  \leq n^-{\beta} \log(n)^{1+\epsilon}, ~ \max_{i} |X_i^T X^* |   \leq n^-{\beta} \log(n)^{1+\epsilon} \right\}.
\end{equation}
Furthermore, recall that we know from Corollary \ref{cr:testsample} that for any $\epsilon>0$, there exists $C >0$, such that for $n$ sufficiently large, $\mathcal{U}$ has measure $P(\mathcal{U}) \geq 1 - n^2 \exp(-C \log(n)^{1+\epsilon}) \to 1$. We can now show a very similar statement for to Theorem \ref{th:main}:

\begin{theorem}
\label{th:flatlimit}
Let $\alpha \in (0,2)$. Then, 
\begin{equation}
    \underset{X^* \in \mathcal{U}}{\max} ~ || \left[ -D^{\alpha,-1}+ \frac{D^{\alpha,-1} 1 1^T D^{\alpha,-1}}{1^T D^{\alpha,-1} 1} \right] \left(v^* - M^*\right) ||_1 \to 0 ~~~ a.s.
\end{equation} 
with
\begin{equation}
    \label{eq:Mstar} 
     M^* =\sum_{i=0}^p (\textbf{X}^TX^*)^{\circ i} \circ \left[
\sum_{m =0}^{p-i} \sum_{k = 0}^{m}  \frac{g_{i}^{(k,m-k)}(1,1)}{k!(m-k)!} \psi^{\circ k}\circ (\psi^*)^{\circ (m-k)} \right]
\end{equation}
and $p = \floor{2/\beta}$.
\end{theorem}
\begin{remark}
We highlight that it would also be possible to replace $\left[ -D^{\alpha,-1}+ \frac{D^{\alpha,-1} 1 1^T D^{\alpha,-1}}{1^T D^{\alpha,-1} 1} \right]$ with a matrix depending only on polynomials of $X_i^TX_j$ of order at most $p$. Similar as done in Theorem \ref{th:main}, where $K$ is replaced with $M$. 
\end{remark}
\begin{proof}[Proof of Theorem \ref{th:flatlimit}]
Define 
\begin{equation}
    B := -D^{\alpha,-1}+ \frac{D^{\alpha,-1} 1 1^T D^{\alpha,-1}}{1^T D^{\alpha,-1} 1}. 
\end{equation}
The proof can now be separated into two steps. In a first step, we show that $||B||_2 $ can be upper bounded by a constant independent of $n$, and in a second step, the concentration inequalities form Lemma \ref{lm:concentration} are used to conclude the proof. \\\\
\textbf{Step 1:} We already know from Lemma \ref{lm:alphaexp} that there exists some constant $c>0$ independent of $n$, such that $||D^{\alpha,-1}||_2 \leq c$. Thus, we only need to show that $||\frac{D^{\alpha,-1} 1 1^T D^{\alpha,-1}}{1^T D^{\alpha,-1} 1}||_2$. Because $\frac{D^{\alpha,-1} 1 1^T D^{\alpha,-1}}{1^T D^{\alpha,-1} 1}$ is a rank one matrix, we know that $$ ||\frac{D^{\alpha,-1} 1 1^T D^{\alpha,-1}}{1^T D^{\alpha,-1} 1}||_2 = \frac{ 1^TD^{\alpha,-2} 1}{1^T D^{\alpha,-1} 1}$$
Assume by contradiction that this quantity increases with $n$. In a first step, we show that this implies that $1^T D^{\alpha,-1} 1 \to 0$. Let $\lambda_1,...,\lambda_{n-1}$ be the $n-1$ negative Eigenvalues of $D^{\alpha,-1}$ and $\lambda_n$ be the only positive Eigenvalue. In particular, because $\trace(D^{\alpha}) = 0$, we know that $\lambda_n = -\sum_{i=1}^{n-1} \lambda_i$. Furthermore, let $v_i$ be the corresponding orthonormal Eigenvectors. Next, let $\alpha_i \in\mathbb{R}$ be such that $1 = \sum_{i = 1}^n \alpha_i v_i$. Since $||1||_2 = \sqrt{n}$, we know that $\alpha_i \leq \sqrt{n}$. Then, 
\begin{align*}
    1^T D^{\alpha,-1} 1 &= \alpha_n^2 \frac{1}{\lambda_n} - \sum_{i = 1}^{n-1} \alpha_i^2 \frac{1}{|\lambda_i|} >0 \\
    1^T D^{\alpha,-2} 1 &=  \alpha_n^2 \frac{1}{\lambda_n^2} + \sum_{i = 1}^{n-1} \alpha_i^2 \frac{1}{\lambda_i^2}
\end{align*}
As already shown in the proof of Lemma \ref{lm:alphaexpbound}, $\frac{1}{n^2} \sum_{i,j}^n D^{\alpha}_{i,j} \geq  2^{\alpha/2}~~a.s.$ and hence, we know that $\frac{1}{n} 1^T D^{\alpha}1^T \geq n ~~a.s.$. On the other hand, we can again see from Lemma \ref{lm:innerpr} that $||D^{\alpha}||_2 \leq ||D^{\alpha}||_F \leq n ~ \underset{i,j}{\max} |D^{\alpha}_{i,j}| \leq n  2^{\alpha/2} + O(n^{1-\beta/2}\log(n)^{1+\epsilon} ~ a.s.$. Therefore, there exists some constant $c>0$ independent of $n$, such that $\alpha_n^2 \frac{1}{\lambda_n} \leq c ~~ a.s$. As a consequence, 
\begin{equation}
    c \geq \alpha_n^2 \frac{1}{\lambda_n} \geq \sum_{i = 1}^{n-1} \alpha_i^2 \frac{1}{|\lambda_i|} \geq c_{\lambda}\sum_{i = 1}^{n-1} \alpha_i^2 \frac{1}{\lambda_i^2}
\end{equation} 
where we have used in the last inequality that $\lambda_i \leq c_{\lambda}$. Furthermore, we have that $ \alpha_n^2 \frac{1}{\lambda_n^2} \leq O(\frac{1}{n})$. Hence, we conclude that $ 1^T D^{\alpha,-2} 1 = O(1)$. Thus, we are only left to verify the case where $1^T D^{\alpha,-1} 1 \to 0$. Let $\gamma = 1^T D^{\alpha,-1} 1$ and $v = D^{\alpha,-1} 1$. Furthermore, let $\tilde{v} = \begin{pmatrix} -\gamma \\ 0 \\ ... \\0  \end{pmatrix}$. We know that $1^T(v +\tilde{v}) = 0$ and hence,
\begin{equation}
    (v + \tilde{v})^T D^{\alpha}  (v + \tilde{v}) \leq - c_{\lambda} (v + \tilde{v})^T (v + \tilde{v}) ~~a.s. 
\end{equation} 
Next, note that we already know from the above discussion that $v^Tv = O(1)$ and $\tilde{v}^T\tilde{v}= \gamma^2 \to 0 ~~a.s.$ by assumption. Therefore, $-c_{\lambda} (v + \tilde{v})^T (v + \tilde{v}) \leq \frac{c_{\lambda}}{2} v^Tv~~a.s.$. Hence, we get 
\begin{align*}
    v^T D^{\alpha}v + 2 \tilde{v}^T D^{\alpha}v + \tilde{v}^T D^{\alpha} \tilde{v} &\leq - \frac{c_{\lambda}}{2} v^Tv ~~a.s.\\ 
    1^T D^{\alpha,-1} 1 + 2 \tilde{v}^T 1 + \gamma^2 d_{\alpha}(X_1,X_1) &\leq - \frac{c_{\lambda}}{2} v^Tv ~~a.s.\\
     \gamma - 2 \gamma + &\leq - \frac{c_{\lambda}}{2} v^Tv ~~a.s. \\
     1&\geq \frac{c_{\lambda}}{2} \frac{v^Tv}{\gamma}~~a.s. \\
\end{align*} 
where we have used the fact that $\gamma$ is negative and $d_{\alpha}(X_n,X_n) = 0$. However, this implies that $||\frac{D^{\alpha,-1} 1 1^T D^{\alpha,-1}}{1^T D^{\alpha,-1} 1}||_2 = O(1) ~~ a.s.$\\\\
\textbf{Step 2:}
The only thing which is left to do is to show that $\sqrt{n} ||v^* - M^*||_2 \to 0$. The rest of the proof is then a straightforward modification of the proof of Theorem \ref{th:main}. \\
By the Binomial extension 
\begin{equation}
    d_{\alpha}(X_i,X^*) = \sum_{j=0}^{\infty} {j \choose \alpha/2} 2^{\alpha/2 }\left(\frac{1}{2} ||X_i - X^*||_2^2 - 1\right)^j, 
\end{equation}
we get that 
\begin{equation}
    \begin{split}
    v^*_i - M^*_i &=  d_{\alpha}(X_i,X^*) - \sum_{j=0}^{p} {j \choose \alpha/2}  {j \choose \alpha/2} 2^{\alpha/2 }\left(\frac{1}{2} ||X_i - X^*||_2^2 - 1\right)^j \\
    &= \sum_{j=p+1}^{\infty} {j \choose \alpha/2}  {j \choose \alpha/2} 2^{\alpha/2 }\left(\frac{1}{2} ||X_i - X^*||_2^2 - 1\right)^j
    \end{split}
\end{equation}
Hence, when applying Lemma \ref{lm:innerpr}, we get that
\begin{equation}
    \sqrt{n} ||v^* - M^*||_2 \leq n~ \underset{i}{\max} |v^*_i - M^*_i| \lesssim n \left(n^{-\beta/2} \log(n)^{1+\epsilon}\right)^{p+1} \to 0
\end{equation}
As a result, we can conclude the proof.
\end{proof}

\begin{proof}[Proof of Corollary \ref{cr:biasflatlimit}]
The proof of this Corollary follows line by line the proof of Corollary \ref{cr:biaslimit}. Hence, we can omit the proof. 
\end{proof}
