# Supplementary material for: How rotational invariance of common kernels prevents generalization in high dimensions
Source: arXiv:2104.04244 source file (2021-04-09)
Supplement: Supplementary file 17 [file Appendix_Sphere.tex]

\section{Spherical Input Data}
\label{sec:sphere}
\Comment{This section is not up to date!!}\\

A consequence of Lemma \ref{lm:innerpr} is that $|||X_i||_2^2 -1 | \to 0$, which shows that the data points concentrate around the $d(n)$-dimensional hyper sphere of radius one, $\mathcal{S}^{d}(1)$. This motivates us to also study the simpler case where the data points are projected on the hyper sphere, i.e. the input data set is set to $\textbf{S}$ with
$$ S_i = Z_i/||Z_i||_2$$
It turns out that any of the results presented in the main section of this paper easily adapt to this setting. This setting resembles the one studied in \cite{Ghorbani}. However, unlike  \cite{Ghorbani}, the data is clearly not uniformly distributed.
\\
The Schoenberg Theorem \cite{Schoenberg1988} is a well known fact stating that any positive definite continuous rotational symmetric kernel function $k(S,S'): \mathcal{S}^{d(n)}(1) \times \mathcal{S}^{d(n)}(1) \to \mathbb{R}$ has the form 
\begin{equation}
\label{eq:kernelsphere}
    k(S,S') = \sum_{j= 0}^{\infty} (S^TS')^{j} g_j
\end{equation}
with $g_j \in \mathbb{R}$. 
\begin{remark}
Say something about Schoenberg Theorem.
\end{remark}
Hence, in this section, we study kernels of the form of :..
Assume that $k_{\textrm{Sphere}}$ can be written in the form of Equation \ref{eq:kernelsphere} where we assume that $g_j$ are chosen such that the sum converges for any choices of $S^TS' \in [-1,1]$.
\
\begin{remark}
Note that $k_{\textrm{Sphere}}$ does not necessarily have to be positive definite. 
\end{remark}

Due to Lemma \ref{lm:innerpSphere}, we can straightforwardly extend any 
of the results from Section 3 to the case where $\textbf{S}$ is used as input data and $k_{\textrm{Sphere}}$ is used as kernel function. 
\begin{cor}
\label{prop:elkarouiextensionSphere}
Let $K$ be the matrix with entries $K_{i,j} = k_{\textrm{Sphere}}(S_i,S_j)$ and assume that Assumption \ref{ass:kernelsphere} holds true. Then,
$$ ||K- M||_2 \to 0 ~~~ a.s.$$ with
\begin{equation}
\label{eq:elkarouiM}
\begin{split}
    M &= \textbf{I}_n\left(g(1)  - \sum_{i =0}^p g_j \right) +  \sum_{i=0}^p g_j (\textbf{S}^T\textbf{S})^{\circ i} 
\end{split}
\end{equation}
where $\circ i$ denotes the $i$-times Hadamard product and $g^{(i)}$ is the $i$-th derivative of $g$.
\end{cor}
The Corollary is a consequence of the proof of Proposition \ref{prop:elkarouiextension} and Lemma \ref{lm:innerpSphere}. Note that we do no longer need the Lipschitz continuity assumption in Assumption \ref{ass:1} due to the fact that $S_i^TS_i = 1$. For the case where $\lambda = 0$, we need again some additional assumptions in order to guarantee that the minimum Eigenvalue of $K$ is asymptotically lower bounded. 
\begin{cor}
\label{cr:posdefsphere}
Assume that $n$ is sufficiently large. Then, if $g(1)  - \sum_{i =0}^p \frac{g^{(i)}(0)}{i!} >0$, the minimum Eigenvalues $\lambda_{min}(K)$ of $K$ is lower bounded by a positive non zero constant independent of $n$. 
\end{cor}
\begin{remark}
List kernels for which this is true.
\end{remark}

\begin{theorem}
\label{th:mainSphere}
Let $\lambda \in \mathbb{R}_{\geq 0}$ be the ridge parameter. Assume that $h$ from Equation \ref{eq:kernel} satisfies the assumption in Proposition \ref{prop:elkarouiextension}. Furthermore, assume that $(\lambda \textrm{I}_n + K)$ has almost surely non zero lower bounded Eigenvalues. Let $K^* = K(\textbf{S},S^*)$. Then, we have that 
$$||(\lambda \textrm{I}_n + K)^{-1}K^* - (\lambda \textrm{I}_n + M)^{-1}M^*||_2 \to 0 ~~~ a.s.$$
where $M$ is from Proposition \ref{prop:elkarouiextension} and 
$$ M^* =\sum_{i=0}^q g_j(\textbf{S}^TS^*)^{\circ i} $$
with $q = \floor{2/\beta}$.
\end{theorem}
