# Supplementary material for: How rotational invariance of common kernels prevents generalization in high dimensions
Source: arXiv:2104.04244 source file (2021-04-09)
Supplement: Supplementary file 18 [file Appendix_Technical_Preliminaries.tex]

\section{Technical Preliminaries}
\subsection{Concentration Inequalities}

\begin{remark}
The proofs from this section are closely following the ideas presented in \cite[Appendix~A]{el2010spectrum}
\end{remark}
\begin{lemma}[Concentration of quadratic forms of bounded R.V.]
\label{lm:concentration}
Suppose the vector $Z \in \mathbb{R}^d$, of some dimension $d \in \mathbb{N}_+$, is a random vector with i.i.d distributed bounded entries $|Z[i]| \leq c_Z $ of zero mean and unit variance. Let $M$ be any symmetric matrix with $||M||_2 = 1$. Let $M = M_+ - M_{-}$ be the decomposition of $M$ into two positive semi-definite matrix $M_+$ and $M_-$ with $||M_+||_2, ||M_-||_2 \leq 1$. Define
$$ \zeta = \frac{128 exp(4\pi) c_Z^2}{\trace(M_+)} $$
Then, for any $r/2 > \zeta$
\begin{equation*}
    \begin{split}
        &P(|z^T M z/\trace(M_+) - \trace(M)/\trace(M_+)| > r)  \\\leq &8 \exp(4\pi) [\exp(-\trace(M_+)(r/2 - \zeta)^2/(288c_z^2)) +  \exp(-\trace(M_+)/(288 c_z^2))]
    \end{split}
\end{equation*}
\end{lemma}
\begin{proof}
Note that we can decompose $M = M_+ - M_-$ in two positive semi definite matrix $M_+$ a $M_-$. Let $$f: \mathbb{R}^d \to \mathbb{R}, Z -> \sqrt{Z^T M_+ Z / \trace(M_+)} =\frac{1}{\sqrt{\trace(M_+)}}||M_+^{1/2} Z||_2 $$ We know that $f$ is a $\lambda_{\textrm{max}}(M_+)/\sqrt{\trace(M)}$-Lipschitz continuous and hence by assumption also a $1/\sqrt{\trace(M)}$-Lipschitz continuous. Using the simple fact that the norm is convex, we can apply \cite[Corollary~4.10]{Ledoux2001}. The rest is obtained by straight forward following line by line the proof of \cite[Lemma~A.2]{el2010spectrum}. We only highlight one intermediate step from the proof which will again be needed in this paper. For any $r>0$, one can show that
\begin{equation}
    \label{eq:concentration}
    P(|\sqrt{z^T M z/\trace(M_+)} - \sqrt{\trace(M)/\trace(M_+)}| > r) \leq 4 \exp(4 \pi) \exp(-\trace(M_+) r^2 /(32 c_z^2))
\end{equation}
\end{proof}

\begin{lemma}[Concentration of quadratic forms of Gaussian R.V.]
\label{lm:concentrationgaussian}
Suppose the vector $Z \in \mathbb{R}^d$, of some dimension $d \in \mathbb{N}_+$, is a random vector with i.i.d normal distributed entries of zero mean and unit variance. Let $M$ be any symmetric matrix with $||M||_2 = 1$. Let $M = M_+ - M_{-}$ be the decomposition of $M$ into two positive semi-definite matrix $M_+$ and $M_-$ with $||M_+||_2, ||M_-||_2 \leq 1$. Define
\begin{equation}
     \zeta = \frac{128 exp(4\pi)}{\trace(M_+)} 
\end{equation}
Then, for any $r/2 > \zeta$
\begin{equation*}
    \begin{split}
        &P(|z^T M z/\trace(M_+) - \trace(M)/\trace(M_+)| > r)  \\\leq & \exp(-\trace(M_+)(r/2 - \zeta)^2/(18)) +  \exp(-\trace(M_+)/(18))
    \end{split}
\end{equation*}
\end{lemma}
\begin{proof}
The proof is essentially the same as the proof of Lemma \ref{lm:concentration}. However, note that because $Z$ are normally distributed, we can directly apply \cite[Theorem~\rom{5}.\rom{1}]{Milman86}. As a consequence, we can replace Equation \ref{eq:concentration} with
\begin{equation}
   P(|\sqrt{z^T M z/\trace(M_+)} - \sqrt{\trace(M)/\trace(M_+)}| > r) \leq  \exp(-\trace(M_+)r^2/2)
\end{equation}
The proof follows then again from the proof of \cite[Lemma~A.2]{el2010spectrum}.

\end{proof}
As a consequence, let
\begin{cor}
\label{cr:simplebound}
Let $Z_i,Z_j$ be distributed as given in Equation \ref{eq:data}. Then, there exists generic constants $C_1,C_2,C_3 > 0$ such that for $\zeta = \frac{C_1}{\trace(\Sigma_n)}$, and any $r > \zeta$,
\begin{equation*}
    \begin{split}
    P(|Z_i^T Z_j/\trace(\Sigma_n) - \delta_{i,j}| > r)  \leq C_3[\exp(-C_2\trace(\Sigma_n)(r/2 - \zeta)^2) +  \exp(-C_2\trace(\Sigma_n)]
    \end{split}
\end{equation*}
\end{cor}
\begin{proof}
The case where $i = j$ is straight forward when applying \ref{lm:concentration} respectively \ref{lm:concentrationgaussian}. For the other case, note that we can choose $M = \begin{pmatrix} 0 & \Sigma_n \\ \Sigma_n & 0 \end{pmatrix}$ and $M_+ = \frac{1}{2}\begin{pmatrix} \Sigma_n & \Sigma_n \\ \Sigma_n & \Sigma_n \end{pmatrix}$,  $M_- =  \frac{1}{2}\begin{pmatrix}0 & \Sigma_n \\ \Sigma_n & 0  \end{pmatrix}$ and $z = (\tilde{Z}_i, \tilde{Z}_j)$ with $\tilde{Z}_i$,$\tilde{Z}_j$ from Equation \ref{eq:data}. The result then follows from $z^T M z = Z_i^T Z_j$ and $\trace(M) =0$, $\trace(M_+)= \trace(\Sigma_n)$. 
\end{proof}
We can now state the proof of Lemma \ref{lm:innerpr}. 
\begin{proof}[Proof of Lemma \ref{lm:innerpr}]
We make us of the Borell-Cantelli Lemma and Corollary \ref{cr:simplebound}. For any $\epsilon > 0$, let $r(n) = n^{-\beta/2} \log(n)^{1+\epsilon} $ and note that because $ \trace(\Sigma_n) \asymp n^{\beta}$, for any $n$ sufficiently large $r(n)/2 > \zeta \to 0$. In particular, we have that $\zeta$ decays at rate $n^{-\beta}$. Hence, making use of Corollary \ref{cr:simplebound}, we can see that there exists some generic constant $C>0$ such that for any $n$ sufficiently large
\begin{equation*}
    \begin{split}
        &P(|Z_i^T Z_j/\trace(\Sigma_n) - \delta_{i,j}| > r(n))  \\  \leq &8 \exp(4\pi) [\exp(-\trace(\Sigma_n)(r/2 - \zeta)^2/(288c_z^2)) +  \exp(-\trace(\Sigma_n)/(288 c_Z^2))] \\ &\leq \exp(-C \log(n)^{1+\epsilon} /(288c_z^2) 
    \end{split}
\end{equation*}
Using the union bound, we get
\begin{equation*}
    \begin{split}
        P(\max_{i,j} |Z_i^T Z_j/\trace(\Sigma_n) - \delta_{i,j}| > r(n)) \leq n^2 \exp(-C \log(n)^{1+\epsilon} /(288c_z^2) 
    \end{split}
\end{equation*}

And because $\epsilon>0$, for any $N \in \mathbb{N}_+$, we have that \begin{equation}
\sum_{n=N}^{\infty}  n^2 \exp(-C \log(n)^{1+\epsilon} /(288c_z^2) < \infty 
\end{equation}
which allows us to apply the Borel Cantelli Lemma, and hence,
\begin{equation}
\max_{i,j} \left|Z_i^T Z_j /\trace(\Sigma_d) - \delta_{i,j}\right| \leq
n^{-\beta/2} log(n)^{1+\epsilon} ~ ~~ a.s.
\end{equation}
which concludes the proof for the random variable $Z_i^T Z_j$. \\
For $\lvert\lvert Z_i - Z_j \rvert \rvert_2^2/\trace(\Sigma_d) $, we can write
\begin{equation}
    \lvert\lvert Z_i - Z_j \rvert \rvert_2^2/\trace(\Sigma_d) =  Z_i^TZ_i/\trace(\Sigma_d) + Z_j^TZ_j/\trace(\Sigma_d) -2 Z_i^TZ_j/\trace(\Sigma_d)
\end{equation}
Hence, the proof follows when taking the triangular inequality. Finally, it is not difficult to see that we can drop the multiplicative constant arising from the triangular inequality. 
\end{proof}
\subsection{Corollaries}
\begin{cor}
\label{cr:testsample}
For every $n$, let $X^*$ be a test sample drawn form the same distribution as the vectors of \textbf{X}. Then, for any $\epsilon > 0$ and $n$ sufficiently large, there exists some constant $C>0$ such that, with probability $\leq n \exp(-C log(n)^{1+\epsilon})$ over the draws of $X^*$, 
\label{lm:norm}
$$
\max_{i}\left| X_i^TX^*\right| \leq n^{-\beta/2}log(n)^{1+\epsilon} ~~~ a.s.
$$
and 
$$
\left| (X^*)^TX^* -1 \right| \leq  n^{-\beta/2}log(n)^{1+\epsilon} 
$$
In addition, Remark \ref{rm:astoinp} is still true.
\end{cor}
\begin{proof}
Denote with $\mathcal{E}_{\textbf{X}}$ the event where the concentration inequality from Lemma \ref{lm:innerpr} holds true and with $\mathcal{E}_{\textbf{X},X^*} \subset \mathcal{E}_{\textbf{X}} $ the event where also the concentration inequalities for $X^*$ from Corollary \ref{cr:testsample} hold true. We already know from the proof of Lemma \ref{lm:innerpr} that for $n$ sufficiently large, $P(\mathcal{E}_{\textbf{X}}) \geq 1-  n^2 \exp(-C \log(n)^{1+\epsilon})$. 
It is straight forward to verify that also $P(\mathcal{E}_{\textbf{X},X^*} \geq 1 -  (n+1)^2 \exp(-C \log(n)^{1+\epsilon})$. However, we can not yet conclude the proof. Let $\textbf{X} \in \mathcal{E}_{\textbf{X}}$. The issue is that we are actually interested in the probability $P(\mathcal{E}_{\textbf{X},X^*}| \textbf{X})$, which is not necessarily $\geq 1 - (n+1)^2 \exp(-C \log(n)^{1+\epsilon})$. Instead, we need to find a more restrictive event $\tilde{\mathcal{E}}_{\textbf{X}} \subset \mathcal{E}_{\textbf{X}}$ such that for every $\textbf{X}$,  $P(\mathcal{E}_{\textbf{X},X^*}| \textbf{X})  \geq 1 - (n+1)^2 \exp(-C \log(n)^{1+\epsilon})$ and simultaneously $\tilde{\mathcal{E}}_{\textbf{X}}$ holds true almost surely with respect to the sequence induced by $n$. Finally, in order to show that Remark \ref{rm:astoinp} still holds true, we need to show that for every $\epsilon >0$ there exists $\tilde{C}>0$ such that $\tilde{\mathcal{E}}_{\textbf{X}} \geq 1 - n^2 \exp(-\tilde{C} \log(n)^{1+\epsilon})$.\\ 
For every $q >0$, let $\overline{\mathcal{E}}_{\textbf{X},q}$ be the event where $\textbf{X} \in \mathcal{E}_{\textbf{X}}$ and $P(\mathcal{E}_{\textbf{X},X^*}| \textbf{X}) \geq 1- q$ and let $p$ be such that $1- p = P(\overline{\mathcal{E}}_{\textbf{X},q}$. We have that $$p \left(1-P(\overline{\mathcal{E}}_{\textbf{X},q}) \right) = p q \leq 1- P(\mathcal{E}_{\textbf{X},X^*}| \textbf{X})  \leq (n+1)^2 \exp(-C \log(n)^{1+\epsilon})  $$
The rest of the proof is then straight forward after observing that for $p=q$, $p \leq (n+1) \exp(-\frac{C}{2} \log(n)^{1+\epsilon})$.  
\end{proof}
\begin{cor}
\label{cr:concentrationh}
For any $\epsilon>0$ and any $k>0$, we have
$$ \underset{i}{\max}~ \left| \frac{(x_i^T x_i)^k}{\trace(\Sigma_d)^k} - 1 \right| \leq  c_k\max[n^{-\beta/2}log(n)^{1+\epsilon}, n^{-k\beta/2}log(n)^{k(1+\epsilon)}] ~~ a.s.$$
where $c_k$ is a constant only depending on $k$.
\end{cor}

\begin{proof}
By Lemma \ref{lm:concentration}, we have for every $k>0$
$$ \textrm{max}_{i}~ \left| \left[\frac{(x_i^T x_i)}{\trace(\Sigma_d)} - 1\right]^k \right| \leq ( n^{-\beta/2}log(n)^{1+\epsilon})^k$$
We proof the the claim by induction. The case where $k=1$ holds trivially with $c_k = 1$. For $k>1$, we have
\begin{equation*}
    \textrm{max}_{i}~  \left| \left[\frac{(x_i^T x_i)}{\trace(\Sigma_d)} - 1\right]^k \right| =  \textrm{max}_{i}~  \left| \frac{(x_i^T x_i)^k}{\trace(\Sigma_d)^k} + \sum_{j=1}^k (-1)^j {k \choose j }  \left(\frac{x_i^T x_i}{\trace(\Sigma_d)}\right)^{k-j}\right| \leq  (n^{-\beta/2}log(n)^{1+\epsilon})^k
\end{equation*} 
Note that we know by induction that $ \textrm{max}_{i}~ \left| \frac{(x_i^T x_i)^k}{\trace(\Sigma_d)^k} - 1 \right| \leq  c_k n^{-\beta/2}log(n)^{k(1+\epsilon)}$. Furthermore, we have $\sum_{j=1}^k(-1)^j {k\choose j} = -1$ which shows that

\begin{equation*}
  \textrm{max}_{i}~ \left| \frac{(x_i^T x_i)^k}{\trace(\Sigma_d)^k} + \sum_{j=1}^k (-1)^j {k \choose j } 1^{k-j} \right| \leq  (n^{-\beta/2}log(n)^{1+\epsilon})^k + \sum_{j=1}^{k-1} c_{k-j} (n^{-\beta/2}log(n)^{1+\epsilon})^{j-k}
\end{equation*} 
from which the claim follows. 
\end{proof}

\begin{cor}
\label{cr:exponentialbound}
For any $Z \in \mathbb{R}^{d(n)}$  generated from the same distribution as $Z_i$ from Equation \ref{eq:data}, we have that
$$
P(|\sqrt{Z_i^T Z_j}| > r) \leq \exp(-\trace(\Sigma) (r-1)^2 /(32 c_z^2))$$ 
\end{cor}
\begin{proof}
The proof follows straight forward from the proof of Lemma \ref{lm:concentration}. 
\end{proof}


\begin{lemma}
\label{lm:consistent}
Let $\hat{t}_n := \frac{1}{n} \sum_{i=1}^n X_i^T X_i $. For any $\epsilon >0$ and  $n$ sufficiently large, we have that for any $i \in \{1,...,n\}$,
$$|\frac{X_i^T X_i}{\hat{t}} - \frac{X_i^T X_i}{\trace(\Sigma_n)} | \leq  3  n^{-\beta/2}log(n)^{1+\epsilon} ~~a.s.$$
\end{lemma}
\begin{proof}
Due to Lemma \ref{lm:innerpr}, we get for any $\epsilon > 0$
$$ |\frac{\hat{t}}{\trace(\Sigma_n)} - 1| = |\frac{1}{n} \sum_{i =1}^n \frac{X_i^TX_i}{\trace(\Sigma_n)} - 1| \leq  n^{-\beta/2}log(n)^{1+\epsilon} ~~~ a.s
$$
and thus, 
\begin{equation}
\begin{split}
    |\frac{X_i^T X_i}{\hat{t}} - \frac{X_i^T X_i}{\trace(\Sigma_n)}) | &=  |\frac{X_i^T X_i (\trace(\Sigma_n)- \hat{t})}{\hat{t} \trace(\Sigma_n)} | = 
    |\frac{\frac{X_i^T X_i}{\trace(\Sigma_n)} (\frac{\hat{t}}{\trace(\Sigma_n)}-1)}{\frac{\hat{t}}{\trace(\Sigma_n)}} | \\
    &\leq \frac{(1+  n^{-\beta/2}log(n)^{1+\epsilon})  n^{-\beta/2}log(n)^{1+\epsilon}}{1-  n^{-\beta/2}log(n)^{1+\epsilon}} ~~~ a.s.\\
    &\leq 3  n^{-\beta/2}log(n)^{1+\epsilon} ~~~ a.s.
\end{split}
\end{equation}
where we choose $n$  sufficiently large such that $ n^{-\beta/2}log(n)^{1+\epsilon} \leq 0.5$
\end{proof}


\subsection{Concentration Inequalities for the Spherical Case}

\begin{cor}
\label{lm:innerpSphere}
For any $\epsilon > 0$, we have that asymptotically
\label{lm:norm}
$$
\max_{i,j }\left| \left(\frac{Z_i}{||Z_i||_2}  \right)^T \frac{Z_j}{||Z_j||_2} - \delta_{i, j}\right| \leq 2 n^{-\beta/2}log(n)^{1+\epsilon} ~~~ a.s.
$$
\end{cor}
\begin{proof}
The case where $i = j$ holds trivially true. Let $S_i = \frac{Z_i}{||Z_i||_2}$ and $X_i = \frac{Z_i}{\trace(\Sigma_n)}$. Since we are in the Euclidean space, the inner product is given by
$$ (S_i^TS_j)^2 = \cos(\alpha)^2 $$
and 
$$ (X_i^TX_j)^2 = \cos(\alpha)^2 ||X_i||_2^2 ||X_j||_2^2 $$
with $\alpha \in [0, 2\pi]$. Let $b(n) := n^{-\beta/2} log(n)^{1+\epsilon}$, then by Lemma \ref{lm:innerpr} we have that $|~ ||X_i||_2^2 -1 | \leq l(n)  ~ a.s.$ and therefore,
\begin{equation*}
    \begin{split}
        \cos(\alpha)^2 &\leq \cos(\alpha)^2 \left( (||X_i||_2^2 + l(n)) (||X_j||_2^2+l(n)) \right)  ~~~ a.s.\\
        &=  \cos(\alpha)^2 \left( (||X_i||_2^2||X_j||_2^2 + l(n) ||X_i||_2^2 + l(n) ||X_j||_2^2  + l(n)^2 \right) ~~~ a.s.
    \end{split}
\end{equation*}  
using again Lemma \ref{lm:innerpr}, we have that $  |\cos(\alpha)^2 ||X_i||_2^2||X_j||_2^2 | \leq l(n)^2 ~a.s. $. Hence,
\begin{equation*}
    \begin{split}
         \cos(\alpha)^2\left(1- l(n) ||X_i||_2^2 - l(n) ||X_j||_2^2  - l(n)^2 \right) &\leq \cos(\alpha)^2 \left( (||X_i||_2^2 + l(n)) (||X_j||_2^2+l(n)) \right)  ~~~ a.s.\\
      \cos(\alpha)^2\left(1- 2 l(n) (1+l(n)) - l(n)^2 \right) &\leq l(n)^2 ~~~ a.s.\\
    \end{split}
\end{equation*}
Finally, since $l(n) \to 0$, for $n$ large enough, $\left(1- 2 l(n) (1+l(n)) - l(n)^2 \right) \geq 1/4$ which concludes the proof. 
\end{proof}
