# Supplementary material for: How rotational invariance of common kernels prevents generalization in high dimensions
Source: arXiv:2104.04244 source file (2021-04-09)
Supplement: Supplementary file 19 [file tmp_stuff.tex]

\begin{prop}
\label{prop:Evlowerbound}
Assume that Assumption A.1-A.5 hold true. In addition, assume that that for any $j$, $g_j$ is a positive definite kernel function. Then, we have that for any $\gamma >0$, 
\begin{equation}
\label{eq:lambdamin}
    \lambda_{min}(K) \geq k(e_1,e_1) - \sum_{j = 1}^{\floor{2/\beta}} g_j(1,1) - \gamma ~~~a.s.
\end{equation}
with $e_1 = (1,0, \cdots,0)$. 
Furthermore, under the assumption that the definition of $g$ can be extended such that $k(e_1,e_1) = \sum_{i=0}^{\infty} g_j(1,1)$ holds true, we can see that the Eigenvalues of $K$ are lower bounded by a positive non zero constant if there exists $j > \floor{2/\beta}$ such that $g_j(1,1) > 0$. 
\end{prop}



We can now show various examples for which Corollary ~\ref{prop:Evlowerbound} holds true. For instance, any inner product kernel of the form $k(\xk,\xkd) = \sum_{j=0}^{\infty} h_j ~ (\xk^T\xkd)^j$ with $h_j \geq 0$ and given that there exists $\hat{j} \geq \floor{2/\beta}$ such that $h_{\hat{j}}>0$ satisfies the assumption in Corollary ~\ref{prop:Evlowerbound}. Another example are the NTK kernels of any depth. We refer to Proposition ~\ref{prop:ntkass} for a proof. Unfortunately, it is unclear whether general RBF kernel satisfy the additional assumptions in Corollary ~\ref{prop:Evlowerbound}. However, we can show that it holds true for the special case when $k(\xk, \xkd) = \exp(-\tau_0 \lvert\lvert \xk - \xkd \rvert\rvert_2^2)$ is the Guassian kernel, which follows immediately from $\exp(-\lvert\lvert \xk - \xkd \rvert\rvert_2^2) =\sum_{j=0}^{\infty} \frac{2}{j!}(\xk^T\xkd)^j \exp(-\lvert\lvert \xk \rvert\rvert_2^2)\exp(-\lvert\lvert \xkd \rvert\rvert_2^2) $. Furthermore, using a different proof technique, Proposition ~\ref{prop:alphaexp} from the appendix shows that the Eigenvalues of $K$ can also be lower bounded away from zero when $k$ is the $\alpha$-exponential kernel with $k(\xk, \xkd) = \exp(-\tau_0 \lvert\lvert \xk - \xkd \rvert\rvert_2^{\alpha})$ and $\alpha \in (0,2)$. \newline
Finally, we remark that the phenomenon of lower bounded Eigenvalues is a consequence of the high dimensionality of the input data. In contrast, in classical regimes where the dimension $d$ is constant there exists many results connecting the decay of the Eigenvalues of the kernel matrix $K$ with the Eigenvalue decay of the operator $\mathcal{T}: L^2_{\mu}(\mathcal{X}) \to L^2_{\mu}(\mathcal{X}), g \to \int_{\mathcal{X}} k(x,y) g(y) d\mu $. For instance, we refer to \cite[Theorem~2]{Belkin18} for a statement of this type. 
We can now discuss the implications of Theorem ~\ref{th:main_text} for various kernels. First of all, we note that whenever $\lambda$ dos not go to zero, based on the previous discussion, the Theorem ~\ref{th:main_text} applies for a very broad range of kernels. For the more interesting case where $\lambda = 0$ or $\lambda \to 0$, we shown in the above discussion several important examples for which Theorem ~\ref{th:main} still holds true.
